# Supplementary material for: SNR-calibrated Type Ia supernova models
Source: arXiv:1810.13123 ancillary file (2018-12-12)
Supplement: Supplementary file 1 [file fulltables.pdf]

# SNR-calibrated Type Ia supernova models

Bravo, Badenes & Martínez-Rodríguez

Monthly Notices of the Royal Astronomical Society, 2018, submitted

Online tables

**LIST OF TABLES**

Table 3. Nucleosynthesis in Chandrasekhar-mass DDT models with  $\xi_{\text{CO}} = 0.9$ .

Table 4. Nucleosynthesis in sub-Chandrasekhar models with  $\xi_{\text{CO}} = 0.9$ .

Table 5. Radioactivities with half-life longer than one day in Chandrasekhar-mass DDT models with  $\xi_{\text{CO}} = 0.9$ .

Table 6. Radioactivities with half-life longer than one day in sub-Chandrasekhar models with  $\xi_{\text{CO}} = 0.9$ .

Table A1. Nucleosynthesis in Chandrasekhar-mass DDT models with the standard  $^{12}\text{C}+^{16}\text{O}$  reaction rate.

Table A2. Nucleosynthesis in sub-Chandrasekhar models with the standard  $^{12}\text{C}+^{16}\text{O}$  reaction rate.

Table A3. Radioactivities with half-life longer than one day in Chandrasekhar-mass DDT models with the standard  $^{12}\text{C}+^{16}\text{O}$  reaction rate.

Table A4. Radioactivities with half-life longer than one day in sub-Chandrasekhar models with the standard  $^{12}\text{C}+^{16}\text{O}$  reaction rate.

*An ascii version of the tables is available online.*

Table 3. Nucleosynthesis in Chandrasekhar-mass DDT models with  $\xi_{\text{CO}} = 0.9$ .

| $\rho_{\text{DDT}}$ |          | 1.2E+07  | 1.2E+07  | 1.2E+07  | 1.2E+07  | 1.2E+07  | 1.6E+07  | 1.6E+07  | 1.6E+07  | 1.6E+07  | 1.6E+07  |
|---------------------|----------|----------|----------|----------|----------|----------|----------|----------|----------|----------|----------|
| Z                   |          | 2.25E-4  | 2.25E-3  | 9.00E-3  | 2.25E-2  | 6.75E-2  | 2.25E-4  | 2.25E-3  | 9.00E-3  | 2.25E-2  | 6.75E-2  |
| elem                | 2 He     | 3.01E-04 | 2.87E-04 | 2.57E-04 | 1.61E-04 | 9.74E-06 | 3.08E-04 | 2.93E-04 | 2.62E-04 | 1.63E-04 | 9.43E-06 |
| isot                | 2 He 3   | 1.58E-12 | 1.56E-12 | 1.54E-12 | 1.42E-12 | 1.16E-12 | 1.58E-12 | 1.56E-12 | 1.54E-12 | 1.42E-12 | 1.16E-12 |
| isot                | 2 He 4   | 3.01E-04 | 2.87E-04 | 2.57E-04 | 1.61E-04 | 9.74E-06 | 3.07E-04 | 2.93E-04 | 2.62E-04 | 1.63E-04 | 9.43E-06 |
| elem                | 6 C      | 4.94E-03 | 4.98E-03 | 4.90E-03 | 5.06E-03 | 5.21E-03 | 2.50E-03 | 2.47E-03 | 2.54E-03 | 2.64E-03 | 2.51E-03 |
| isot                | 6 C 12   | 4.94E-03 | 4.98E-03 | 4.90E-03 | 5.05E-03 | 5.21E-03 | 2.50E-03 | 2.47E-03 | 2.54E-03 | 2.64E-03 | 2.51E-03 |
| isot                | 6 C 13   | 1.94E-10 | 3.57E-09 | 1.26E-08 | 2.95E-08 | 7.43E-08 | 1.04E-10 | 1.64E-09 | 6.37E-09 | 1.57E-08 | 3.94E-08 |
| elem                | 7 N      | 1.76E-05 | 1.38E-05 | 9.73E-06 | 6.92E-06 | 5.37E-06 | 1.56E-05 | 1.21E-05 | 8.32E-06 | 5.21E-06 | 2.48E-06 |
| isot                | 7 N 14   | 1.75E-05 | 1.38E-05 | 9.72E-06 | 6.91E-06 | 5.37E-06 | 1.55E-05 | 1.21E-05 | 8.32E-06 | 5.21E-06 | 2.48E-06 |
| isot                | 7 N 15   | 1.59E-07 | 4.81E-09 | 2.61E-09 | 3.93E-09 | 7.26E-09 | 8.44E-08 | 2.50E-09 | 1.33E-09 | 1.77E-09 | 2.76E-09 |
| elem                | 8 O      | 1.71E-01 | 1.74E-01 | 1.75E-01 | 1.82E-01 | 1.86E-01 | 1.12E-01 | 1.13E-01 | 1.19E-01 | 1.24E-01 | 1.21E-01 |
| isot                | 8 O 16   | 1.71E-01 | 1.74E-01 | 1.75E-01 | 1.82E-01 | 1.86E-01 | 1.12E-01 | 1.13E-01 | 1.19E-01 | 1.24E-01 | 1.21E-01 |
| isot                | 8 O 17   | 8.50E-09 | 1.17E-07 | 2.64E-07 | 4.15E-07 | 5.87E-07 | 4.40E-09 | 5.04E-08 | 1.16E-07 | 1.78E-07 | 2.13E-07 |
| isot                | 8 O 18   | 2.46E-09 | 1.90E-09 | 2.15E-09 | 2.97E-09 | 3.97E-09 | 1.14E-09 | 8.14E-10 | 9.46E-10 | 1.21E-09 | 1.33E-09 |
| elem                | 9 F      | 5.43E-11 | 1.42E-11 | 1.47E-11 | 3.74E-11 | 1.41E-10 | 2.28E-11 | 5.36E-12 | 6.02E-12 | 1.66E-11 | 6.28E-11 |
| isot                | 9 F 19   | 5.43E-11 | 1.42E-11 | 1.47E-11 | 3.74E-11 | 1.41E-10 | 2.28E-11 | 5.36E-12 | 6.02E-12 | 1.66E-11 | 6.28E-11 |
| elem                | 10 Ne    | 3.95E-03 | 3.96E-03 | 3.88E-03 | 4.04E-03 | 4.31E-03 | 1.80E-03 | 1.77E-03 | 1.83E-03 | 1.93E-03 | 1.89E-03 |
| isot                | 10 Ne 20 | 3.95E-03 | 3.96E-03 | 3.86E-03 | 3.99E-03 | 4.07E-03 | 1.80E-03 | 1.77E-03 | 1.82E-03 | 1.91E-03 | 1.77E-03 |
| isot                | 10 Ne 21 | 8.91E-09 | 5.27E-08 | 1.50E-07 | 3.83E-07 | 1.67E-06 | 4.56E-09 | 2.39E-08 | 7.08E-08 | 1.84E-07 | 7.51E-07 |
| isot                | 10 Ne 22 | 1.40E-07 | 2.03E-06 | 1.23E-05 | 4.57E-05 | 2.39E-04 | 9.49E-08 | 1.13E-06 | 6.61E-06 | 2.40E-05 | 1.16E-04 |
| elem                | 11 Na    | 2.56E-05 | 2.77E-05 | 3.40E-05 | 5.25E-05 | 1.27E-04 | 1.23E-05 | 1.27E-05 | 1.65E-05 | 2.58E-05 | 5.76E-05 |
| isot                | 11 Na 23 | 2.56E-05 | 2.77E-05 | 3.40E-05 | 5.25E-05 | 1.27E-04 | 1.23E-05 | 1.27E-05 | 1.65E-05 | 2.58E-05 | 5.76E-05 |
| elem                | 12 Mg    | 3.93E-02 | 3.52E-02 | 2.64E-02 | 1.92E-02 | 1.10E-02 | 2.26E-02 | 2.01E-02 | 1.55E-02 | 1.13E-02 | 5.99E-03 |
| isot                | 12 Mg 24 | 3.93E-02 | 3.52E-02 | 2.63E-02 | 1.90E-02 | 1.02E-02 | 2.26E-02 | 2.01E-02 | 1.55E-02 | 1.12E-02 | 5.66E-03 |
| isot                | 12 Mg 25 | 1.08E-06 | 1.03E-05 | 2.83E-05 | 7.67E-05 | 2.62E-04 | 5.64E-07 | 5.22E-06 | 1.43E-05 | 3.80E-05 | 1.16E-04 |
| isot                | 12 Mg 26 | 1.28E-06 | 9.06E-06 | 4.03E-05 | 1.14E-04 | 4.64E-04 | 6.15E-07 | 4.31E-06 | 2.03E-05 | 5.76E-05 | 2.11E-04 |
| elem                | 13 Al    | 1.09E-04 | 3.72E-04 | 6.91E-04 | 8.47E-04 | 8.43E-04 | 5.64E-05 | 2.03E-04 | 3.89E-04 | 4.77E-04 | 4.28E-04 |
| isot                | 13 Al 27 | 1.09E-04 | 3.72E-04 | 6.91E-04 | 8.47E-04 | 8.43E-04 | 5.64E-05 | 2.03E-04 | 3.89E-04 | 4.77E-04 | 4.28E-04 |
| elem                | 14 Si    | 3.68E-01 | 3.82E-01 | 3.84E-01 | 3.93E-01 | 3.87E-01 | 2.86E-01 | 2.94E-01 | 3.05E-01 | 3.11E-01 | 2.99E-01 |
| isot                | 14 Si 28 | 3.68E-01 | 3.82E-01 | 3.83E-01 | 3.89E-01 | 3.76E-01 | 2.86E-01 | 2.93E-01 | 3.04E-01 | 3.08E-01 | 2.93E-01 |
| isot                | 14 Si 29 | 1.53E-04 | 4.19E-04 | 6.39E-04 | 1.10E-03 | 2.78E-03 | 9.91E-05 | 2.66E-04 | 4.15E-04 | 6.93E-04 | 1.57E-03 |
| isot                | 14 Si 30 | 2.03E-05 | 1.78E-04 | 1.02E-03 | 2.65E-03 | 8.82E-03 | 1.24E-05 | 1.09E-04 | 6.31E-04 | 1.64E-03 | 5.25E-03 |
| elem                | 15 P     | 5.50E-05 | 1.24E-04 | 3.50E-04 | 6.82E-04 | 1.53E-03 | 4.19E-05 | 8.16E-05 | 2.26E-04 | 4.34E-04 | 9.15E-04 |
| isot                | 15 P 31  | 5.50E-05 | 1.24E-04 | 3.50E-04 | 6.82E-04 | 1.53E-03 | 4.19E-05 | 8.16E-05 | 2.26E-04 | 4.34E-04 | 9.15E-04 |
| elem                | 16 S     | 2.30E-01 | 2.31E-01 | 2.34E-01 | 2.37E-01 | 2.10E-01 | 1.94E-01 | 1.94E-01 | 1.98E-01 | 1.98E-01 | 1.70E-01 |
| isot                | 16 S 32  | 2.30E-01 | 2.31E-01 | 2.32E-01 | 2.32E-01 | 1.95E-01 | 1.94E-01 | 1.93E-01 | 1.97E-01 | 1.95E-01 | 1.59E-01 |
| isot                | 16 S 33  | 7.81E-05 | 1.47E-04 | 2.91E-04 | 4.36E-04 | 6.36E-04 | 4.91E-05 | 9.51E-05 | 1.93E-04 | 2.93E-04 | 4.30E-04 |
| isot                | 16 S 34  | 8.21E-07 | 2.95E-04 | 1.68E-03 | 4.72E-03 | 1.50E-02 | 8.99E-07 | 2.03E-04 | 1.18E-03 | 3.30E-03 | 1.02E-02 |
| isot                | 16 S 36  | 1.33E-10 | 6.43E-09 | 7.80E-08 | 5.31E-07 | 1.71E-05 | 1.14E-10 | 3.53E-09 | 4.20E-08 | 3.00E-07 | 9.24E-06 |
| elem                | 17 Cl    | 1.47E-05 | 3.81E-05 | 1.20E-04 | 2.60E-04 | 4.65E-04 | 1.25E-05 | 2.72E-05 | 8.24E-05 | 1.75E-04 | 3.13E-04 |
| isot                | 17 Cl 35 | 8.20E-06 | 2.62E-05 | 9.49E-05 | 2.18E-04 | 3.91E-04 | 7.95E-06 | 1.85E-05 | 6.43E-05 | 1.45E-04 | 2.60E-04 |
| isot                | 17 Cl 37 | 6.52E-06 | 1.18E-05 | 2.51E-05 | 4.16E-05 | 7.42E-05 | 4.55E-06 | 8.76E-06 | 1.80E-05 | 2.96E-05 | 5.25E-05 |
| elem                | 18 Ar    | 5.71E-02 | 5.48E-02 | 5.28E-02 | 5.10E-02 | 4.23E-02 | 5.10E-02 | 4.92E-02 | 4.79E-02 | 4.56E-02 | 3.65E-02 |
| isot                | 18 Ar 36 | 5.71E-02 | 5.47E-02 | 5.21E-02 | 4.86E-02 | 3.51E-02 | 5.10E-02 | 4.92E-02 | 4.74E-02 | 4.40E-02 | 3.16E-02 |
| isot                | 18 Ar 38 | 5.32E-07 | 1.15E-04 | 7.90E-04 | 2.37E-03 | 7.23E-03 | 3.24E-07 | 7.58E-05 | 5.27E-04 | 1.61E-03 | 4.95E-03 |
| isot                | 18 Ar 40 | 3.05E-11 | 1.59E-09 | 2.13E-08 | 1.13E-07 | 1.38E-06 | 1.89E-11 | 7.26E-10 | 9.93E-09 | 5.40E-08 | 6.60E-07 |
| elem                | 19 K     | 3.97E-06 | 2.29E-05 | 8.07E-05 | 1.61E-04 | 2.68E-04 | 3.93E-06 | 1.71E-05 | 5.77E-05 | 1.14E-04 | 1.95E-04 |
| isot                | 19 K 39  | 2.99E-06 | 2.07E-05 | 7.51E-05 | 1.52E-04 | 2.54E-04 | 3.06E-06 | 1.53E-05 | 5.35E-05 | 1.07E-04 | 1.84E-04 |
| isot                | 19 K 40  | 7.19E-11 | 3.33E-09 | 2.62E-08 | 1.57E-07 | 5.21E-07 | 4.63E-11 | 2.09E-09 | 1.66E-08 | 9.93E-08 | 3.07E-07 |
| isot                | 19 K 41  | 9.76E-07 | 2.19E-06 | 5.53E-06 | 9.53E-06 | 1.39E-05 | 8.78E-07 | 1.77E-06 | 4.19E-06 | 6.96E-06 | 1.02E-05 |
| elem                | 20 Ca    | 6.44E-02 | 5.88E-02 | 5.32E-02 | 4.67E-02 | 3.08E-02 | 6.08E-02 | 5.67E-02 | 5.20E-02 | 4.61E-02 | 3.14E-02 |
| isot                | 20 Ca 40 | 6.44E-02 | 5.88E-02 | 5.31E-02 | 4.66E-02 | 3.06E-02 | 6.07E-02 | 5.67E-02 | 5.20E-02 | 4.61E-02 | 3.12E-02 |
| isot                | 20 Ca 42 | 7.94E-09 | 2.39E-06 | 2.04E-05 | 6.72E-05 | 2.03E-04 | 4.74E-09 | 1.66E-06 | 1.40E-05 | 4.56E-05 | 1.39E-04 |
| isot                | 20 Ca 43 | 1.59E-09 | 5.55E-09 | 4.36E-08 | 2.07E-07 | 1.09E-06 | 1.19E-09 | 3.40E-09 | 2.65E-08 | 1.26E-07 | 6.19E-07 |
| isot                | 20 Ca 44 | 4.31E-05 | 3.69E-05 | 3.14E-05 | 2.59E-05 | 1.85E-05 | 4.42E-05 | 3.96E-05 | 3.45E-05 | 2.94E-05 | 2.13E-05 |
| isot                | 20 Ca 46 | 5.09E-09 | 5.97E-09 | 1.61E-08 | 6.79E-08 | 8.61E-07 | 4.91E-09 | 5.34E-09 | 1.03E-08 | 3.52E-08 | 3.98E-07 |
| isot                | 20 Ca 48 | 1.89E-07 | 1.96E-07 | 2.26E-07 | 3.02E-07 | 7.97E-07 | 1.82E-07 | 1.89E-07 | 2.23E-07 | 2.84E-07 | 6.70E-07 |
| elem                | 21 Sc    | 1.70E-07 | 2.20E-07 | 4.00E-07 | 7.25E-07 | 1.98E-06 | 1.49E-07 | 2.04E-07 | 3.41E-07 | 5.50E-07 | 1.22E-06 |
| isot                | 21 Sc 45 | 1.70E-07 | 2.20E-07 | 4.00E-07 | 7.25E-07 | 1.98E-06 | 1.49E-07 | 2.04E-07 | 3.41E-07 | 5.50E-07 | 1.22E-06 |

Rows starting by 'elem' give the elemental yields of each model, in solar masses, where the element is identified by the atomic number and symbol. Rows starting by 'isot' give the yields of each isotope, in solar masses. In this case, the isotope is identified by the atomic number and symbol, and by the baryon number.

Table 3 *continued.*

| $\rho_{\text{DDT}}$ |          | 1.2E+07  | 1.2E+07  | 1.2E+07  | 1.2E+07  | 1.2E+07  | 1.6E+07  | 1.6E+07  | 1.6E+07  | 1.6E+07  | 1.6E+07  |
|---------------------|----------|----------|----------|----------|----------|----------|----------|----------|----------|----------|----------|
| Z                   |          | 2.25E-4  | 2.25E-3  | 9.00E-3  | 2.25E-2  | 6.75E-2  | 2.25E-4  | 2.25E-3  | 9.00E-3  | 2.25E-2  | 6.75E-2  |
| elem                | 22 Ti    | 9.69E-04 | 9.45E-04 | 9.33E-04 | 9.19E-04 | 9.90E-04 | 1.11E-03 | 1.10E-03 | 1.08E-03 | 1.06E-03 | 1.10E-03 |
| isot                | 22 Ti 46 | 7.83E-08 | 2.11E-06 | 1.58E-05 | 4.43E-05 | 1.02E-04 | 7.40E-08 | 1.65E-06 | 1.13E-05 | 3.07E-05 | 7.33E-05 |
| isot                | 22 Ti 47 | 3.30E-08 | 2.10E-08 | 2.23E-07 | 1.07E-06 | 5.13E-06 | 3.45E-08 | 1.64E-08 | 1.45E-07 | 6.79E-07 | 3.19E-06 |
| isot                | 22 Ti 48 | 5.33E-04 | 4.98E-04 | 4.44E-04 | 3.53E-04 | 2.10E-04 | 6.81E-04 | 6.54E-04 | 5.89E-04 | 5.04E-04 | 3.43E-04 |
| isot                | 22 Ti 49 | 1.05E-05 | 1.41E-05 | 2.20E-05 | 2.94E-05 | 3.45E-05 | 8.85E-06 | 1.59E-05 | 2.48E-05 | 3.43E-05 | 4.30E-05 |
| isot                | 22 Ti 50 | 4.26E-04 | 4.32E-04 | 4.51E-04 | 4.91E-04 | 6.39E-04 | 4.23E-04 | 4.29E-04 | 4.50E-04 | 4.89E-04 | 6.34E-04 |
| elem                | 23 V     | 6.42E-05 | 7.47E-05 | 1.06E-04 | 1.45E-04 | 2.12E-04 | 6.53E-05 | 7.74E-05 | 1.15E-04 | 1.61E-04 | 2.39E-04 |
| isot                | 23 V 50  | 1.63E-08 | 1.69E-08 | 2.95E-08 | 1.46E-07 | 5.79E-07 | 1.60E-08 | 1.63E-08 | 2.31E-08 | 8.44E-08 | 3.29E-07 |
| isot                | 23 V 51  | 6.41E-05 | 7.46E-05 | 1.06E-04 | 1.45E-04 | 2.11E-04 | 6.53E-05 | 7.74E-05 | 1.15E-04 | 1.61E-04 | 2.39E-04 |
| elem                | 24 Cr    | 1.57E-02 | 1.53E-02 | 1.50E-02 | 1.41E-02 | 1.42E-02 | 2.12E-02 | 2.11E-02 | 2.02E-02 | 1.94E-02 | 1.91E-02 |
| isot                | 24 Cr 50 | 3.47E-05 | 6.58E-05 | 1.71E-04 | 4.19E-04 | 1.50E-03 | 4.02E-05 | 6.71E-05 | 1.66E-04 | 4.02E-04 | 1.41E-03 |
| isot                | 24 Cr 52 | 1.24E-02 | 1.18E-02 | 1.11E-02 | 9.47E-03 | 7.61E-03 | 1.79E-02 | 1.74E-02 | 1.60E-02 | 1.44E-02 | 1.20E-02 |
| isot                | 24 Cr 53 | 6.27E-04 | 7.45E-04 | 1.02E-03 | 1.25E-03 | 1.49E-03 | 6.90E-04 | 8.98E-04 | 1.25E-03 | 1.63E-03 | 2.14E-03 |
| isot                | 24 Cr 54 | 2.62E-03 | 2.65E-03 | 2.75E-03 | 2.94E-03 | 3.58E-03 | 2.62E-03 | 2.65E-03 | 2.75E-03 | 2.94E-03 | 3.58E-03 |
| elem                | 25 Mn    | 3.73E-03 | 5.11E-03 | 7.13E-03 | 9.14E-03 | 1.21E-02 | 3.98E-03 | 5.93E-03 | 8.76E-03 | 1.19E-02 | 1.76E-02 |
| isot                | 25 Mn 55 | 3.73E-03 | 5.11E-03 | 7.13E-03 | 9.14E-03 | 1.21E-02 | 3.98E-03 | 5.93E-03 | 8.76E-03 | 1.19E-02 | 1.76E-02 |
| elem                | 26 Fe    | 3.89E-01 | 3.79E-01 | 3.84E-01 | 3.69E-01 | 4.00E-01 | 5.90E-01 | 5.87E-01 | 5.70E-01 | 5.59E-01 | 5.96E-01 |
| isot                | 26 Fe 54 | 3.24E-02 | 3.58E-02 | 4.85E-02 | 7.50E-02 | 1.60E-01 | 3.22E-02 | 3.58E-02 | 4.99E-02 | 7.93E-02 | 1.76E-01 |
| isot                | 26 Fe 56 | 3.45E-01 | 3.32E-01 | 3.23E-01 | 2.81E-01 | 2.23E-01 | 5.46E-01 | 5.39E-01 | 5.06E-01 | 4.64E-01 | 4.00E-01 |
| isot                | 26 Fe 57 | 4.47E-03 | 4.90E-03 | 5.89E-03 | 6.85E-03 | 8.10E-03 | 5.04E-03 | 5.61E-03 | 6.97E-03 | 8.59E-03 | 1.14E-02 |
| isot                | 26 Fe 58 | 6.41E-03 | 6.46E-03 | 6.65E-03 | 7.04E-03 | 8.28E-03 | 6.42E-03 | 6.47E-03 | 6.66E-03 | 7.04E-03 | 8.26E-03 |
| elem                | 27 Co    | 3.97E-04 | 3.84E-04 | 3.99E-04 | 4.07E-04 | 4.63E-04 | 4.20E-04 | 4.05E-04 | 4.19E-04 | 4.32E-04 | 4.77E-04 |
| isot                | 27 Co 59 | 3.97E-04 | 3.84E-04 | 3.99E-04 | 4.07E-04 | 4.63E-04 | 4.20E-04 | 4.05E-04 | 4.19E-04 | 4.32E-04 | 4.77E-04 |
| elem                | 28 Ni    | 2.85E-02 | 2.91E-02 | 3.15E-02 | 3.62E-02 | 5.07E-02 | 2.83E-02 | 2.90E-02 | 3.16E-02 | 3.69E-02 | 5.39E-02 |
| isot                | 28 Ni 58 | 2.20E-02 | 2.25E-02 | 2.47E-02 | 2.92E-02 | 4.20E-02 | 2.19E-02 | 2.25E-02 | 2.49E-02 | 3.00E-02 | 4.59E-02 |
| isot                | 28 Ni 60 | 4.41E-03 | 4.43E-03 | 4.45E-03 | 4.45E-03 | 5.06E-03 | 4.35E-03 | 4.36E-03 | 4.37E-03 | 4.39E-03 | 4.84E-03 |
| isot                | 28 Ni 61 | 3.80E-05 | 4.07E-05 | 4.85E-05 | 6.33E-05 | 1.66E-04 | 3.85E-05 | 4.05E-05 | 4.50E-05 | 5.29E-05 | 1.07E-04 |
| isot                | 28 Ni 62 | 1.94E-03 | 1.97E-03 | 2.09E-03 | 2.34E-03 | 3.07E-03 | 1.93E-03 | 1.96E-03 | 2.07E-03 | 2.28E-03 | 2.80E-03 |
| isot                | 28 Ni 64 | 1.46E-04 | 1.50E-04 | 1.62E-04 | 1.94E-04 | 3.43E-04 | 1.47E-04 | 1.50E-04 | 1.60E-04 | 1.90E-04 | 3.15E-04 |
| elem                | 29 Cu    | 2.40E-06 | 2.75E-06 | 1.25E-05 | 3.56E-05 | 9.85E-05 | 2.62E-06 | 2.17E-06 | 7.50E-06 | 2.04E-05 | 5.23E-05 |
| isot                | 29 Cu 63 | 1.94E-06 | 1.76E-06 | 7.32E-06 | 1.55E-05 | 3.87E-05 | 2.17E-06 | 1.37E-06 | 4.31E-06 | 8.76E-06 | 1.97E-05 |
| isot                | 29 Cu 65 | 4.57E-07 | 9.89E-07 | 5.22E-06 | 2.01E-05 | 5.98E-05 | 4.50E-07 | 7.92E-07 | 3.18E-06 | 1.16E-05 | 3.25E-05 |
| elem                | 30 Zn    | 7.36E-06 | 1.54E-05 | 6.52E-05 | 1.44E-04 | 1.50E-04 | 7.75E-06 | 1.15E-05 | 4.29E-05 | 9.43E-05 | 9.25E-05 |
| isot                | 30 Zn 64 | 4.89E-06 | 1.01E-05 | 2.24E-05 | 1.69E-05 | 6.96E-06 | 5.21E-06 | 6.70E-06 | 1.27E-05 | 1.00E-05 | 4.29E-06 |
| isot                | 30 Zn 66 | 2.27E-06 | 4.50E-06 | 4.02E-05 | 1.09E-04 | 1.03E-04 | 2.34E-06 | 4.22E-06 | 2.83E-05 | 7.23E-05 | 6.63E-05 |
| isot                | 30 Zn 67 | 1.05E-07 | 1.69E-07 | 6.29E-07 | 2.26E-06 | 9.70E-06 | 1.07E-07 | 1.45E-07 | 4.50E-07 | 1.42E-06 | 5.27E-06 |
| isot                | 30 Zn 68 | 9.17E-08 | 6.06E-07 | 1.98E-06 | 1.62E-05 | 2.93E-05 | 8.81E-08 | 4.67E-07 | 1.37E-06 | 1.04E-05 | 1.63E-05 |
| isot                | 30 Zn 70 | 6.89E-09 | 8.34E-09 | 2.69E-08 | 1.76E-07 | 7.70E-07 | 7.03E-09 | 7.90E-09 | 1.91E-08 | 1.15E-07 | 4.28E-07 |
| elem                | 31 Ga    | 1.95E-09 | 8.52E-08 | 1.15E-06 | 6.25E-06 | 4.32E-06 | 1.50E-09 | 6.58E-08 | 8.33E-07 | 4.05E-06 | 2.34E-06 |
| isot                | 31 Ga 69 | 1.70E-09 | 7.92E-08 | 1.04E-06 | 4.99E-06 | 2.79E-06 | 1.30E-09 | 6.14E-08 | 7.40E-07 | 3.20E-06 | 1.53E-06 |
| isot                | 31 Ga 71 | 2.49E-10 | 6.07E-09 | 1.13E-07 | 1.26E-06 | 1.53E-06 | 1.94E-10 | 4.41E-09 | 9.34E-08 | 8.52E-07 | 8.14E-07 |
| elem                | 32 Ge    | 9.14E-09 | 7.69E-07 | 1.42E-05 | 3.48E-05 | 8.17E-06 | 7.77E-09 | 7.66E-07 | 1.14E-05 | 2.50E-05 | 5.03E-06 |
| isot                | 32 Ge 70 | 5.81E-09 | 6.77E-07 | 1.10E-05 | 1.99E-05 | 3.39E-06 | 5.42E-09 | 6.63E-07 | 8.52E-06 | 1.40E-05 | 2.16E-06 |
| isot                | 32 Ge 72 | 2.30E-09 | 8.06E-08 | 3.08E-06 | 1.43E-05 | 4.12E-06 | 1.53E-09 | 9.31E-08 | 2.77E-06 | 1.06E-05 | 2.53E-06 |
| isot                | 32 Ge 73 | 5.10E-10 | 9.62E-09 | 5.66E-08 | 1.16E-07 | 1.56E-07 | 3.36E-10 | 7.69E-09 | 5.15E-08 | 8.30E-08 | 8.12E-08 |
| isot                | 32 Ge 74 | 3.12E-10 | 1.34E-09 | 3.40E-08 | 5.87E-07 | 4.61E-07 | 2.91E-10 | 9.02E-10 | 2.71E-08 | 4.04E-07 | 2.34E-07 |
| isot                | 32 Ge 76 | 2.02E-10 | 3.99E-10 | 2.22E-09 | 1.32E-08 | 4.14E-08 | 1.96E-10 | 2.99E-10 | 1.45E-09 | 8.29E-09 | 2.20E-08 |
| elem                | 33 As    | 1.60E-10 | 4.59E-09 | 9.58E-08 | 6.65E-07 | 1.67E-07 | 1.03E-10 | 4.57E-09 | 8.30E-08 | 4.69E-07 | 9.27E-08 |
| isot                | 33 As 75 | 1.60E-10 | 4.59E-09 | 9.58E-08 | 6.65E-07 | 1.67E-07 | 1.03E-10 | 4.57E-09 | 8.30E-08 | 4.69E-07 | 9.27E-08 |
| elem                | 34 Se    | 4.11E-09 | 2.56E-07 | 5.26E-06 | 8.92E-06 | 6.55E-07 | 3.56E-09 | 3.35E-07 | 5.40E-06 | 7.46E-06 | 4.24E-07 |
| isot                | 34 Se 74 | 3.05E-09 | 1.98E-07 | 2.53E-06 | 3.46E-06 | 1.96E-07 | 2.56E-09 | 2.46E-07 | 2.49E-06 | 2.95E-06 | 1.36E-07 |
| isot                | 34 Se 76 | 4.88E-10 | 5.43E-08 | 2.63E-06 | 4.95E-06 | 2.96E-07 | 5.86E-10 | 8.61E-08 | 2.80E-06 | 4.14E-06 | 2.02E-07 |
| isot                | 34 Se 77 | 3.46E-10 | 2.19E-09 | 1.06E-08 | 6.19E-08 | 4.48E-08 | 2.80E-10 | 1.63E-09 | 9.86E-09 | 4.26E-08 | 2.29E-08 |
| isot                | 34 Se 78 | 6.90E-11 | 1.20E-09 | 8.81E-08 | 4.16E-07 | 7.26E-08 | 4.12E-11 | 8.58E-10 | 9.13E-08 | 3.18E-07 | 4.21E-08 |
| isot                | 34 Se 80 | 1.56E-10 | 6.44E-10 | 4.97E-09 | 2.09E-08 | 4.60E-08 | 9.73E-11 | 3.43E-10 | 2.88E-09 | 1.16E-08 | 2.13E-08 |
| elem                | 35 Br    | 7.46E-11 | 3.00E-09 | 3.49E-08 | 5.25E-08 | 1.55E-08 | 5.23E-11 | 2.71E-09 | 3.23E-08 | 3.91E-08 | 7.79E-09 |
| isot                | 35 Br 79 | 7.46E-11 | 3.00E-09 | 3.49E-08 | 5.25E-08 | 1.55E-08 | 5.23E-11 | 2.71E-09 | 3.23E-08 | 3.91E-08 | 7.79E-09 |
| elem                | 36 Kr    | 1.45E-09 | 5.53E-08 | 9.76E-07 | 7.40E-07 | 3.11E-08 | 1.69E-09 | 7.79E-08 | 1.20E-06 | 6.96E-07 | 1.93E-08 |
| isot                | 36 Kr 78 | 1.29E-09 | 3.07E-08 | 2.06E-07 | 1.28E-07 | 5.62E-09 | 1.51E-09 | 3.97E-08 | 2.42E-07 | 1.20E-07 | 3.36E-09 |
| isot                | 36 Kr 80 | 1.65E-10 | 2.45E-08 | 7.70E-07 | 6.11E-07 | 2.55E-08 | 1.82E-10 | 3.82E-08 | 9.54E-07 | 5.76E-07 | 1.59E-08 |

Table 3 *continued.*

|                     |          |          |          |          |          |          |          |          |          |          |          |
|---------------------|----------|----------|----------|----------|----------|----------|----------|----------|----------|----------|----------|
| $\rho_{\text{DDT}}$ |          | 2.4E+07  | 2.4E+07  | 2.4E+07  | 2.4E+07  | 2.4E+07  | 2.8E+07  | 2.8E+07  | 2.8E+07  | 2.8E+07  | 2.8E+07  |
| Z                   |          | 2.25E-4  | 2.25E-3  | 9.00E-3  | 2.25E-2  | 6.75E-2  | 2.25E-4  | 2.25E-3  | 9.00E-3  | 2.25E-2  | 6.75E-2  |
| elem                | 2 He     | 1.09E-03 | 1.23E-03 | 2.62E-04 | 7.43E-04 | 8.03E-05 | 3.24E-03 | 3.24E-03 | 3.50E-03 | 2.82E-03 | 2.45E-03 |
| isot                | 2 He 3   | 1.58E-12 | 1.56E-12 | 1.54E-12 | 1.42E-12 | 1.16E-12 | 1.58E-12 | 1.56E-12 | 1.54E-12 | 1.42E-12 | 1.16E-12 |
| isot                | 2 He 4   | 1.09E-03 | 1.22E-03 | 2.62E-04 | 7.43E-04 | 8.03E-05 | 3.24E-03 | 3.24E-03 | 3.50E-03 | 2.82E-03 | 2.45E-03 |
| elem                | 6 C      | 1.24E-03 | 1.23E-03 | 1.28E-03 | 1.27E-03 | 1.28E-03 | 1.02E-03 | 1.02E-03 | 1.02E-03 | 1.01E-03 | 9.98E-04 |
| isot                | 6 C 12   | 1.24E-03 | 1.23E-03 | 1.28E-03 | 1.27E-03 | 1.28E-03 | 1.02E-03 | 1.02E-03 | 1.02E-03 | 1.01E-03 | 9.98E-04 |
| isot                | 6 C 13   | 7.75E-11 | 1.09E-09 | 4.42E-09 | 1.07E-08 | 2.75E-08 | 6.17E-11 | 7.90E-10 | 3.24E-09 | 7.83E-09 | 1.99E-08 |
| elem                | 7 N      | 1.14E-05 | 8.94E-06 | 6.09E-06 | 3.57E-06 | 1.34E-06 | 9.86E-06 | 7.79E-06 | 5.23E-06 | 3.01E-06 | 1.05E-06 |
| isot                | 7 N 14   | 1.13E-05 | 8.94E-06 | 6.09E-06 | 3.57E-06 | 1.34E-06 | 9.83E-06 | 7.79E-06 | 5.23E-06 | 3.01E-06 | 1.05E-06 |
| isot                | 7 N 15   | 4.19E-08 | 1.25E-09 | 7.53E-10 | 9.36E-10 | 1.30E-09 | 3.47E-08 | 1.06E-09 | 5.82E-10 | 7.03E-10 | 9.60E-10 |
| elem                | 8 O      | 6.54E-02 | 6.67E-02 | 7.15E-02 | 7.25E-02 | 7.48E-02 | 5.59E-02 | 5.75E-02 | 5.85E-02 | 6.11E-02 | 6.21E-02 |
| isot                | 8 O 16   | 6.54E-02 | 6.67E-02 | 7.15E-02 | 7.25E-02 | 7.48E-02 | 5.59E-02 | 5.75E-02 | 5.85E-02 | 6.11E-02 | 6.21E-02 |
| isot                | 8 O 17   | 2.81E-09 | 2.87E-08 | 6.42E-08 | 8.55E-08 | 8.83E-08 | 2.20E-09 | 2.17E-08 | 4.61E-08 | 6.22E-08 | 6.19E-08 |
| isot                | 8 O 18   | 6.85E-10 | 4.12E-10 | 4.48E-10 | 5.02E-10 | 5.11E-10 | 6.62E-10 | 3.33E-10 | 3.35E-10 | 3.63E-10 | 3.65E-10 |
| elem                | 9 F      | 8.68E-12 | 2.07E-12 | 3.85E-12 | 9.23E-12 | 3.06E-11 | 6.23E-12 | 1.61E-12 | 2.96E-12 | 7.15E-12 | 2.33E-11 |
| isot                | 9 F 19   | 8.68E-12 | 2.07E-12 | 3.85E-12 | 9.23E-12 | 3.06E-11 | 6.23E-12 | 1.61E-12 | 2.96E-12 | 7.15E-12 | 2.33E-11 |
| elem                | 10 Ne    | 6.75E-04 | 6.67E-04 | 7.06E-04 | 7.10E-04 | 7.70E-04 | 5.32E-04 | 5.31E-04 | 5.33E-04 | 5.44E-04 | 5.96E-04 |
| isot                | 10 Ne 20 | 6.75E-04 | 6.66E-04 | 7.02E-04 | 6.97E-04 | 7.08E-04 | 5.32E-04 | 5.31E-04 | 5.31E-04 | 5.35E-04 | 5.51E-04 |
| isot                | 10 Ne 21 | 2.70E-09 | 1.38E-08 | 4.15E-08 | 9.65E-08 | 3.69E-07 | 5.51E-09 | 1.11E-08 | 3.15E-08 | 7.60E-08 | 2.86E-07 |
| isot                | 10 Ne 22 | 9.31E-08 | 6.06E-07 | 3.66E-06 | 1.29E-05 | 6.18E-05 | 1.46E-07 | 4.67E-07 | 2.60E-06 | 9.14E-06 | 4.39E-05 |
| elem                | 11 Na    | 4.99E-06 | 5.25E-06 | 7.29E-06 | 1.14E-05 | 2.75E-05 | 3.94E-06 | 4.19E-06 | 5.53E-06 | 8.75E-06 | 2.10E-05 |
| isot                | 11 Na 23 | 4.99E-06 | 5.25E-06 | 7.29E-06 | 1.14E-05 | 2.75E-05 | 3.94E-06 | 4.19E-06 | 5.53E-06 | 8.75E-06 | 2.10E-05 |
| elem                | 12 Mg    | 1.06E-02 | 9.33E-03 | 7.26E-03 | 4.96E-03 | 2.80E-03 | 8.37E-03 | 7.47E-03 | 5.41E-03 | 3.77E-03 | 2.11E-03 |
| isot                | 12 Mg 24 | 1.06E-02 | 9.32E-03 | 7.25E-03 | 4.92E-03 | 2.66E-03 | 8.37E-03 | 7.47E-03 | 5.40E-03 | 3.74E-03 | 2.00E-03 |
| isot                | 12 Mg 25 | 2.92E-07 | 2.48E-06 | 6.96E-06 | 1.67E-05 | 5.12E-05 | 2.60E-07 | 1.95E-06 | 5.21E-06 | 1.27E-05 | 3.85E-05 |
| isot                | 12 Mg 26 | 3.48E-07 | 2.02E-06 | 9.49E-06 | 2.48E-05 | 9.40E-05 | 7.98E-07 | 1.73E-06 | 7.42E-06 | 1.98E-05 | 7.46E-05 |
| elem                | 13 Al    | 2.33E-05 | 9.12E-05 | 1.75E-04 | 2.00E-04 | 1.89E-04 | 1.83E-05 | 7.24E-05 | 1.30E-04 | 1.50E-04 | 1.43E-04 |
| isot                | 13 Al 27 | 2.33E-05 | 9.12E-05 | 1.75E-04 | 2.00E-04 | 1.89E-04 | 1.83E-05 | 7.24E-05 | 1.30E-04 | 1.50E-04 | 1.43E-04 |
| elem                | 14 Si    | 1.95E-01 | 2.00E-01 | 2.10E-01 | 2.12E-01 | 2.10E-01 | 1.73E-01 | 1.78E-01 | 1.83E-01 | 1.86E-01 | 1.86E-01 |
| isot                | 14 Si 28 | 1.95E-01 | 2.00E-01 | 2.10E-01 | 2.11E-01 | 2.07E-01 | 1.73E-01 | 1.78E-01 | 1.83E-01 | 1.85E-01 | 1.83E-01 |
| isot                | 14 Si 29 | 5.80E-05 | 1.44E-04 | 2.33E-04 | 3.47E-04 | 7.85E-04 | 5.03E-05 | 1.21E-04 | 1.84E-04 | 2.76E-04 | 6.14E-04 |
| isot                | 14 Si 30 | 8.61E-06 | 5.58E-05 | 3.17E-04 | 7.78E-04 | 2.73E-03 | 9.93E-06 | 4.68E-05 | 2.40E-04 | 6.05E-04 | 2.12E-03 |
| elem                | 15 P     | 2.79E-05 | 4.94E-05 | 1.29E-04 | 2.32E-04 | 5.06E-04 | 2.51E-05 | 4.32E-05 | 1.03E-04 | 1.90E-04 | 4.07E-04 |
| isot                | 15 P 31  | 2.79E-05 | 4.94E-05 | 1.29E-04 | 2.32E-04 | 5.06E-04 | 2.51E-05 | 4.32E-05 | 1.03E-04 | 1.90E-04 | 4.07E-04 |
| elem                | 16 S     | 1.38E-01 | 1.38E-01 | 1.42E-01 | 1.40E-01 | 1.23E-01 | 1.23E-01 | 1.23E-01 | 1.25E-01 | 1.23E-01 | 1.09E-01 |
| isot                | 16 S 32  | 1.38E-01 | 1.37E-01 | 1.41E-01 | 1.38E-01 | 1.16E-01 | 1.23E-01 | 1.23E-01 | 1.24E-01 | 1.21E-01 | 1.03E-01 |
| isot                | 16 S 33  | 2.93E-05 | 5.98E-05 | 1.21E-04 | 1.79E-04 | 2.85E-04 | 2.51E-05 | 5.25E-05 | 1.02E-04 | 1.53E-04 | 2.45E-04 |
| isot                | 16 S 34  | 1.43E-06 | 1.37E-04 | 7.81E-04 | 2.10E-03 | 6.79E-03 | 2.56E-06 | 1.24E-04 | 6.52E-04 | 1.81E-03 | 5.73E-03 |
| isot                | 16 S 36  | 1.03E-10 | 2.19E-09 | 2.37E-08 | 1.47E-07 | 4.25E-06 | 9.75E-11 | 1.78E-09 | 1.90E-08 | 1.19E-07 | 3.24E-06 |
| elem                | 17 Cl    | 9.85E-06 | 2.14E-05 | 5.85E-05 | 1.16E-04 | 2.15E-04 | 9.51E-06 | 2.00E-05 | 5.15E-05 | 1.03E-04 | 1.88E-04 |
| isot                | 17 Cl 35 | 6.35E-06 | 1.45E-05 | 4.49E-05 | 9.41E-05 | 1.76E-04 | 6.34E-06 | 1.36E-05 | 3.93E-05 | 8.28E-05 | 1.53E-04 |
| isot                | 17 Cl 37 | 3.50E-06 | 6.95E-06 | 1.36E-05 | 2.19E-05 | 3.86E-05 | 3.17E-06 | 6.46E-06 | 1.22E-05 | 1.99E-05 | 3.46E-05 |
| elem                | 18 Ar    | 3.73E-02 | 3.59E-02 | 3.54E-02 | 3.33E-02 | 2.73E-02 | 3.33E-02 | 3.22E-02 | 3.13E-02 | 2.95E-02 | 2.44E-02 |
| isot                | 18 Ar 36 | 3.73E-02 | 3.58E-02 | 3.50E-02 | 3.22E-02 | 2.35E-02 | 3.33E-02 | 3.22E-02 | 3.09E-02 | 2.85E-02 | 2.11E-02 |
| isot                | 18 Ar 38 | 3.07E-07 | 6.16E-05 | 3.89E-04 | 1.17E-03 | 3.74E-03 | 4.30E-07 | 5.74E-05 | 3.42E-04 | 1.05E-03 | 3.31E-03 |
| isot                | 18 Ar 40 | 1.39E-11 | 4.67E-10 | 5.48E-09 | 2.48E-08 | 3.04E-07 | 1.27E-11 | 3.74E-10 | 4.40E-09 | 2.03E-08 | 2.35E-07 |
| elem                | 19 K     | 3.53E-06 | 1.51E-05 | 4.51E-05 | 8.67E-05 | 1.53E-04 | 3.42E-06 | 1.44E-05 | 4.17E-05 | 7.99E-05 | 1.40E-04 |
| isot                | 19 K 39  | 2.69E-06 | 1.35E-05 | 4.18E-05 | 8.13E-05 | 1.45E-04 | 2.62E-06 | 1.29E-05 | 3.87E-05 | 7.49E-05 | 1.33E-04 |
| isot                | 19 K 40  | 3.37E-11 | 1.44E-09 | 1.03E-08 | 5.41E-08 | 1.71E-07 | 2.83E-11 | 1.27E-09 | 8.66E-09 | 4.47E-08 | 1.39E-07 |
| isot                | 19 K 41  | 8.43E-07 | 1.56E-06 | 3.28E-06 | 5.34E-06 | 8.01E-06 | 7.97E-07 | 1.48E-06 | 3.03E-06 | 4.93E-06 | 7.40E-06 |
| elem                | 20 Ca    | 4.54E-02 | 4.23E-02 | 3.98E-02 | 3.48E-02 | 2.39E-02 | 4.05E-02 | 3.80E-02 | 3.50E-02 | 3.08E-02 | 2.13E-02 |
| isot                | 20 Ca 40 | 4.54E-02 | 4.23E-02 | 3.97E-02 | 3.47E-02 | 2.37E-02 | 4.04E-02 | 3.80E-02 | 3.49E-02 | 3.07E-02 | 2.12E-02 |
| isot                | 20 Ca 42 | 5.05E-09 | 1.49E-06 | 1.07E-05 | 3.48E-05 | 1.09E-04 | 5.70E-09 | 1.41E-06 | 9.74E-06 | 3.18E-05 | 9.91E-05 |
| isot                | 20 Ca 43 | 2.37E-09 | 3.54E-09 | 1.72E-08 | 7.77E-08 | 3.79E-07 | 9.92E-09 | 1.13E-08 | 1.14E-07 | 1.11E-07 | 3.49E-07 |
| isot                | 20 Ca 44 | 3.87E-05 | 3.41E-05 | 3.01E-05 | 2.54E-05 | 1.77E-05 | 3.73E-05 | 3.46E-05 | 3.55E-05 | 2.82E-05 | 2.09E-05 |
| isot                | 20 Ca 46 | 4.77E-09 | 5.04E-09 | 7.55E-09 | 1.79E-08 | 1.62E-07 | 4.68E-09 | 4.92E-09 | 7.05E-09 | 1.56E-08 | 1.25E-07 |
| isot                | 20 Ca 48 | 1.77E-07 | 1.84E-07 | 2.18E-07 | 2.72E-07 | 6.21E-07 | 1.79E-07 | 1.86E-07 | 2.12E-07 | 2.73E-07 | 5.94E-07 |
| elem                | 21 Sc    | 1.41E-07 | 1.73E-07 | 2.74E-07 | 4.01E-07 | 7.62E-07 | 1.33E-07 | 1.64E-07 | 2.52E-07 | 3.64E-07 | 6.66E-07 |
| isot                | 21 Sc 45 | 1.41E-07 | 1.73E-07 | 2.74E-07 | 4.01E-07 | 7.62E-07 | 1.33E-07 | 1.64E-07 | 2.52E-07 | 3.64E-07 | 6.66E-07 |

Table 3 *continued.*

|                     |          |          |          |          |          |          |          |          |          |          |          |
|---------------------|----------|----------|----------|----------|----------|----------|----------|----------|----------|----------|----------|
| $\rho_{\text{DDT}}$ |          | 2.4E+07  | 2.4E+07  | 2.4E+07  | 2.4E+07  | 2.4E+07  | 2.8E+07  | 2.8E+07  | 2.8E+07  | 2.8E+07  | 2.8E+07  |
| Z                   |          | 2.25E-4  | 2.25E-3  | 9.00E-3  | 2.25E-2  | 6.75E-2  | 2.25E-4  | 2.25E-3  | 9.00E-3  | 2.25E-2  | 6.75E-2  |
| elem                | 22 Ti    | 1.03E-03 | 1.02E-03 | 1.03E-03 | 1.00E-03 | 1.03E-03 | 9.67E-04 | 9.63E-04 | 9.57E-04 | 9.51E-04 | 9.94E-04 |
| isot                | 22 Ti 46 | 1.95E-07 | 1.54E-06 | 8.84E-06 | 2.37E-05 | 5.81E-05 | 1.24E-06 | 1.49E-06 | 8.19E-06 | 2.17E-05 | 5.37E-05 |
| isot                | 22 Ti 47 | 1.88E-07 | 2.28E-08 | 1.09E-07 | 5.01E-07 | 2.15E-06 | 1.56E-06 | 8.24E-08 | 3.29E-07 | 6.29E-07 | 2.11E-06 |
| isot                | 22 Ti 48 | 5.97E-04 | 5.71E-04 | 5.48E-04 | 4.60E-04 | 3.00E-04 | 5.38E-04 | 5.22E-04 | 4.82E-04 | 4.16E-04 | 2.75E-04 |
| isot                | 22 Ti 49 | 6.69E-06 | 1.41E-05 | 2.26E-05 | 3.05E-05 | 3.75E-05 | 6.02E-06 | 1.30E-05 | 1.98E-05 | 2.74E-05 | 3.39E-05 |
| isot                | 22 Ti 50 | 4.23E-04 | 4.28E-04 | 4.48E-04 | 4.88E-04 | 6.30E-04 | 4.21E-04 | 4.27E-04 | 4.47E-04 | 4.86E-04 | 6.29E-04 |
| elem                | 23 V     | 6.54E-05 | 7.67E-05 | 1.13E-04 | 1.53E-04 | 2.20E-04 | 6.46E-05 | 7.49E-05 | 1.06E-04 | 1.43E-04 | 2.06E-04 |
| isot                | 23 V 50  | 1.57E-08 | 1.58E-08 | 1.85E-08 | 4.12E-08 | 1.63E-07 | 1.52E-08 | 1.54E-08 | 1.80E-08 | 3.44E-08 | 1.27E-07 |
| isot                | 23 V 51  | 6.54E-05 | 7.67E-05 | 1.13E-04 | 1.53E-04 | 2.20E-04 | 6.45E-05 | 7.48E-05 | 1.06E-04 | 1.43E-04 | 2.06E-04 |
| elem                | 24 Cr    | 2.14E-02 | 2.11E-02 | 2.20E-02 | 2.01E-02 | 1.86E-02 | 1.97E-02 | 1.96E-02 | 1.90E-02 | 1.84E-02 | 1.73E-02 |
| isot                | 24 Cr 50 | 4.56E-05 | 6.42E-05 | 1.49E-04 | 3.36E-04 | 1.11E-03 | 5.11E-05 | 6.22E-05 | 1.35E-04 | 3.04E-04 | 1.01E-03 |
| isot                | 24 Cr 52 | 1.81E-02 | 1.75E-02 | 1.78E-02 | 1.51E-02 | 1.18E-02 | 1.64E-02 | 1.60E-02 | 1.49E-02 | 1.37E-02 | 1.08E-02 |
| isot                | 24 Cr 53 | 6.50E-04 | 9.09E-04 | 1.35E-03 | 1.69E-03 | 2.14E-03 | 6.10E-04 | 8.58E-04 | 1.17E-03 | 1.54E-03 | 1.94E-03 |
| isot                | 24 Cr 54 | 2.63E-03 | 2.65E-03 | 2.75E-03 | 2.94E-03 | 3.58E-03 | 2.63E-03 | 2.65E-03 | 2.75E-03 | 2.94E-03 | 3.58E-03 |
| elem                | 25 Mn    | 3.94E-03 | 5.97E-03 | 1.00E-02 | 1.32E-02 | 1.98E-02 | 3.92E-03 | 5.73E-03 | 8.60E-03 | 1.21E-02 | 1.77E-02 |
| isot                | 25 Mn 55 | 3.94E-03 | 5.97E-03 | 1.00E-02 | 1.32E-02 | 1.98E-02 | 3.92E-03 | 5.73E-03 | 8.60E-03 | 1.21E-02 | 1.77E-02 |
| elem                | 26 Fe    | 8.25E-01 | 8.22E-01 | 8.00E-01 | 7.90E-01 | 7.75E-01 | 8.79E-01 | 8.74E-01 | 8.61E-01 | 8.46E-01 | 8.09E-01 |
| isot                | 26 Fe 54 | 3.22E-02 | 3.54E-02 | 5.01E-02 | 7.62E-02 | 1.65E-01 | 3.22E-02 | 3.50E-02 | 4.66E-02 | 7.09E-02 | 1.49E-01 |
| isot                | 26 Fe 56 | 7.80E-01 | 7.72E-01 | 7.34E-01 | 6.94E-01 | 5.83E-01 | 8.33E-01 | 8.23E-01 | 7.95E-01 | 7.52E-01 | 6.29E-01 |
| isot                | 26 Fe 57 | 6.41E-03 | 8.00E-03 | 8.85E-03 | 1.31E-02 | 1.86E-02 | 7.35E-03 | 9.63E-03 | 1.24E-02 | 1.59E-02 | 2.27E-02 |
| isot                | 26 Fe 58 | 6.43E-03 | 6.49E-03 | 6.68E-03 | 7.06E-03 | 8.27E-03 | 6.43E-03 | 6.49E-03 | 6.68E-03 | 7.07E-03 | 8.27E-03 |
| elem                | 27 Co    | 7.30E-04 | 4.16E-04 | 4.17E-04 | 5.08E-04 | 4.97E-04 | 1.13E-03 | 4.26E-04 | 5.85E-04 | 6.91E-04 | 8.88E-04 |
| isot                | 27 Co 59 | 7.30E-04 | 4.16E-04 | 4.17E-04 | 5.08E-04 | 4.97E-04 | 1.13E-03 | 4.26E-04 | 5.85E-04 | 6.91E-04 | 8.88E-04 |
| elem                | 28 Ni    | 2.96E-02 | 3.04E-02 | 3.23E-02 | 4.44E-02 | 7.88E-02 | 3.29E-02 | 3.33E-02 | 4.02E-02 | 5.34E-02 | 1.03E-01 |
| isot                | 28 Ni 58 | 2.22E-02 | 2.26E-02 | 2.58E-02 | 3.67E-02 | 7.11E-02 | 2.26E-02 | 2.26E-02 | 2.88E-02 | 4.21E-02 | 8.93E-02 |
| isot                | 28 Ni 60 | 5.28E-03 | 5.66E-03 | 4.33E-03 | 4.97E-03 | 4.66E-03 | 8.15E-03 | 8.46E-03 | 8.52E-03 | 7.54E-03 | 7.11E-03 |
| isot                | 28 Ni 61 | 4.33E-05 | 5.75E-05 | 4.23E-05 | 6.88E-05 | 7.35E-05 | 6.29E-05 | 1.11E-04 | 1.59E-04 | 1.74E-04 | 2.49E-04 |
| isot                | 28 Ni 62 | 1.92E-03 | 1.97E-03 | 2.03E-03 | 2.45E-03 | 2.69E-03 | 1.92E-03 | 2.00E-03 | 2.55E-03 | 3.35E-03 | 6.11E-03 |
| isot                | 28 Ni 64 | 1.46E-04 | 1.49E-04 | 1.62E-04 | 1.87E-04 | 2.97E-04 | 1.47E-04 | 1.50E-04 | 1.61E-04 | 1.88E-04 | 2.92E-04 |
| elem                | 29 Cu    | 1.36E-05 | 3.71E-06 | 3.97E-06 | 9.25E-06 | 2.55E-05 | 5.45E-05 | 1.11E-05 | 4.12E-06 | 8.20E-06 | 2.25E-05 |
| isot                | 29 Cu 63 | 1.32E-05 | 3.04E-06 | 2.31E-06 | 4.22E-06 | 9.05E-06 | 5.39E-05 | 1.02E-05 | 2.33E-06 | 3.96E-06 | 9.12E-06 |
| isot                | 29 Cu 65 | 4.54E-07 | 6.71E-07 | 1.66E-06 | 5.03E-06 | 1.64E-05 | 5.26E-07 | 8.97E-07 | 1.79E-06 | 4.24E-06 | 1.34E-05 |
| elem                | 30 Zn    | 2.18E-05 | 2.10E-05 | 2.37E-05 | 5.40E-05 | 5.50E-05 | 8.36E-05 | 8.38E-05 | 4.92E-05 | 7.11E-05 | 1.13E-04 |
| isot                | 30 Zn 64 | 1.91E-05 | 1.66E-05 | 5.90E-06 | 5.99E-06 | 2.52E-06 | 7.93E-05 | 7.75E-05 | 2.42E-05 | 1.49E-05 | 1.07E-05 |
| isot                | 30 Zn 66 | 2.28E-06 | 3.96E-06 | 1.67E-05 | 4.19E-05 | 4.10E-05 | 2.46E-06 | 5.65E-06 | 2.41E-05 | 5.14E-05 | 9.31E-05 |
| isot                | 30 Zn 67 | 1.76E-07 | 1.26E-07 | 2.88E-07 | 7.05E-07 | 2.52E-06 | 5.69E-07 | 1.61E-07 | 2.54E-07 | 5.90E-07 | 1.96E-06 |
| isot                | 30 Zn 68 | 2.29E-07 | 3.29E-07 | 7.73E-07 | 5.37E-06 | 8.73E-06 | 1.31E-06 | 4.24E-07 | 6.20E-07 | 4.18E-06 | 7.09E-06 |
| isot                | 30 Zn 70 | 7.30E-09 | 7.80E-09 | 1.37E-08 | 6.00E-08 | 2.24E-07 | 7.37E-09 | 7.85E-09 | 1.27E-08 | 4.91E-08 | 1.75E-07 |
| elem                | 31 Ga    | 1.19E-09 | 4.39E-08 | 4.83E-07 | 2.27E-06 | 1.33E-06 | 1.83E-09 | 3.83E-08 | 3.78E-07 | 1.79E-06 | 1.09E-06 |
| isot                | 31 Ga 69 | 9.79E-10 | 4.08E-08 | 4.17E-07 | 1.78E-06 | 8.67E-07 | 1.11E-09 | 3.53E-08 | 3.23E-07 | 1.41E-06 | 7.21E-07 |
| isot                | 31 Ga 71 | 2.09E-10 | 3.05E-09 | 6.51E-08 | 4.89E-07 | 4.60E-07 | 7.11E-10 | 3.01E-09 | 5.54E-08 | 3.89E-07 | 3.68E-07 |
| elem                | 32 Ge    | 7.65E-09 | 6.60E-07 | 7.87E-06 | 1.61E-05 | 3.11E-06 | 4.10E-08 | 6.45E-07 | 6.75E-06 | 1.40E-05 | 3.38E-06 |
| isot                | 32 Ge 70 | 4.83E-09 | 5.57E-07 | 5.62E-06 | 8.69E-06 | 1.38E-06 | 2.28E-08 | 5.46E-07 | 4.79E-06 | 7.54E-06 | 1.90E-06 |
| isot                | 32 Ge 72 | 2.20E-09 | 9.51E-08 | 2.17E-06 | 7.10E-06 | 1.55E-06 | 1.75E-08 | 9.26E-08 | 1.90E-06 | 6.14E-06 | 1.33E-06 |
| isot                | 32 Ge 73 | 2.16E-10 | 6.35E-09 | 4.82E-08 | 6.08E-08 | 4.08E-08 | 1.88E-10 | 5.73E-09 | 4.45E-08 | 5.41E-08 | 3.13E-08 |
| isot                | 32 Ge 74 | 2.40E-10 | 5.93E-10 | 2.13E-08 | 2.77E-07 | 1.29E-07 | 2.66E-10 | 5.66E-10 | 1.85E-08 | 2.38E-07 | 1.08E-07 |
| isot                | 32 Ge 76 | 1.73E-10 | 2.24E-10 | 9.74E-10 | 5.16E-09 | 1.11E-08 | 1.96E-10 | 2.45E-10 | 8.50E-10 | 4.49E-09 | 8.43E-09 |
| elem                | 33 As    | 5.48E-11 | 4.87E-09 | 7.54E-08 | 3.46E-07 | 5.50E-08 | 4.46E-11 | 4.73E-09 | 6.90E-08 | 3.09E-07 | 4.78E-08 |
| isot                | 33 As 75 | 5.48E-11 | 4.87E-09 | 7.54E-08 | 3.46E-07 | 5.50E-08 | 4.46E-11 | 4.73E-09 | 6.90E-08 | 3.09E-07 | 4.78E-08 |
| elem                | 34 Se    | 2.84E-09 | 4.03E-07 | 5.05E-06 | 6.04E-06 | 2.79E-07 | 2.64E-09 | 4.05E-07 | 4.81E-06 | 5.67E-06 | 2.48E-07 |
| isot                | 34 Se 74 | 2.06E-09 | 2.74E-07 | 2.20E-06 | 2.38E-06 | 9.50E-08 | 1.90E-09 | 2.69E-07 | 2.04E-06 | 2.21E-06 | 8.75E-08 |
| isot                | 34 Se 76 | 5.19E-10 | 1.26E-07 | 2.74E-06 | 3.36E-06 | 1.40E-07 | 5.07E-10 | 1.34E-07 | 2.66E-06 | 3.18E-06 | 1.25E-07 |
| isot                | 34 Se 77 | 1.84E-10 | 1.57E-09 | 1.09E-08 | 3.39E-08 | 1.27E-08 | 1.62E-10 | 1.57E-09 | 1.11E-08 | 3.09E-08 | 1.04E-08 |
| isot                | 34 Se 78 | 2.26E-11 | 7.92E-10 | 9.91E-08 | 2.58E-07 | 2.24E-08 | 1.96E-11 | 7.80E-10 | 9.79E-08 | 2.45E-07 | 1.84E-08 |
| isot                | 34 Se 80 | 5.67E-11 | 1.69E-10 | 1.76E-09 | 7.16E-09 | 9.15E-09 | 4.93E-11 | 1.39E-10 | 1.62E-09 | 6.51E-09 | 7.10E-09 |
| elem                | 35 Br    | 3.89E-11 | 3.38E-09 | 3.84E-08 | 3.56E-08 | 3.73E-09 | 3.45E-11 | 3.52E-09 | 4.07E-08 | 3.60E-08 | 2.84E-09 |
| isot                | 35 Br 79 | 3.89E-11 | 3.38E-09 | 3.84E-08 | 3.56E-08 | 3.73E-09 | 3.45E-11 | 3.52E-09 | 4.07E-08 | 3.60E-08 | 2.84E-09 |
| elem                | 36 Kr    | 1.48E-09 | 1.25E-07 | 1.42E-06 | 6.69E-07 | 1.27E-08 | 1.41E-09 | 1.40E-07 | 1.50E-06 | 6.60E-07 | 1.09E-08 |
| isot                | 36 Kr 78 | 1.26E-09 | 5.75E-08 | 2.82E-07 | 1.19E-07 | 2.23E-09 | 1.19E-09 | 6.19E-08 | 2.98E-07 | 1.19E-07 | 1.86E-09 |
| isot                | 36 Kr 80 | 2.21E-10 | 6.80E-08 | 1.14E-06 | 5.50E-07 | 1.05E-08 | 2.19E-10 | 7.81E-08 | 1.20E-06 | 5.41E-07 | 9.04E-09 |

Table 3 *continued.*

|                     |          |          |          |          |          |          |
|---------------------|----------|----------|----------|----------|----------|----------|
| $\rho_{\text{DDT}}$ |          | 4.0E+07  | 4.0E+07  | 4.0E+07  | 4.0E+07  | 4.0E+07  |
| Z                   |          | 2.25E-4  | 2.25E-3  | 9.00E-3  | 2.25E-2  | 6.75E-2  |
| elem                | 2 He     | 8.56E-03 | 8.63E-03 | 8.18E-03 | 7.50E-03 | 5.82E-03 |
| isot                | 2 He 3   | 1.63E-12 | 1.61E-12 | 1.49E-12 | 1.46E-12 | 1.12E-12 |
| isot                | 2 He 4   | 8.56E-03 | 8.63E-03 | 8.18E-03 | 7.50E-03 | 5.82E-03 |
| elem                | 6 C      | 5.55E-04 | 5.52E-04 | 5.54E-04 | 5.51E-04 | 5.31E-04 |
| isot                | 6 C 12   | 5.55E-04 | 5.52E-04 | 5.54E-04 | 5.51E-04 | 5.31E-04 |
| isot                | 6 C 13   | 3.38E-11 | 4.82E-10 | 2.18E-09 | 5.13E-09 | 1.22E-08 |
| elem                | 7 N      | 7.23E-06 | 5.65E-06 | 3.77E-06 | 2.13E-06 | 6.35E-07 |
| isot                | 7 N 14   | 7.21E-06 | 5.65E-06 | 3.77E-06 | 2.13E-06 | 6.34E-07 |
| isot                | 7 N 15   | 2.09E-08 | 7.39E-10 | 3.63E-10 | 3.75E-10 | 5.04E-10 |
| elem                | 8 O      | 3.51E-02 | 3.62E-02 | 3.80E-02 | 3.93E-02 | 3.98E-02 |
| isot                | 8 O 16   | 3.51E-02 | 3.62E-02 | 3.80E-02 | 3.93E-02 | 3.98E-02 |
| isot                | 8 O 17   | 1.53E-09 | 1.23E-08 | 2.39E-08 | 3.02E-08 | 2.83E-08 |
| isot                | 8 O 18   | 5.30E-10 | 2.09E-10 | 1.72E-10 | 1.67E-10 | 1.68E-10 |
| elem                | 9 F      | 2.90E-12 | 8.57E-13 | 1.48E-12 | 3.56E-12 | 1.16E-11 |
| isot                | 9 F 19   | 2.90E-12 | 8.57E-13 | 1.48E-12 | 3.56E-12 | 1.16E-11 |
| elem                | 10 Ne    | 2.64E-04 | 2.58E-04 | 2.62E-04 | 2.66E-04 | 2.74E-04 |
| isot                | 10 Ne 20 | 2.63E-04 | 2.58E-04 | 2.61E-04 | 2.61E-04 | 2.49E-04 |
| isot                | 10 Ne 21 | 1.31E-08 | 6.18E-09 | 1.55E-08 | 3.78E-08 | 1.45E-07 |
| isot                | 10 Ne 22 | 1.66E-07 | 2.79E-07 | 1.52E-06 | 5.15E-06 | 2.41E-05 |
| elem                | 11 Na    | 2.02E-06 | 2.10E-06 | 2.81E-06 | 4.44E-06 | 1.05E-05 |
| isot                | 11 Na 23 | 2.02E-06 | 2.10E-06 | 2.81E-06 | 4.44E-06 | 1.05E-05 |
| elem                | 12 Mg    | 4.50E-03 | 3.93E-03 | 2.88E-03 | 1.95E-03 | 1.06E-03 |
| isot                | 12 Mg 24 | 4.50E-03 | 3.93E-03 | 2.87E-03 | 1.93E-03 | 1.01E-03 |
| isot                | 12 Mg 25 | 2.04E-07 | 9.86E-07 | 2.64E-06 | 6.28E-06 | 1.82E-05 |
| isot                | 12 Mg 26 | 1.63E-06 | 9.36E-07 | 3.70E-06 | 9.90E-06 | 3.54E-05 |
| elem                | 13 Al    | 9.98E-06 | 3.83E-05 | 6.80E-05 | 7.68E-05 | 6.89E-05 |
| isot                | 13 Al 27 | 9.98E-06 | 3.83E-05 | 6.80E-05 | 7.68E-05 | 6.89E-05 |
| elem                | 14 Si    | 1.27E-01 | 1.30E-01 | 1.35E-01 | 1.38E-01 | 1.37E-01 |
| isot                | 14 Si 28 | 1.27E-01 | 1.30E-01 | 1.35E-01 | 1.38E-01 | 1.35E-01 |
| isot                | 14 Si 29 | 3.52E-05 | 6.95E-05 | 1.08E-04 | 1.60E-04 | 3.36E-04 |
| isot                | 14 Si 30 | 1.59E-05 | 2.80E-05 | 1.34E-04 | 3.28E-04 | 1.15E-03 |
| elem                | 15 P     | 2.01E-05 | 2.83E-05 | 6.54E-05 | 1.17E-04 | 2.45E-04 |
| isot                | 15 P 31  | 2.01E-05 | 2.83E-05 | 6.54E-05 | 1.17E-04 | 2.45E-04 |
| elem                | 16 S     | 9.32E-02 | 9.28E-02 | 9.43E-02 | 9.34E-02 | 8.11E-02 |
| isot                | 16 S 32  | 9.32E-02 | 9.26E-02 | 9.38E-02 | 9.21E-02 | 7.71E-02 |
| isot                | 16 S 33  | 1.58E-05 | 3.42E-05 | 6.66E-05 | 1.02E-04 | 1.66E-04 |
| isot                | 16 S 34  | 7.90E-06 | 8.36E-05 | 4.37E-04 | 1.19E-03 | 3.80E-03 |
| isot                | 16 S 36  | 9.03E-11 | 9.49E-10 | 9.93E-09 | 6.40E-08 | 1.68E-06 |
| elem                | 17 Cl    | 9.22E-06 | 1.56E-05 | 3.81E-05 | 7.42E-05 | 1.33E-04 |
| isot                | 17 Cl 35 | 6.97E-06 | 1.08E-05 | 2.90E-05 | 5.94E-05 | 1.07E-04 |
| isot                | 17 Cl 37 | 2.24E-06 | 4.80E-06 | 9.13E-06 | 1.49E-05 | 2.52E-05 |
| elem                | 18 Ar    | 2.54E-02 | 2.45E-02 | 2.38E-02 | 2.26E-02 | 1.84E-02 |
| isot                | 18 Ar 36 | 2.54E-02 | 2.44E-02 | 2.35E-02 | 2.18E-02 | 1.60E-02 |
| isot                | 18 Ar 38 | 1.35E-06 | 4.08E-05 | 2.47E-04 | 7.43E-04 | 2.35E-03 |
| isot                | 18 Ar 40 | 1.06E-11 | 1.80E-10 | 2.09E-09 | 9.93E-09 | 1.18E-07 |
| elem                | 19 K     | 3.47E-06 | 1.13E-05 | 3.40E-05 | 6.31E-05 | 1.06E-04 |
| isot                | 19 K 39  | 2.82E-06 | 1.01E-05 | 3.16E-05 | 5.92E-05 | 9.99E-05 |
| isot                | 19 K 40  | 1.82E-11 | 8.83E-10 | 5.94E-09 | 2.98E-08 | 8.86E-08 |
| isot                | 19 K 41  | 6.49E-07 | 1.17E-06 | 2.36E-06 | 3.85E-06 | 5.61E-06 |
| elem                | 20 Ca    | 3.09E-02 | 2.88E-02 | 2.66E-02 | 2.36E-02 | 1.62E-02 |
| isot                | 20 Ca 40 | 3.09E-02 | 2.88E-02 | 2.65E-02 | 2.35E-02 | 1.61E-02 |
| isot                | 20 Ca 42 | 9.29E-09 | 1.05E-06 | 7.27E-06 | 2.35E-05 | 7.20E-05 |
| isot                | 20 Ca 43 | 5.35E-08 | 7.89E-08 | 4.13E-07 | 3.37E-07 | 3.00E-07 |
| isot                | 20 Ca 44 | 4.20E-05 | 4.96E-05 | 5.11E-05 | 4.31E-05 | 2.58E-05 |
| isot                | 20 Ca 46 | 4.66E-09 | 4.80E-09 | 5.97E-09 | 1.02E-08 | 5.96E-08 |
| isot                | 20 Ca 48 | 1.76E-07 | 1.83E-07 | 2.00E-07 | 2.66E-07 | 5.57E-07 |
| elem                | 21 Sc    | 1.17E-07 | 1.36E-07 | 1.99E-07 | 2.82E-07 | 4.68E-07 |
| isot                | 21 Sc 45 | 1.17E-07 | 1.36E-07 | 1.99E-07 | 2.82E-07 | 4.68E-07 |

Table 3 *continued.*

|                     |          |          |          |          |          |          |
|---------------------|----------|----------|----------|----------|----------|----------|
| $\rho_{\text{DDT}}$ |          | 4.0E+07  | 4.0E+07  | 4.0E+07  | 4.0E+07  | 4.0E+07  |
| Z                   |          | 2.25E-4  | 2.25E-3  | 9.00E-3  | 2.25E-2  | 6.75E-2  |
| elem                | 22 Ti    | 8.62E-04 | 8.62E-04 | 8.64E-04 | 8.69E-04 | 9.16E-04 |
| isot                | 22 Ti 46 | 6.30E-06 | 1.32E-06 | 6.23E-06 | 1.66E-05 | 3.99E-05 |
| isot                | 22 Ti 47 | 7.53E-06 | 4.95E-07 | 9.17E-07 | 1.27E-06 | 1.92E-06 |
| isot                | 22 Ti 48 | 4.23E-04 | 4.25E-04 | 3.96E-04 | 3.45E-04 | 2.22E-04 |
| isot                | 22 Ti 49 | 4.74E-06 | 1.06E-05 | 1.58E-05 | 2.20E-05 | 2.70E-05 |
| isot                | 22 Ti 50 | 4.20E-04 | 4.25E-04 | 4.45E-04 | 4.84E-04 | 6.25E-04 |
| elem                | 23 V     | 6.43E-05 | 7.21E-05 | 9.71E-05 | 1.28E-04 | 1.78E-04 |
| isot                | 23 V 50  | 1.52E-08 | 1.53E-08 | 1.69E-08 | 2.54E-08 | 7.51E-08 |
| isot                | 23 V 51  | 6.43E-05 | 7.21E-05 | 9.71E-05 | 1.28E-04 | 1.78E-04 |
| elem                | 24 Cr    | 1.64E-02 | 1.63E-02 | 1.59E-02 | 1.57E-02 | 1.50E-02 |
| isot                | 24 Cr 50 | 7.16E-05 | 5.75E-05 | 1.13E-04 | 2.46E-04 | 7.83E-04 |
| isot                | 24 Cr 52 | 1.32E-02 | 1.28E-02 | 1.21E-02 | 1.12E-02 | 9.06E-03 |
| isot                | 24 Cr 53 | 5.25E-04 | 7.49E-04 | 9.87E-04 | 1.28E-03 | 1.61E-03 |
| isot                | 24 Cr 54 | 2.62E-03 | 2.65E-03 | 2.75E-03 | 2.94E-03 | 3.58E-03 |
| elem                | 25 Mn    | 3.87E-03 | 5.23E-03 | 7.51E-03 | 1.03E-02 | 1.49E-02 |
| isot                | 25 Mn 55 | 3.87E-03 | 5.23E-03 | 7.51E-03 | 1.03E-02 | 1.49E-02 |
| elem                | 26 Fe    | 9.87E-01 | 9.86E-01 | 9.69E-01 | 9.44E-01 | 8.83E-01 |
| isot                | 26 Fe 54 | 3.22E-02 | 3.43E-02 | 4.32E-02 | 6.20E-02 | 1.22E-01 |
| isot                | 26 Fe 56 | 9.39E-01 | 9.32E-01 | 9.02E-01 | 8.54E-01 | 7.23E-01 |
| isot                | 26 Fe 57 | 9.43E-03 | 1.32E-02 | 1.65E-02 | 2.10E-02 | 3.01E-02 |
| isot                | 26 Fe 58 | 6.44E-03 | 6.49E-03 | 6.69E-03 | 7.07E-03 | 8.28E-03 |
| elem                | 27 Co    | 1.75E-03 | 4.61E-04 | 8.00E-04 | 1.06E-03 | 1.43E-03 |
| isot                | 27 Co 59 | 1.75E-03 | 4.61E-04 | 8.00E-04 | 1.06E-03 | 1.43E-03 |
| elem                | 28 Ni    | 4.11E-02 | 4.13E-02 | 5.03E-02 | 7.07E-02 | 1.43E-01 |
| isot                | 28 Ni 58 | 2.35E-02 | 2.27E-02 | 3.16E-02 | 5.13E-02 | 1.21E-01 |
| isot                | 28 Ni 60 | 1.53E-02 | 1.60E-02 | 1.48E-02 | 1.34E-02 | 1.06E-02 |
| isot                | 28 Ni 61 | 1.26E-04 | 2.87E-04 | 3.56E-04 | 4.26E-04 | 5.17E-04 |
| isot                | 28 Ni 62 | 1.93E-03 | 2.10E-03 | 3.32E-03 | 5.36E-03 | 1.08E-02 |
| isot                | 28 Ni 64 | 1.49E-04 | 1.52E-04 | 1.63E-04 | 1.89E-04 | 2.89E-04 |
| elem                | 29 Cu    | 1.56E-04 | 2.77E-05 | 4.88E-06 | 8.02E-06 | 1.78E-05 |
| isot                | 29 Cu 63 | 1.55E-04 | 2.57E-05 | 2.51E-06 | 4.07E-06 | 8.94E-06 |
| isot                | 29 Cu 65 | 7.77E-07 | 2.00E-06 | 2.38E-06 | 3.95E-06 | 8.85E-06 |
| elem                | 30 Zn    | 2.82E-04 | 3.04E-04 | 1.03E-04 | 1.37E-04 | 1.99E-04 |
| isot                | 30 Zn 64 | 2.71E-04 | 2.90E-04 | 6.22E-05 | 4.45E-05 | 2.38E-05 |
| isot                | 30 Zn 66 | 2.98E-06 | 1.30E-05 | 3.98E-05 | 9.00E-05 | 1.70E-04 |
| isot                | 30 Zn 67 | 1.84E-06 | 3.16E-07 | 2.06E-07 | 4.31E-07 | 1.23E-06 |
| isot                | 30 Zn 68 | 5.84E-06 | 1.10E-06 | 4.22E-07 | 2.41E-06 | 4.34E-06 |
| isot                | 30 Zn 70 | 7.45E-09 | 7.89E-09 | 1.12E-08 | 3.40E-08 | 1.05E-07 |
| elem                | 31 Ga    | 5.28E-09 | 3.04E-08 | 2.39E-07 | 1.10E-06 | 6.70E-07 |
| isot                | 31 Ga 69 | 2.89E-09 | 2.73E-08 | 1.98E-07 | 8.54E-07 | 4.50E-07 |
| isot                | 31 Ga 71 | 2.38E-09 | 3.13E-09 | 4.09E-08 | 2.51E-07 | 2.20E-07 |
| elem                | 32 Ge    | 2.27E-07 | 7.49E-07 | 4.85E-06 | 1.04E-05 | 3.64E-06 |
| isot                | 32 Ge 70 | 1.23E-07 | 6.64E-07 | 3.50E-06 | 5.95E-06 | 2.63E-06 |
| isot                | 32 Ge 72 | 1.03E-07 | 8.02E-08 | 1.30E-06 | 4.21E-06 | 9.19E-07 |
| isot                | 32 Ge 73 | 2.06E-10 | 4.57E-09 | 3.70E-08 | 4.25E-08 | 1.83E-08 |
| isot                | 32 Ge 74 | 2.50E-10 | 4.74E-10 | 1.39E-08 | 1.66E-07 | 7.02E-08 |
| isot                | 32 Ge 76 | 1.88E-10 | 2.20E-10 | 7.96E-10 | 3.49E-09 | 5.10E-09 |
| elem                | 33 As    | 6.38E-11 | 4.26E-09 | 5.42E-08 | 2.29E-07 | 3.37E-08 |
| isot                | 33 As 75 | 6.38E-11 | 4.26E-09 | 5.42E-08 | 2.29E-07 | 3.37E-08 |
| elem                | 34 Se    | 2.39E-09 | 3.71E-07 | 3.84E-06 | 4.70E-06 | 1.95E-07 |
| isot                | 34 Se 74 | 1.73E-09 | 2.32E-07 | 1.56E-06 | 1.82E-06 | 7.43E-08 |
| isot                | 34 Se 76 | 4.91E-10 | 1.37E-07 | 2.18E-06 | 2.64E-06 | 9.89E-08 |
| isot                | 34 Se 77 | 1.14E-10 | 1.55E-09 | 1.08E-08 | 2.46E-08 | 6.38E-09 |
| isot                | 34 Se 78 | 1.39E-11 | 8.38E-10 | 8.77E-08 | 2.10E-07 | 1.17E-08 |
| isot                | 34 Se 80 | 4.17E-11 | 9.27E-11 | 1.39E-09 | 5.15E-09 | 3.45E-09 |
| elem                | 35 Br    | 2.89E-11 | 3.79E-09 | 4.12E-08 | 3.57E-08 | 1.74E-09 |
| isot                | 35 Br 79 | 2.89E-11 | 3.79E-09 | 4.12E-08 | 3.57E-08 | 1.74E-09 |
| elem                | 36 Kr    | 1.24E-09 | 1.68E-07 | 1.48E-06 | 6.71E-07 | 7.69E-09 |
| isot                | 36 Kr 78 | 1.01E-09 | 6.84E-08 | 2.99E-07 | 1.28E-07 | 1.40E-09 |
| isot                | 36 Kr 80 | 2.28E-10 | 9.97E-08 | 1.18E-06 | 5.43E-07 | 6.29E-09 |



Table 4. Nucleosynthesis in sub-Chandrasekhar models with  $\xi_{\text{CO}} = 0.9$ .

| $M_{\text{WD}}$ |          | 0.88     | 0.88     | 0.88     | 0.88     | 0.88     | 0.97     | 0.97     | 0.97     | 0.97     | 0.97     |
|-----------------|----------|----------|----------|----------|----------|----------|----------|----------|----------|----------|----------|
| Z               |          | 2.25E-4  | 2.25E-3  | 9.00E-3  | 2.25E-2  | 6.75E-2  | 2.25E-4  | 2.25E-3  | 9.00E-3  | 2.25E-2  | 6.75E-2  |
| elem            | 2 He     | 1.95E-07 | 1.94E-07 | 1.73E-07 | 1.30E-07 | 1.02E-08 | 2.21E-04 | 2.34E-04 | 2.67E-04 | 3.31E-04 | 4.90E-04 |
| isot            | 2 He 3   | 1.76E-16 | 1.76E-16 | 1.78E-16 | 1.83E-16 | 2.15E-16 | 6.37E-16 | 6.31E-16 | 6.14E-16 | 5.81E-16 | 4.83E-16 |
| isot            | 2 He 4   | 1.95E-07 | 1.94E-07 | 1.73E-07 | 1.29E-07 | 1.02E-08 | 2.20E-04 | 2.34E-04 | 2.67E-04 | 3.31E-04 | 4.90E-04 |
| elem            | 6 C      | 4.04E-03 | 4.03E-03 | 3.96E-03 | 3.82E-03 | 3.35E-03 | 1.67E-03 | 1.66E-03 | 1.63E-03 | 1.57E-03 | 1.37E-03 |
| isot            | 6 C 12   | 4.04E-03 | 4.03E-03 | 3.96E-03 | 3.82E-03 | 3.34E-03 | 1.67E-03 | 1.66E-03 | 1.63E-03 | 1.56E-03 | 1.37E-03 |
| isot            | 6 C 13   | 2.20E-10 | 3.65E-09 | 1.21E-08 | 2.59E-08 | 5.61E-08 | 9.51E-11 | 1.52E-09 | 5.65E-09 | 1.28E-08 | 2.83E-08 |
| elem            | 7 N      | 1.40E-05 | 1.09E-05 | 7.63E-06 | 5.06E-06 | 2.80E-06 | 1.14E-05 | 8.90E-06 | 5.87E-06 | 3.39E-06 | 1.22E-06 |
| isot            | 7 N 14   | 1.39E-05 | 1.09E-05 | 7.62E-06 | 5.06E-06 | 2.79E-06 | 1.14E-05 | 8.90E-06 | 5.87E-06 | 3.39E-06 | 1.22E-06 |
| isot            | 7 N 15   | 1.07E-07 | 3.04E-09 | 1.99E-09 | 2.79E-09 | 3.50E-09 | 4.36E-08 | 1.28E-09 | 7.84E-10 | 1.02E-09 | 1.25E-09 |
| elem            | 8 O      | 1.38E-01 | 1.39E-01 | 1.40E-01 | 1.41E-01 | 1.33E-01 | 7.45E-02 | 7.59E-02 | 7.66E-02 | 7.70E-02 | 7.18E-02 |
| isot            | 8 O 16   | 1.38E-01 | 1.39E-01 | 1.40E-01 | 1.41E-01 | 1.33E-01 | 7.45E-02 | 7.59E-02 | 7.66E-02 | 7.70E-02 | 7.18E-02 |
| isot            | 8 O 17   | 7.12E-09 | 1.01E-07 | 2.20E-07 | 2.95E-07 | 2.84E-07 | 3.52E-09 | 3.74E-08 | 7.59E-08 | 9.84E-08 | 8.38E-08 |
| isot            | 8 O 18   | 1.90E-09 | 1.52E-09 | 1.66E-09 | 1.98E-09 | 1.79E-09 | 6.78E-10 | 5.12E-10 | 5.38E-10 | 6.01E-10 | 5.13E-10 |
| elem            | 9 F      | 3.50E-11 | 8.80E-12 | 1.02E-11 | 2.41E-11 | 7.60E-11 | 1.03E-11 | 2.50E-12 | 3.95E-12 | 1.01E-11 | 3.06E-11 |
| isot            | 9 F 19   | 3.50E-11 | 8.80E-12 | 1.02E-11 | 2.41E-11 | 7.60E-11 | 1.03E-11 | 2.50E-12 | 3.95E-12 | 1.01E-11 | 3.06E-11 |
| elem            | 10 Ne    | 2.61E-03 | 2.59E-03 | 2.54E-03 | 2.48E-03 | 2.26E-03 | 8.52E-04 | 8.43E-04 | 8.24E-04 | 7.96E-04 | 7.32E-04 |
| isot            | 10 Ne 20 | 2.61E-03 | 2.59E-03 | 2.53E-03 | 2.43E-03 | 2.06E-03 | 8.52E-04 | 8.42E-04 | 8.18E-04 | 7.77E-04 | 6.54E-04 |
| isot            | 10 Ne 21 | 6.50E-09 | 4.45E-08 | 1.23E-07 | 2.74E-07 | 9.22E-07 | 2.93E-09 | 1.70E-08 | 4.99E-08 | 1.17E-07 | 3.79E-07 |
| isot            | 10 Ne 22 | 2.29E-07 | 2.91E-06 | 1.54E-05 | 4.88E-05 | 1.91E-04 | 9.87E-08 | 1.18E-06 | 6.09E-06 | 1.93E-05 | 7.79E-05 |
| elem            | 11 Na    | 1.78E-05 | 1.93E-05 | 2.43E-05 | 3.55E-05 | 7.19E-05 | 6.25E-06 | 6.71E-06 | 8.68E-06 | 1.31E-05 | 2.74E-05 |
| isot            | 11 Na 23 | 1.78E-05 | 1.93E-05 | 2.43E-05 | 3.55E-05 | 7.19E-05 | 6.25E-06 | 6.71E-06 | 8.68E-06 | 1.31E-05 | 2.74E-05 |
| elem            | 12 Mg    | 2.97E-02 | 2.65E-02 | 2.00E-02 | 1.38E-02 | 6.89E-03 | 1.21E-02 | 1.07E-02 | 7.80E-03 | 5.20E-03 | 2.51E-03 |
| isot            | 12 Mg 24 | 2.96E-02 | 2.65E-02 | 1.99E-02 | 1.37E-02 | 6.50E-03 | 1.21E-02 | 1.07E-02 | 7.78E-03 | 5.16E-03 | 2.37E-03 |
| isot            | 12 Mg 25 | 7.97E-07 | 7.87E-06 | 2.14E-05 | 5.19E-05 | 1.42E-04 | 3.51E-07 | 2.96E-06 | 8.02E-06 | 1.90E-05 | 5.01E-05 |
| isot            | 12 Mg 26 | 8.97E-07 | 6.68E-06 | 2.95E-05 | 7.60E-05 | 2.52E-04 | 3.25E-07 | 2.54E-06 | 1.14E-05 | 2.89E-05 | 9.12E-05 |
| elem            | 13 Al    | 7.61E-05 | 2.71E-04 | 5.06E-04 | 5.89E-04 | 5.00E-04 | 2.76E-05 | 1.05E-04 | 1.89E-04 | 2.12E-04 | 1.71E-04 |
| isot            | 13 Al 27 | 7.61E-05 | 2.71E-04 | 5.06E-04 | 5.89E-04 | 5.00E-04 | 2.76E-05 | 1.05E-04 | 1.89E-04 | 2.12E-04 | 1.71E-04 |
| elem            | 14 Si    | 2.63E-01 | 2.73E-01 | 2.79E-01 | 2.80E-01 | 2.71E-01 | 1.98E-01 | 2.05E-01 | 2.09E-01 | 2.09E-01 | 1.99E-01 |
| isot            | 14 Si 28 | 2.63E-01 | 2.73E-01 | 2.78E-01 | 2.77E-01 | 2.63E-01 | 1.98E-01 | 2.04E-01 | 2.08E-01 | 2.08E-01 | 1.96E-01 |
| isot            | 14 Si 29 | 1.21E-04 | 3.31E-04 | 4.97E-04 | 8.03E-04 | 1.75E-03 | 6.18E-05 | 1.64E-04 | 2.40E-04 | 3.58E-04 | 7.06E-04 |
| isot            | 14 Si 30 | 1.40E-05 | 1.37E-04 | 7.92E-04 | 1.98E-03 | 5.95E-03 | 5.69E-06 | 6.30E-05 | 3.38E-04 | 8.16E-04 | 2.47E-03 |
| elem            | 15 P     | 3.48E-05 | 9.54E-05 | 2.67E-04 | 4.98E-04 | 1.00E-03 | 2.42E-05 | 5.36E-05 | 1.36E-04 | 2.42E-04 | 4.67E-04 |
| isot            | 15 P 31  | 3.48E-05 | 9.54E-05 | 2.67E-04 | 4.98E-04 | 1.00E-03 | 2.42E-05 | 5.36E-05 | 1.36E-04 | 2.42E-04 | 4.67E-04 |
| elem            | 16 S     | 1.59E-01 | 1.61E-01 | 1.66E-01 | 1.66E-01 | 1.46E-01 | 1.34E-01 | 1.35E-01 | 1.36E-01 | 1.34E-01 | 1.14E-01 |
| isot            | 16 S 32  | 1.59E-01 | 1.61E-01 | 1.64E-01 | 1.62E-01 | 1.35E-01 | 1.34E-01 | 1.35E-01 | 1.36E-01 | 1.32E-01 | 1.07E-01 |
| isot            | 16 S 33  | 6.22E-05 | 1.15E-04 | 2.22E-04 | 3.22E-04 | 4.46E-04 | 3.39E-05 | 6.75E-05 | 1.27E-04 | 1.86E-04 | 2.71E-04 |
| isot            | 16 S 34  | 6.46E-07 | 2.45E-04 | 1.36E-03 | 3.71E-03 | 1.12E-02 | 4.52E-07 | 1.61E-04 | 8.51E-04 | 2.27E-03 | 6.68E-03 |
| isot            | 16 S 36  | 2.47E-11 | 5.54E-09 | 6.15E-08 | 3.78E-07 | 1.03E-05 | 1.16E-11 | 2.55E-09 | 2.75E-08 | 1.64E-07 | 3.86E-06 |
| elem            | 17 Cl    | 1.03E-05 | 3.10E-05 | 9.12E-05 | 1.86E-04 | 3.17E-04 | 9.09E-06 | 2.44E-05 | 6.36E-05 | 1.24E-04 | 2.11E-04 |
| isot            | 17 Cl 35 | 4.63E-06 | 2.14E-05 | 7.16E-05 | 1.55E-04 | 2.64E-04 | 4.85E-06 | 1.66E-05 | 4.88E-05 | 1.00E-04 | 1.73E-04 |
| isot            | 17 Cl 37 | 5.63E-06 | 9.58E-06 | 1.96E-05 | 3.08E-05 | 5.26E-05 | 4.24E-06 | 7.85E-06 | 1.48E-05 | 2.34E-05 | 3.84E-05 |
| elem            | 18 Ar    | 3.93E-02 | 3.78E-02 | 3.70E-02 | 3.55E-02 | 2.96E-02 | 3.49E-02 | 3.37E-02 | 3.26E-02 | 3.08E-02 | 2.48E-02 |
| isot            | 18 Ar 36 | 3.93E-02 | 3.77E-02 | 3.64E-02 | 3.37E-02 | 2.42E-02 | 3.49E-02 | 3.36E-02 | 3.22E-02 | 2.95E-02 | 2.08E-02 |
| isot            | 18 Ar 38 | 4.63E-07 | 9.87E-05 | 6.17E-04 | 1.80E-03 | 5.42E-03 | 3.73E-07 | 7.75E-05 | 4.47E-04 | 1.31E-03 | 3.94E-03 |
| isot            | 18 Ar 40 | 1.47E-11 | 1.35E-09 | 1.68E-08 | 7.72E-08 | 7.83E-07 | 5.72E-12 | 6.03E-10 | 7.14E-09 | 3.05E-08 | 2.88E-07 |
| elem            | 19 K     | 2.77E-06 | 1.98E-05 | 6.53E-05 | 1.21E-04 | 1.98E-04 | 3.25E-06 | 1.84E-05 | 5.17E-05 | 9.64E-05 | 1.60E-04 |
| isot            | 19 K 39  | 1.94E-06 | 1.79E-05 | 6.08E-05 | 1.14E-04 | 1.88E-04 | 2.31E-06 | 1.67E-05 | 4.81E-05 | 9.06E-05 | 1.51E-04 |
| isot            | 19 K 40  | 5.87E-11 | 2.57E-09 | 1.83E-08 | 1.05E-07 | 3.10E-07 | 3.85E-11 | 1.60E-09 | 1.04E-08 | 5.38E-08 | 1.52E-07 |
| isot            | 19 K 41  | 8.23E-07 | 1.88E-06 | 4.50E-06 | 7.13E-06 | 1.01E-05 | 9.39E-07 | 1.79E-06 | 3.62E-06 | 5.74E-06 | 8.13E-06 |
| elem            | 20 Ca    | 4.48E-02 | 4.09E-02 | 3.72E-02 | 3.26E-02 | 2.18E-02 | 4.16E-02 | 3.86E-02 | 3.52E-02 | 3.07E-02 | 2.03E-02 |
| isot            | 20 Ca 40 | 4.47E-02 | 4.09E-02 | 3.72E-02 | 3.26E-02 | 2.16E-02 | 4.16E-02 | 3.86E-02 | 3.52E-02 | 3.07E-02 | 2.01E-02 |
| isot            | 20 Ca 42 | 7.16E-09 | 2.18E-06 | 1.63E-05 | 5.06E-05 | 1.51E-04 | 5.86E-09 | 1.90E-06 | 1.24E-05 | 3.92E-05 | 1.17E-04 |
| isot            | 20 Ca 43 | 5.21E-10 | 3.75E-09 | 3.16E-08 | 1.42E-07 | 6.69E-07 | 6.92E-10 | 2.44E-09 | 1.83E-08 | 7.91E-08 | 3.57E-07 |
| isot            | 20 Ca 44 | 2.93E-05 | 2.52E-05 | 2.16E-05 | 1.82E-05 | 1.38E-05 | 3.19E-05 | 2.78E-05 | 2.40E-05 | 2.03E-05 | 1.42E-05 |
| isot            | 20 Ca 46 | 2.22E-12 | 6.26E-10 | 7.89E-09 | 4.06E-08 | 4.69E-07 | 8.51E-13 | 2.76E-10 | 3.22E-09 | 1.51E-08 | 1.47E-07 |
| isot            | 20 Ca 48 | 1.23E-11 | 1.21E-10 | 1.42E-09 | 9.30E-09 | 1.03E-07 | 4.69E-12 | 4.88E-11 | 6.29E-10 | 3.79E-09 | 3.69E-08 |
| elem            | 21 Sc    | 1.12E-07 | 1.54E-07 | 2.95E-07 | 4.97E-07 | 1.20E-06 | 1.28E-07 | 1.60E-07 | 2.57E-07 | 3.75E-07 | 6.78E-07 |
| isot            | 21 Sc 45 | 1.12E-07 | 1.54E-07 | 2.95E-07 | 4.97E-07 | 1.20E-06 | 1.28E-07 | 1.60E-07 | 2.57E-07 | 3.75E-07 | 6.78E-07 |

Table 4 *continued.*

| $M_{\text{WD}}$ |          | 0.88     | 0.88     | 0.88     | 0.88     | 0.88     | 0.97     | 0.97     | 0.97     | 0.97     | 0.97     |
|-----------------|----------|----------|----------|----------|----------|----------|----------|----------|----------|----------|----------|
| Z               |          | 2.25E-4  | 2.25E-3  | 9.00E-3  | 2.25E-2  | 6.75E-2  | 2.25E-4  | 2.25E-3  | 9.00E-3  | 2.25E-2  | 6.75E-2  |
| elem            | 22 Ti    | 3.81E-04 | 3.60E-04 | 3.35E-04 | 3.14E-04 | 2.91E-04 | 4.80E-04 | 4.64E-04 | 4.36E-04 | 4.00E-04 | 3.18E-04 |
| isot            | 22 Ti 46 | 4.74E-08 | 2.05E-06 | 1.33E-05 | 3.37E-05 | 7.68E-05 | 4.96E-08 | 1.93E-06 | 1.04E-05 | 2.68E-05 | 6.23E-05 |
| isot            | 22 Ti 47 | 5.65E-09 | 1.18E-08 | 1.58E-07 | 7.68E-07 | 3.40E-06 | 2.34E-08 | 9.35E-09 | 1.07E-07 | 5.04E-07 | 2.15E-06 |
| isot            | 22 Ti 48 | 3.74E-04 | 3.49E-04 | 3.08E-04 | 2.60E-04 | 1.82E-04 | 4.72E-04 | 4.52E-04 | 4.09E-04 | 3.50E-04 | 2.25E-04 |
| isot            | 22 Ti 49 | 6.48E-06 | 8.62E-06 | 1.38E-05 | 1.92E-05 | 2.46E-05 | 7.24E-06 | 1.04E-05 | 1.64E-05 | 2.29E-05 | 2.75E-05 |
| isot            | 22 Ti 50 | 3.44E-11 | 1.10E-09 | 8.79E-09 | 1.14E-07 | 3.99E-06 | 1.36E-11 | 4.08E-10 | 3.68E-09 | 4.25E-08 | 1.41E-06 |
| elem            | 23 V     | 2.62E-06 | 1.15E-05 | 3.24E-05 | 5.82E-05 | 1.05E-04 | 2.30E-06 | 1.47E-05 | 4.00E-05 | 7.02E-05 | 1.16E-04 |
| isot            | 23 V 50  | 2.09E-11 | 3.17E-10 | 8.70E-09 | 8.41E-08 | 3.44E-07 | 6.99E-12 | 1.33E-10 | 3.15E-09 | 2.69E-08 | 1.28E-07 |
| isot            | 23 V 51  | 2.62E-06 | 1.15E-05 | 3.24E-05 | 5.81E-05 | 1.05E-04 | 2.30E-06 | 1.47E-05 | 4.00E-05 | 7.02E-05 | 1.16E-04 |
| elem            | 24 Cr    | 7.70E-03 | 7.37E-03 | 6.90E-03 | 6.48E-03 | 6.50E-03 | 1.21E-02 | 1.18E-02 | 1.12E-02 | 1.04E-02 | 8.64E-03 |
| isot            | 24 Cr 50 | 1.13E-06 | 1.96E-05 | 9.53E-05 | 2.70E-04 | 1.04E-03 | 1.19E-06 | 1.86E-05 | 9.18E-05 | 2.58E-04 | 9.23E-04 |
| isot            | 24 Cr 52 | 7.48E-03 | 7.05E-03 | 6.31E-03 | 5.52E-03 | 4.48E-03 | 1.18E-02 | 1.14E-02 | 1.04E-02 | 9.10E-03 | 6.39E-03 |
| isot            | 24 Cr 53 | 2.16E-04 | 2.97E-04 | 4.89E-04 | 6.91E-04 | 9.82E-04 | 3.23E-04 | 4.41E-04 | 7.15E-04 | 1.01E-03 | 1.32E-03 |
| isot            | 24 Cr 54 | 2.30E-10 | 7.64E-09 | 5.04E-08 | 2.89E-07 | 1.75E-06 | 9.49E-11 | 3.54E-09 | 2.43E-08 | 1.40E-07 | 9.41E-07 |
| elem            | 25 Mn    | 1.94E-04 | 1.19E-03 | 2.68E-03 | 4.37E-03 | 7.36E-03 | 1.93E-04 | 1.80E-03 | 4.24E-03 | 7.01E-03 | 1.13E-02 |
| isot            | 25 Mn 55 | 1.94E-04 | 1.19E-03 | 2.68E-03 | 4.37E-03 | 7.36E-03 | 1.93E-04 | 1.80E-03 | 4.24E-03 | 7.01E-03 | 1.13E-02 |
| elem            | 26 Fe    | 1.92E-01 | 1.85E-01 | 1.82E-01 | 1.88E-01 | 2.39E-01 | 4.59E-01 | 4.54E-01 | 4.50E-01 | 4.53E-01 | 4.79E-01 |
| isot            | 26 Fe 54 | 8.43E-05 | 2.48E-03 | 1.15E-02 | 3.05E-02 | 9.48E-02 | 6.69E-05 | 2.81E-03 | 1.34E-02 | 3.52E-02 | 1.03E-01 |
| isot            | 26 Fe 56 | 1.91E-01 | 1.82E-01 | 1.69E-01 | 1.55E-01 | 1.41E-01 | 4.57E-01 | 4.49E-01 | 4.33E-01 | 4.12E-01 | 3.65E-01 |
| isot            | 26 Fe 57 | 5.69E-04 | 7.99E-04 | 1.37E-03 | 2.06E-03 | 3.31E-03 | 1.63E-03 | 2.36E-03 | 3.84E-03 | 6.00E-03 | 1.09E-02 |
| isot            | 26 Fe 58 | 1.44E-08 | 2.58E-07 | 6.48E-07 | 1.86E-06 | 1.78E-05 | 5.47E-09 | 8.33E-08 | 2.24E-07 | 7.01E-07 | 6.96E-06 |
| elem            | 27 Co    | 4.53E-07 | 1.79E-06 | 2.37E-06 | 6.31E-06 | 4.98E-05 | 8.46E-05 | 1.11E-05 | 2.70E-05 | 5.30E-05 | 1.50E-04 |
| isot            | 27 Co 59 | 4.53E-07 | 1.79E-06 | 2.37E-06 | 6.31E-06 | 4.98E-05 | 8.46E-05 | 1.11E-05 | 2.70E-05 | 5.30E-05 | 1.50E-04 |
| elem            | 28 Ni    | 8.02E-05 | 3.10E-04 | 1.19E-03 | 3.12E-03 | 9.77E-03 | 5.32E-04 | 8.80E-04 | 3.18E-03 | 8.83E-03 | 3.51E-02 |
| isot            | 28 Ni 58 | 7.90E-05 | 2.75E-04 | 1.05E-03 | 2.77E-03 | 8.53E-03 | 2.44E-04 | 5.13E-04 | 2.74E-03 | 8.12E-03 | 3.33E-02 |
| isot            | 28 Ni 60 | 1.15E-06 | 2.98E-05 | 9.05E-05 | 1.93E-04 | 6.34E-04 | 2.86E-04 | 3.51E-04 | 3.77E-04 | 4.91E-04 | 8.36E-04 |
| isot            | 28 Ni 61 | 2.02E-08 | 8.56E-07 | 5.04E-06 | 1.36E-05 | 7.28E-05 | 2.38E-06 | 4.43E-06 | 8.27E-06 | 1.70E-05 | 5.98E-05 |
| isot            | 28 Ni 62 | 3.63E-08 | 4.51E-06 | 3.76E-05 | 1.43E-04 | 4.95E-04 | 3.37E-07 | 1.08E-05 | 5.70E-05 | 1.99E-04 | 8.93E-04 |
| isot            | 28 Ni 64 | 1.44E-10 | 3.04E-08 | 6.31E-07 | 5.95E-06 | 3.92E-05 | 5.33E-11 | 1.20E-08 | 2.32E-07 | 2.05E-06 | 1.42E-05 |
| elem            | 29 Cu    | 2.82E-08 | 9.93E-07 | 7.56E-06 | 2.23E-05 | 5.62E-05 | 2.29E-06 | 4.46E-07 | 2.86E-06 | 8.13E-06 | 2.09E-05 |
| isot            | 29 Cu 63 | 2.28E-08 | 5.97E-07 | 4.27E-06 | 9.11E-06 | 2.02E-05 | 2.28E-06 | 2.47E-07 | 1.56E-06 | 3.35E-06 | 7.17E-06 |
| isot            | 29 Cu 65 | 5.43E-09 | 3.96E-07 | 3.28E-06 | 1.32E-05 | 3.60E-05 | 8.61E-09 | 1.99E-07 | 1.29E-06 | 4.78E-06 | 1.37E-05 |
| elem            | 30 Zn    | 2.45E-07 | 8.89E-06 | 4.79E-05 | 1.06E-04 | 9.35E-05 | 4.02E-06 | 5.20E-06 | 2.17E-05 | 4.81E-05 | 4.65E-05 |
| isot            | 30 Zn 64 | 2.23E-07 | 6.48E-06 | 1.53E-05 | 1.14E-05 | 4.39E-06 | 3.96E-06 | 3.62E-06 | 6.02E-06 | 4.96E-06 | 2.81E-06 |
| isot            | 30 Zn 66 | 6.02E-09 | 1.91E-06 | 3.06E-05 | 8.09E-05 | 6.54E-05 | 1.49E-08 | 1.29E-06 | 1.47E-05 | 3.72E-05 | 3.44E-05 |
| isot            | 30 Zn 67 | 1.54E-09 | 5.16E-08 | 3.57E-07 | 1.37E-06 | 5.30E-06 | 1.65E-08 | 2.74E-08 | 1.77E-07 | 5.73E-07 | 1.91E-06 |
| isot            | 30 Zn 68 | 1.49E-08 | 4.56E-07 | 1.56E-06 | 1.24E-05 | 1.80E-05 | 2.51E-08 | 2.64E-07 | 7.43E-07 | 5.37E-06 | 7.25E-06 |
| isot            | 30 Zn 70 | 3.46E-11 | 8.38E-10 | 1.28E-08 | 1.11E-07 | 4.30E-07 | 1.32E-11 | 3.19E-10 | 5.26E-09 | 4.71E-08 | 1.64E-07 |
| elem            | 31 Ga    | 1.21E-09 | 6.64E-08 | 8.86E-07 | 4.40E-06 | 2.43E-06 | 6.21E-10 | 4.25E-08 | 4.69E-07 | 2.10E-06 | 1.06E-06 |
| isot            | 31 Ga 69 | 1.04E-09 | 6.20E-08 | 8.00E-07 | 3.49E-06 | 1.57E-06 | 5.37E-10 | 3.97E-08 | 4.11E-07 | 1.65E-06 | 6.95E-07 |
| isot            | 31 Ga 71 | 1.71E-10 | 4.45E-09 | 8.57E-08 | 9.11E-07 | 8.60E-07 | 8.41E-11 | 2.83E-09 | 5.83E-08 | 4.52E-07 | 3.63E-07 |
| elem            | 32 Ge    | 6.14E-09 | 7.57E-07 | 1.25E-05 | 2.75E-05 | 5.24E-06 | 3.92E-09 | 6.61E-07 | 7.80E-06 | 1.53E-05 | 2.59E-06 |
| isot            | 32 Ge 70 | 3.98E-09 | 6.68E-07 | 9.55E-06 | 1.54E-05 | 2.21E-06 | 2.85E-09 | 5.61E-07 | 5.57E-06 | 8.26E-06 | 1.16E-06 |
| isot            | 32 Ge 72 | 1.66E-09 | 8.05E-08 | 2.86E-06 | 1.15E-05 | 2.67E-06 | 8.41E-10 | 9.46E-08 | 2.17E-06 | 6.73E-06 | 1.28E-06 |
| isot            | 32 Ge 73 | 4.19E-10 | 7.34E-09 | 4.27E-08 | 7.69E-08 | 8.46E-08 | 1.99E-10 | 5.43E-09 | 3.82E-08 | 4.92E-08 | 3.23E-08 |
| isot            | 32 Ge 74 | 5.99E-11 | 7.26E-10 | 2.91E-08 | 4.59E-07 | 2.54E-07 | 2.15E-11 | 3.36E-10 | 1.96E-08 | 2.51E-07 | 1.03E-07 |
| isot            | 32 Ge 76 | 2.31E-11 | 1.58E-10 | 1.36E-09 | 8.88E-09 | 2.39E-08 | 1.13E-11 | 5.36E-11 | 6.63E-10 | 4.14E-09 | 8.60E-09 |
| elem            | 33 As    | 1.32E-10 | 3.97E-09 | 8.24E-08 | 5.00E-07 | 9.51E-08 | 5.22E-11 | 4.26E-09 | 6.59E-08 | 3.01E-07 | 4.34E-08 |
| isot            | 33 As 75 | 1.32E-10 | 3.97E-09 | 8.24E-08 | 5.00E-07 | 9.51E-08 | 5.22E-11 | 4.26E-09 | 6.59E-08 | 3.01E-07 | 4.34E-08 |
| elem            | 34 Se    | 3.80E-09 | 2.71E-07 | 4.82E-06 | 7.02E-06 | 4.15E-07 | 2.95E-09 | 3.87E-07 | 4.85E-06 | 5.58E-06 | 2.34E-07 |
| isot            | 34 Se 74 | 2.79E-09 | 2.08E-07 | 2.28E-06 | 2.73E-06 | 1.26E-07 | 2.19E-09 | 2.66E-07 | 2.13E-06 | 2.22E-06 | 7.97E-08 |
| isot            | 34 Se 76 | 5.66E-10 | 6.03E-08 | 2.44E-06 | 3.89E-06 | 1.91E-07 | 5.26E-10 | 1.19E-07 | 2.62E-06 | 3.10E-06 | 1.16E-07 |
| isot            | 34 Se 77 | 3.20E-10 | 1.60E-09 | 8.45E-09 | 4.60E-08 | 2.60E-08 | 1.93E-10 | 1.22E-09 | 8.39E-09 | 2.86E-08 | 1.05E-08 |
| isot            | 34 Se 78 | 4.13E-11 | 9.33E-10 | 8.30E-08 | 3.29E-07 | 4.67E-08 | 1.92E-11 | 7.93E-10 | 9.26E-08 | 2.25E-07 | 1.96E-08 |
| isot            | 34 Se 80 | 8.27E-11 | 4.11E-10 | 3.67E-09 | 1.39E-08 | 2.54E-08 | 3.01E-11 | 1.50E-10 | 1.60E-09 | 6.32E-09 | 8.23E-09 |
| elem            | 35 Br    | 7.04E-11 | 2.59E-09 | 2.80E-08 | 3.53E-08 | 8.56E-09 | 4.23E-11 | 2.80E-09 | 3.07E-08 | 2.72E-08 | 3.14E-09 |
| isot            | 35 Br 79 | 7.04E-11 | 2.59E-09 | 2.80E-08 | 3.53E-08 | 8.56E-09 | 4.23E-11 | 2.80E-09 | 3.07E-08 | 2.72E-08 | 3.14E-09 |
| elem            | 36 Kr    | 1.77E-09 | 5.61E-08 | 8.71E-07 | 5.47E-07 | 1.96E-08 | 1.61E-09 | 1.11E-07 | 1.29E-06 | 5.74E-07 | 1.18E-08 |
| isot            | 36 Kr 78 | 1.60E-09 | 3.04E-08 | 1.70E-07 | 8.81E-08 | 3.43E-09 | 1.36E-09 | 5.01E-08 | 2.46E-07 | 9.71E-08 | 1.98E-09 |
| isot            | 36 Kr 80 | 1.63E-10 | 2.57E-08 | 7.01E-07 | 4.59E-07 | 1.62E-08 | 2.46E-10 | 6.08E-08 | 1.05E-06 | 4.77E-07 | 9.78E-09 |

Table 4 *continued.*

| $M_{\text{WD}}$ |          | 1.06     | 1.06     | 1.06     | 1.06     | 1.06     | 1.10     | 1.10     | 1.10     | 1.10     | 1.10     |
|-----------------|----------|----------|----------|----------|----------|----------|----------|----------|----------|----------|----------|
| Z               |          | 2.25E-4  | 2.25E-3  | 9.00E-3  | 2.25E-2  | 6.75E-2  | 2.25E-4  | 2.25E-3  | 9.00E-3  | 2.25E-2  | 6.75E-2  |
| elem            | 2 He     | 5.13E-03 | 5.12E-03 | 4.90E-03 | 4.42E-03 | 2.84E-03 | 7.04E-03 | 7.01E-03 | 6.63E-03 | 5.86E-03 | 3.52E-03 |
| isot            | 2 He 3   | 1.88E-15 | 1.87E-15 | 2.88E-15 | 2.71E-15 | 3.97E-15 | 6.25E-13 | 6.58E-13 | 7.15E-13 | 8.14E-13 | 1.07E-12 |
| isot            | 2 He 4   | 5.13E-03 | 5.12E-03 | 4.90E-03 | 4.42E-03 | 2.84E-03 | 7.04E-03 | 7.00E-03 | 6.63E-03 | 5.86E-03 | 3.52E-03 |
| elem            | 6 C      | 7.27E-04 | 7.26E-04 | 7.07E-04 | 6.75E-04 | 5.86E-04 | 4.98E-04 | 4.97E-04 | 4.83E-04 | 4.59E-04 | 3.96E-04 |
| isot            | 6 C 12   | 7.27E-04 | 7.26E-04 | 7.07E-04 | 6.75E-04 | 5.86E-04 | 4.98E-04 | 4.97E-04 | 4.83E-04 | 4.59E-04 | 3.96E-04 |
| isot            | 6 C 13   | 4.53E-11 | 6.64E-10 | 2.73E-09 | 6.32E-09 | 1.38E-08 | 3.77E-11 | 4.94E-10 | 1.97E-09 | 4.56E-09 | 9.65E-09 |
| elem            | 7 N      | 7.91E-06 | 6.17E-06 | 4.02E-06 | 2.19E-06 | 6.03E-07 | 6.34E-06 | 4.98E-06 | 3.24E-06 | 1.75E-06 | 4.42E-07 |
| isot            | 7 N 14   | 7.89E-06 | 6.17E-06 | 4.02E-06 | 2.19E-06 | 6.03E-07 | 6.33E-06 | 4.98E-06 | 3.24E-06 | 1.75E-06 | 4.42E-07 |
| isot            | 7 N 15   | 1.93E-08 | 6.89E-10 | 3.68E-10 | 3.88E-10 | 5.23E-10 | 1.29E-08 | 5.51E-10 | 2.75E-10 | 2.56E-10 | 3.50E-10 |
| elem            | 8 O      | 3.57E-02 | 3.69E-02 | 3.75E-02 | 3.75E-02 | 3.41E-02 | 2.42E-02 | 2.52E-02 | 2.56E-02 | 2.55E-02 | 2.28E-02 |
| isot            | 8 O 16   | 3.57E-02 | 3.69E-02 | 3.75E-02 | 3.75E-02 | 3.41E-02 | 2.42E-02 | 2.52E-02 | 2.56E-02 | 2.55E-02 | 2.28E-02 |
| isot            | 8 O 17   | 1.81E-09 | 1.50E-08 | 2.72E-08 | 3.28E-08 | 2.68E-08 | 1.32E-09 | 9.98E-09 | 1.72E-08 | 1.97E-08 | 1.56E-08 |
| isot            | 8 O 18   | 3.30E-10 | 1.97E-10 | 1.87E-10 | 1.86E-10 | 1.79E-10 | 2.47E-10 | 1.31E-10 | 1.17E-10 | 1.10E-10 | 1.11E-10 |
| elem            | 9 F      | 3.16E-12 | 8.11E-13 | 1.60E-12 | 4.23E-12 | 1.30E-11 | 1.92E-12 | 5.38E-13 | 1.09E-12 | 2.66E-12 | 8.16E-12 |
| isot            | 9 F 19   | 3.16E-12 | 8.11E-13 | 1.60E-12 | 4.23E-12 | 1.30E-11 | 1.92E-12 | 5.38E-13 | 1.09E-12 | 2.66E-12 | 8.16E-12 |
| elem            | 10 Ne    | 2.91E-04 | 2.88E-04 | 2.80E-04 | 2.69E-04 | 2.48E-04 | 1.79E-04 | 1.76E-04 | 1.72E-04 | 1.64E-04 | 1.51E-04 |
| isot            | 10 Ne 20 | 2.91E-04 | 2.87E-04 | 2.78E-04 | 2.61E-04 | 2.15E-04 | 1.79E-04 | 1.76E-04 | 1.70E-04 | 1.58E-04 | 1.29E-04 |
| isot            | 10 Ne 21 | 6.97E-09 | 6.82E-09 | 1.95E-08 | 4.78E-08 | 1.70E-07 | 7.13E-09 | 4.52E-09 | 1.27E-08 | 3.08E-08 | 1.13E-07 |
| isot            | 10 Ne 22 | 2.24E-07 | 5.25E-07 | 2.66E-06 | 8.24E-06 | 3.28E-05 | 2.08E-07 | 3.74E-07 | 1.86E-06 | 5.67E-06 | 2.21E-05 |
| elem            | 11 Na    | 2.21E-06 | 2.39E-06 | 3.16E-06 | 4.89E-06 | 1.07E-05 | 1.35E-06 | 1.47E-06 | 1.97E-06 | 3.07E-06 | 6.81E-06 |
| isot            | 11 Na 23 | 2.21E-06 | 2.39E-06 | 3.16E-06 | 4.89E-06 | 1.07E-05 | 1.35E-06 | 1.47E-06 | 1.97E-06 | 3.07E-06 | 6.81E-06 |
| elem            | 12 Mg    | 4.28E-03 | 3.75E-03 | 2.61E-03 | 1.66E-03 | 7.78E-04 | 2.48E-03 | 2.15E-03 | 1.46E-03 | 9.06E-04 | 4.22E-04 |
| isot            | 12 Mg 24 | 4.28E-03 | 3.75E-03 | 2.61E-03 | 1.64E-03 | 7.25E-04 | 2.48E-03 | 2.15E-03 | 1.45E-03 | 8.95E-04 | 3.89E-04 |
| isot            | 12 Mg 25 | 1.96E-07 | 1.05E-06 | 2.93E-06 | 6.89E-06 | 1.84E-05 | 1.61E-07 | 6.33E-07 | 1.80E-06 | 4.23E-06 | 1.15E-05 |
| isot            | 12 Mg 26 | 1.56E-06 | 9.72E-07 | 4.34E-06 | 1.13E-05 | 3.45E-05 | 1.41E-06 | 6.43E-07 | 2.72E-06 | 7.19E-06 | 2.21E-05 |
| elem            | 13 Al    | 9.88E-06 | 3.70E-05 | 6.28E-05 | 6.69E-05 | 5.18E-05 | 6.05E-06 | 2.17E-05 | 3.55E-05 | 3.69E-05 | 2.83E-05 |
| isot            | 13 Al 27 | 9.88E-06 | 3.70E-05 | 6.28E-05 | 6.69E-05 | 5.18E-05 | 6.05E-06 | 2.17E-05 | 3.55E-05 | 3.69E-05 | 2.83E-05 |
| elem            | 14 Si    | 1.31E-01 | 1.35E-01 | 1.38E-01 | 1.38E-01 | 1.30E-01 | 1.04E-01 | 1.07E-01 | 1.10E-01 | 1.10E-01 | 1.02E-01 |
| isot            | 14 Si 28 | 1.31E-01 | 1.35E-01 | 1.38E-01 | 1.38E-01 | 1.29E-01 | 1.04E-01 | 1.07E-01 | 1.10E-01 | 1.10E-01 | 1.01E-01 |
| isot            | 14 Si 29 | 3.06E-05 | 6.80E-05 | 9.96E-05 | 1.42E-04 | 2.59E-04 | 2.37E-05 | 4.28E-05 | 6.30E-05 | 8.82E-05 | 1.56E-04 |
| isot            | 14 Si 30 | 5.57E-06 | 2.57E-05 | 1.25E-04 | 2.87E-04 | 8.68E-04 | 6.69E-06 | 1.64E-05 | 7.38E-05 | 1.65E-04 | 4.95E-04 |
| elem            | 15 P     | 1.72E-05 | 2.76E-05 | 6.27E-05 | 1.07E-04 | 1.99E-04 | 1.47E-05 | 1.97E-05 | 4.20E-05 | 7.02E-05 | 1.28E-04 |
| isot            | 15 P 31  | 1.72E-05 | 2.76E-05 | 6.27E-05 | 1.07E-04 | 1.99E-04 | 1.47E-05 | 1.97E-05 | 4.20E-05 | 7.02E-05 | 1.28E-04 |
| elem            | 16 S     | 9.60E-02 | 9.59E-02 | 9.62E-02 | 9.35E-02 | 7.73E-02 | 7.85E-02 | 7.85E-02 | 7.84E-02 | 7.58E-02 | 6.17E-02 |
| isot            | 16 S 32  | 9.60E-02 | 9.58E-02 | 9.57E-02 | 9.22E-02 | 7.38E-02 | 7.85E-02 | 7.84E-02 | 7.80E-02 | 7.50E-02 | 5.94E-02 |
| isot            | 16 S 33  | 1.64E-05 | 3.53E-05 | 6.56E-05 | 9.73E-05 | 1.45E-04 | 1.10E-05 | 2.46E-05 | 4.58E-05 | 6.83E-05 | 1.02E-04 |
| isot            | 16 S 34  | 1.31E-06 | 8.46E-05 | 4.36E-04 | 1.14E-03 | 3.31E-03 | 2.24E-06 | 5.81E-05 | 2.97E-04 | 7.72E-04 | 2.20E-03 |
| isot            | 16 S 36  | 5.48E-12 | 1.07E-09 | 1.19E-08 | 7.04E-08 | 1.34E-06 | 3.81E-12 | 7.00E-10 | 7.85E-09 | 4.67E-08 | 8.07E-07 |
| elem            | 17 Cl    | 6.95E-06 | 1.59E-05 | 3.95E-05 | 7.40E-05 | 1.22E-04 | 5.94E-06 | 1.21E-05 | 2.95E-05 | 5.46E-05 | 8.84E-05 |
| isot            | 17 Cl 35 | 4.40E-06 | 1.07E-05 | 2.98E-05 | 5.86E-05 | 9.86E-05 | 4.12E-06 | 8.08E-06 | 2.21E-05 | 4.29E-05 | 7.07E-05 |
| isot            | 17 Cl 37 | 2.54E-06 | 5.27E-06 | 9.74E-06 | 1.53E-05 | 2.39E-05 | 1.81E-06 | 4.02E-06 | 7.41E-06 | 1.17E-05 | 1.78E-05 |
| elem            | 18 Ar    | 2.58E-02 | 2.49E-02 | 2.39E-02 | 2.23E-02 | 1.74E-02 | 2.14E-02 | 2.07E-02 | 1.98E-02 | 1.84E-02 | 1.41E-02 |
| isot            | 18 Ar 36 | 2.58E-02 | 2.48E-02 | 2.36E-02 | 2.15E-02 | 1.52E-02 | 2.14E-02 | 2.07E-02 | 1.96E-02 | 1.79E-02 | 1.26E-02 |
| isot            | 18 Ar 38 | 4.38E-07 | 4.71E-05 | 2.67E-04 | 7.71E-04 | 2.23E-03 | 4.71E-07 | 3.36E-05 | 1.91E-04 | 5.50E-04 | 1.55E-03 |
| isot            | 18 Ar 40 | 2.24E-12 | 2.49E-10 | 2.99E-09 | 1.29E-08 | 1.06E-07 | 1.48E-12 | 1.62E-10 | 1.92E-09 | 8.45E-09 | 6.64E-08 |
| elem            | 19 K     | 2.78E-06 | 1.31E-05 | 3.59E-05 | 6.51E-05 | 1.03E-04 | 2.44E-06 | 1.01E-05 | 2.75E-05 | 4.94E-05 | 7.55E-05 |
| isot            | 19 K 39  | 2.06E-06 | 1.18E-05 | 3.33E-05 | 6.11E-05 | 9.72E-05 | 1.86E-06 | 9.02E-06 | 2.55E-05 | 4.63E-05 | 7.13E-05 |
| isot            | 19 K 40  | 2.02E-11 | 9.34E-10 | 5.78E-09 | 2.72E-08 | 7.35E-08 | 1.49E-11 | 6.93E-10 | 4.27E-09 | 1.97E-08 | 5.17E-08 |
| isot            | 19 K 41  | 7.16E-07 | 1.32E-06 | 2.57E-06 | 4.00E-06 | 5.44E-06 | 5.76E-07 | 1.05E-06 | 2.02E-06 | 3.13E-06 | 4.13E-06 |
| elem            | 20 Ca    | 3.11E-02 | 2.89E-02 | 2.63E-02 | 2.29E-02 | 1.51E-02 | 2.59E-02 | 2.42E-02 | 2.20E-02 | 1.92E-02 | 1.27E-02 |
| isot            | 20 Ca 40 | 3.11E-02 | 2.88E-02 | 2.62E-02 | 2.29E-02 | 1.51E-02 | 2.59E-02 | 2.42E-02 | 2.20E-02 | 1.92E-02 | 1.26E-02 |
| isot            | 20 Ca 42 | 4.48E-09 | 1.25E-06 | 8.05E-06 | 2.48E-05 | 7.00E-05 | 4.15E-09 | 9.20E-07 | 5.94E-06 | 1.82E-05 | 4.98E-05 |
| isot            | 20 Ca 43 | 2.17E-08 | 2.48E-08 | 1.12E-07 | 1.04E-07 | 1.96E-07 | 2.96E-08 | 3.58E-08 | 1.43E-07 | 1.12E-07 | 1.46E-07 |
| isot            | 20 Ca 44 | 3.39E-05 | 2.99E-05 | 2.92E-05 | 2.37E-05 | 1.32E-05 | 3.27E-05 | 2.97E-05 | 2.95E-05 | 2.36E-05 | 1.23E-05 |
| isot            | 20 Ca 46 | 3.85E-13 | 1.19E-10 | 1.40E-09 | 6.07E-09 | 4.63E-08 | 2.41E-13 | 7.82E-11 | 9.26E-10 | 3.98E-09 | 2.74E-08 |
| isot            | 20 Ca 48 | 1.86E-12 | 2.02E-11 | 2.96E-10 | 1.72E-09 | 1.38E-08 | 1.18E-12 | 1.29E-11 | 2.01E-10 | 1.19E-09 | 8.89E-09 |
| elem            | 21 Sc    | 1.18E-07 | 1.34E-07 | 1.97E-07 | 2.70E-07 | 4.10E-07 | 1.08E-07 | 1.15E-07 | 1.67E-07 | 2.25E-07 | 3.22E-07 |
| isot            | 21 Sc 45 | 1.18E-07 | 1.34E-07 | 1.97E-07 | 2.70E-07 | 4.10E-07 | 1.08E-07 | 1.15E-07 | 1.67E-07 | 2.25E-07 | 3.22E-07 |

Table 4 *continued.*

| $M_{\text{WD}}$ |          | 1.06     | 1.06     | 1.06     | 1.06     | 1.06     | 1.10     | 1.10     | 1.10     | 1.10     | 1.10     |
|-----------------|----------|----------|----------|----------|----------|----------|----------|----------|----------|----------|----------|
| Z               |          | 2.25E-4  | 2.25E-3  | 9.00E-3  | 2.25E-2  | 6.75E-2  | 2.25E-4  | 2.25E-3  | 9.00E-3  | 2.25E-2  | 6.75E-2  |
| elem            | 22 Ti    | 3.94E-04 | 3.85E-04 | 3.64E-04 | 3.31E-04 | 2.48E-04 | 3.45E-04 | 3.39E-04 | 3.21E-04 | 2.89E-04 | 2.10E-04 |
| isot            | 22 Ti 46 | 1.46E-06 | 1.34E-06 | 7.08E-06 | 1.80E-05 | 3.98E-05 | 1.88E-06 | 1.02E-06 | 5.33E-06 | 1.34E-05 | 2.88E-05 |
| isot            | 22 Ti 47 | 1.73E-06 | 1.11E-07 | 3.15E-07 | 5.64E-07 | 1.33E-06 | 1.96E-06 | 1.55E-07 | 3.79E-07 | 5.64E-07 | 1.02E-06 |
| isot            | 22 Ti 48 | 3.86E-04 | 3.75E-04 | 3.43E-04 | 2.94E-04 | 1.84E-04 | 3.38E-04 | 3.30E-04 | 3.03E-04 | 2.59E-04 | 1.61E-04 |
| isot            | 22 Ti 49 | 4.35E-06 | 8.66E-06 | 1.34E-05 | 1.87E-05 | 2.23E-05 | 3.29E-06 | 7.69E-06 | 1.18E-05 | 1.64E-05 | 1.95E-05 |
| isot            | 22 Ti 50 | 6.10E-12 | 1.60E-10 | 1.61E-09 | 1.54E-08 | 4.05E-07 | 3.94E-12 | 1.05E-10 | 1.11E-09 | 9.63E-09 | 2.14E-07 |
| elem            | 23 V     | 3.25E-06 | 1.18E-05 | 3.29E-05 | 5.76E-05 | 9.30E-05 | 3.56E-06 | 1.03E-05 | 2.88E-05 | 5.03E-05 | 8.09E-05 |
| isot            | 23 V 50  | 2.92E-12 | 6.37E-11 | 1.19E-09 | 8.46E-09 | 4.21E-08 | 1.95E-12 | 4.54E-11 | 7.61E-10 | 4.97E-09 | 2.50E-08 |
| isot            | 23 V 51  | 3.25E-06 | 1.18E-05 | 3.29E-05 | 5.76E-05 | 9.30E-05 | 3.56E-06 | 1.03E-05 | 2.88E-05 | 5.03E-05 | 8.09E-05 |
| elem            | 24 Cr    | 9.76E-03 | 9.59E-03 | 9.12E-03 | 8.40E-03 | 6.82E-03 | 8.41E-03 | 8.31E-03 | 7.90E-03 | 7.27E-03 | 5.89E-03 |
| isot            | 24 Cr 50 | 7.89E-06 | 1.35E-05 | 6.86E-05 | 1.94E-04 | 6.78E-04 | 9.03E-06 | 1.10E-05 | 5.71E-05 | 1.62E-04 | 5.61E-04 |
| isot            | 24 Cr 52 | 9.52E-03 | 9.21E-03 | 8.46E-03 | 7.38E-03 | 5.08E-03 | 8.23E-03 | 7.97E-03 | 7.33E-03 | 6.39E-03 | 4.39E-03 |
| isot            | 24 Cr 53 | 2.32E-04 | 3.68E-04 | 5.85E-04 | 8.28E-04 | 1.07E-03 | 1.79E-04 | 3.25E-04 | 5.10E-04 | 7.20E-04 | 9.38E-04 |
| isot            | 24 Cr 54 | 4.04E-11 | 1.60E-09 | 1.16E-08 | 6.70E-08 | 5.04E-07 | 2.59E-11 | 1.07E-09 | 8.19E-09 | 4.70E-08 | 3.64E-07 |
| elem            | 25 Mn    | 9.15E-05 | 1.42E-03 | 3.46E-03 | 5.75E-03 | 9.20E-03 | 8.50E-05 | 1.21E-03 | 3.00E-03 | 5.00E-03 | 8.80E-03 |
| isot            | 25 Mn 55 | 9.15E-05 | 1.42E-03 | 3.46E-03 | 5.75E-03 | 9.20E-03 | 8.50E-05 | 1.21E-03 | 3.00E-03 | 5.00E-03 | 8.80E-03 |
| elem            | 26 Fe    | 7.11E-01 | 7.08E-01 | 7.01E-01 | 6.91E-01 | 6.70E-01 | 8.14E-01 | 8.13E-01 | 8.03E-01 | 7.89E-01 | 7.49E-01 |
| isot            | 26 Fe 54 | 4.42E-05 | 2.02E-03 | 1.01E-02 | 2.65E-02 | 7.69E-02 | 3.93E-05 | 1.65E-03 | 8.40E-03 | 2.22E-02 | 6.64E-02 |
| isot            | 26 Fe 56 | 7.06E-01 | 6.99E-01 | 6.80E-01 | 6.51E-01 | 5.69E-01 | 8.07E-01 | 8.01E-01 | 7.81E-01 | 7.49E-01 | 6.54E-01 |
| isot            | 26 Fe 57 | 5.02E-03 | 7.71E-03 | 1.03E-02 | 1.43E-02 | 2.33E-02 | 6.99E-03 | 1.02E-02 | 1.32E-02 | 1.81E-02 | 2.86E-02 |
| isot            | 26 Fe 58 | 2.24E-09 | 2.94E-08 | 8.27E-08 | 2.63E-07 | 2.32E-06 | 1.45E-09 | 1.82E-08 | 5.23E-08 | 1.65E-07 | 1.33E-06 |
| elem            | 27 Co    | 7.33E-04 | 8.87E-05 | 2.96E-04 | 4.74E-04 | 6.64E-04 | 9.10E-04 | 1.37E-04 | 4.20E-04 | 6.51E-04 | 8.15E-04 |
| isot            | 27 Co 59 | 7.33E-04 | 8.87E-05 | 2.96E-04 | 4.74E-04 | 6.64E-04 | 9.10E-04 | 1.37E-04 | 4.20E-04 | 6.51E-04 | 8.15E-04 |
| elem            | 28 Ni    | 8.12E-03 | 8.25E-03 | 1.54E-02 | 3.16E-02 | 9.44E-02 | 1.11E-02 | 1.15E-02 | 2.07E-02 | 4.15E-02 | 1.17E-01 |
| isot            | 28 Ni 58 | 1.28E-03 | 7.63E-04 | 8.07E-03 | 2.41E-02 | 8.72E-02 | 1.60E-03 | 1.31E-03 | 1.09E-02 | 3.17E-02 | 1.09E-01 |
| isot            | 28 Ni 60 | 6.75E-03 | 7.14E-03 | 6.28E-03 | 5.36E-03 | 2.99E-03 | 9.37E-03 | 9.73E-03 | 8.49E-03 | 7.04E-03 | 3.54E-03 |
| isot            | 28 Ni 61 | 7.85E-05 | 1.45E-04 | 1.82E-04 | 2.20E-04 | 2.22E-04 | 1.17E-04 | 2.00E-04 | 2.47E-04 | 2.90E-04 | 2.68E-04 |
| isot            | 28 Ni 62 | 1.13E-05 | 2.08E-04 | 8.24E-04 | 1.93E-03 | 3.94E-03 | 3.81E-05 | 3.02E-04 | 1.13E-03 | 2.52E-03 | 4.69E-03 |
| isot            | 28 Ni 64 | 2.28E-11 | 4.98E-09 | 8.42E-08 | 6.32E-07 | 4.37E-06 | 1.55E-11 | 3.39E-09 | 5.33E-08 | 3.64E-07 | 2.34E-06 |
| elem            | 29 Cu    | 6.49E-05 | 5.17E-06 | 2.09E-06 | 4.23E-06 | 9.25E-06 | 7.95E-05 | 9.43E-06 | 2.08E-06 | 3.64E-06 | 6.87E-06 |
| isot            | 29 Cu 63 | 6.47E-05 | 4.63E-06 | 1.05E-06 | 2.08E-06 | 4.25E-06 | 7.91E-05 | 8.76E-06 | 1.04E-06 | 1.94E-06 | 3.78E-06 |
| isot            | 29 Cu 65 | 2.89E-07 | 5.40E-07 | 1.04E-06 | 2.15E-06 | 4.99E-06 | 3.76E-07 | 6.72E-07 | 1.04E-06 | 1.70E-06 | 3.10E-06 |
| elem            | 30 Zn    | 1.65E-04 | 7.85E-05 | 4.48E-05 | 6.12E-05 | 5.85E-05 | 2.15E-04 | 1.08E-04 | 5.37E-05 | 6.64E-05 | 6.10E-05 |
| isot            | 30 Zn 64 | 1.61E-04 | 7.30E-05 | 2.54E-05 | 1.75E-05 | 6.36E-06 | 2.10E-04 | 1.01E-04 | 3.23E-05 | 2.15E-05 | 7.28E-06 |
| isot            | 30 Zn 66 | 1.05E-06 | 5.29E-06 | 1.90E-05 | 4.15E-05 | 4.84E-05 | 1.79E-06 | 6.91E-06 | 2.11E-05 | 4.36E-05 | 5.15E-05 |
| isot            | 30 Zn 67 | 7.24E-07 | 2.01E-08 | 8.46E-08 | 2.39E-07 | 6.50E-07 | 8.32E-07 | 2.77E-08 | 5.99E-08 | 1.62E-07 | 3.91E-07 |
| isot            | 30 Zn 68 | 2.01E-06 | 2.11E-07 | 3.00E-07 | 2.00E-06 | 2.99E-06 | 2.45E-06 | 2.16E-07 | 1.91E-07 | 1.15E-06 | 1.81E-06 |
| isot            | 30 Zn 70 | 5.28E-12 | 1.37E-10 | 2.24E-09 | 1.84E-08 | 5.74E-08 | 3.60E-12 | 9.71E-11 | 1.52E-09 | 1.17E-08 | 3.40E-08 |
| elem            | 31 Ga    | 1.95E-09 | 2.42E-08 | 2.05E-07 | 9.00E-07 | 4.70E-07 | 2.46E-09 | 1.80E-08 | 1.33E-07 | 5.75E-07 | 3.12E-07 |
| isot            | 31 Ga 69 | 1.09E-09 | 2.22E-08 | 1.71E-07 | 6.99E-07 | 3.20E-07 | 1.34E-09 | 1.62E-08 | 1.08E-07 | 4.42E-07 | 2.15E-07 |
| isot            | 31 Ga 71 | 8.66E-10 | 2.01E-09 | 3.43E-08 | 2.01E-07 | 1.51E-07 | 1.12E-09 | 1.75E-09 | 2.56E-08 | 1.32E-07 | 9.67E-08 |
| elem            | 32 Ge    | 6.75E-08 | 5.09E-07 | 4.06E-06 | 8.21E-06 | 1.59E-06 | 8.99E-08 | 4.20E-07 | 2.73E-06 | 5.69E-06 | 1.22E-06 |
| isot            | 32 Ge 70 | 4.94E-08 | 4.34E-07 | 2.81E-06 | 4.38E-06 | 8.49E-07 | 6.82E-08 | 3.62E-07 | 1.88E-06 | 3.06E-06 | 7.13E-07 |
| isot            | 32 Ge 72 | 1.80E-08 | 7.15E-08 | 1.21E-06 | 3.66E-06 | 6.75E-07 | 2.16E-08 | 5.55E-08 | 8.10E-07 | 2.50E-06 | 4.67E-07 |
| isot            | 32 Ge 73 | 9.93E-11 | 3.68E-09 | 2.99E-08 | 3.38E-08 | 1.25E-08 | 8.73E-11 | 2.90E-09 | 2.47E-08 | 2.80E-08 | 7.94E-09 |
| isot            | 32 Ge 74 | 7.94E-12 | 1.87E-10 | 1.16E-08 | 1.39E-07 | 4.88E-08 | 4.83E-12 | 1.44E-10 | 8.39E-09 | 9.23E-08 | 3.17E-08 |
| isot            | 32 Ge 76 | 4.64E-12 | 2.27E-11 | 4.31E-10 | 2.43E-09 | 2.98E-09 | 2.81E-12 | 1.40E-11 | 3.71E-10 | 1.93E-09 | 1.79E-09 |
| elem            | 33 As    | 2.39E-11 | 3.73E-09 | 4.58E-08 | 1.89E-07 | 2.43E-08 | 1.78E-11 | 3.21E-09 | 3.52E-08 | 1.34E-07 | 1.69E-08 |
| isot            | 33 As 75 | 2.39E-11 | 3.73E-09 | 4.58E-08 | 1.89E-07 | 2.43E-08 | 1.78E-11 | 3.21E-09 | 3.52E-08 | 1.34E-07 | 1.69E-08 |
| elem            | 34 Se    | 2.26E-09 | 3.60E-07 | 3.51E-06 | 3.96E-06 | 1.41E-07 | 2.27E-09 | 2.98E-07 | 2.65E-06 | 3.17E-06 | 1.09E-07 |
| isot            | 34 Se 74 | 1.68E-09 | 2.23E-07 | 1.41E-06 | 1.53E-06 | 5.25E-08 | 1.68E-09 | 1.77E-07 | 1.03E-06 | 1.21E-06 | 4.22E-08 |
| isot            | 34 Se 76 | 4.64E-10 | 1.34E-07 | 2.00E-06 | 2.22E-06 | 7.23E-08 | 4.92E-10 | 1.19E-07 | 1.55E-06 | 1.79E-06 | 5.66E-08 |
| isot            | 34 Se 77 | 9.92E-11 | 1.24E-09 | 8.89E-09 | 1.97E-08 | 4.50E-09 | 8.09E-11 | 1.22E-09 | 8.64E-09 | 1.58E-08 | 2.95E-09 |
| isot            | 34 Se 78 | 7.55E-12 | 8.35E-10 | 8.43E-08 | 1.83E-07 | 9.15E-09 | 4.64E-12 | 7.74E-10 | 6.49E-08 | 1.46E-07 | 6.09E-09 |
| isot            | 34 Se 80 | 1.10E-11 | 5.67E-11 | 1.13E-09 | 4.14E-09 | 2.56E-09 | 6.65E-12 | 3.59E-11 | 1.03E-09 | 3.42E-09 | 1.49E-09 |
| elem            | 35 Br    | 2.13E-11 | 3.34E-09 | 3.50E-08 | 2.87E-08 | 1.27E-09 | 2.07E-11 | 3.24E-09 | 3.20E-08 | 2.68E-08 | 8.26E-10 |
| isot            | 35 Br 79 | 2.13E-11 | 3.34E-09 | 3.50E-08 | 2.87E-08 | 1.27E-09 | 2.07E-11 | 3.24E-09 | 3.20E-08 | 2.68E-08 | 8.26E-10 |
| elem            | 36 Kr    | 1.21E-09 | 1.63E-07 | 1.34E-06 | 5.55E-07 | 5.79E-09 | 1.21E-09 | 1.65E-07 | 1.20E-06 | 5.27E-07 | 4.25E-09 |
| isot            | 36 Kr 78 | 9.62E-10 | 6.43E-08 | 2.64E-07 | 1.05E-07 | 1.02E-09 | 9.53E-10 | 6.13E-08 | 2.39E-07 | 1.04E-07 | 7.85E-10 |
| isot            | 36 Kr 80 | 2.51E-10 | 9.90E-08 | 1.07E-06 | 4.50E-07 | 4.78E-09 | 2.61E-10 | 1.03E-07 | 9.58E-07 | 4.23E-07 | 3.46E-09 |

Table 4 *continued.*

| $M_{\text{WD}}$ |          | 1.15     | 1.15     | 1.15     | 1.15     | 1.15     |
|-----------------|----------|----------|----------|----------|----------|----------|
| Z               |          | 2.25E-4  | 2.25E-3  | 9.00E-3  | 2.25E-2  | 6.75E-2  |
| elem            | 2 He     | 8.74E-03 | 8.65E-03 | 8.10E-03 | 6.95E-03 | 4.06E-03 |
| isot            | 2 He 3   | 3.75E-12 | 3.76E-12 | 3.72E-12 | 3.71E-12 | 3.57E-12 |
| isot            | 2 He 4   | 8.73E-03 | 8.65E-03 | 8.10E-03 | 6.95E-03 | 4.06E-03 |
| elem            | 6 C      | 3.06E-04 | 3.04E-04 | 2.93E-04 | 2.77E-04 | 2.36E-04 |
| isot            | 6 C 12   | 3.05E-04 | 3.04E-04 | 2.93E-04 | 2.77E-04 | 2.36E-04 |
| isot            | 6 C 13   | 2.86E-11 | 3.07E-10 | 1.38E-09 | 3.25E-09 | 6.27E-09 |
| elem            | 7 N      | 4.34E-06 | 3.49E-06 | 2.31E-06 | 1.26E-06 | 2.95E-07 |
| isot            | 7 N 14   | 4.33E-06 | 3.49E-06 | 2.31E-06 | 1.26E-06 | 2.95E-07 |
| isot            | 7 N 15   | 7.75E-09 | 4.14E-10 | 1.86E-10 | 1.67E-10 | 2.03E-10 |
| elem            | 8 O      | 1.39E-02 | 1.45E-02 | 1.48E-02 | 1.46E-02 | 1.29E-02 |
| isot            | 8 O 16   | 1.39E-02 | 1.45E-02 | 1.48E-02 | 1.46E-02 | 1.29E-02 |
| isot            | 8 O 17   | 9.46E-10 | 6.19E-09 | 9.57E-09 | 1.07E-08 | 7.72E-09 |
| isot            | 8 O 18   | 1.88E-10 | 8.51E-11 | 6.65E-11 | 5.79E-11 | 5.79E-11 |
| elem            | 9 F      | 9.66E-13 | 3.23E-13 | 6.27E-13 | 1.54E-12 | 4.37E-12 |
| isot            | 9 F 19   | 9.66E-13 | 3.23E-13 | 6.27E-13 | 1.54E-12 | 4.37E-12 |
| elem            | 10 Ne    | 9.42E-05 | 9.30E-05 | 9.02E-05 | 8.59E-05 | 7.90E-05 |
| isot            | 10 Ne 20 | 9.41E-05 | 9.27E-05 | 8.90E-05 | 8.23E-05 | 6.56E-05 |
| isot            | 10 Ne 21 | 4.28E-09 | 2.84E-09 | 6.89E-09 | 1.79E-08 | 6.34E-08 |
| isot            | 10 Ne 22 | 1.56E-07 | 2.50E-07 | 1.19E-06 | 3.57E-06 | 1.34E-05 |
| elem            | 11 Na    | 7.07E-07 | 7.80E-07 | 1.06E-06 | 1.67E-06 | 3.72E-06 |
| isot            | 11 Na 23 | 7.07E-07 | 7.80E-07 | 1.06E-06 | 1.67E-06 | 3.72E-06 |
| elem            | 12 Mg    | 1.12E-03 | 9.58E-04 | 6.34E-04 | 3.88E-04 | 1.84E-04 |
| isot            | 12 Mg 24 | 1.12E-03 | 9.57E-04 | 6.32E-04 | 3.82E-04 | 1.66E-04 |
| isot            | 12 Mg 25 | 1.05E-07 | 3.25E-07 | 9.59E-07 | 2.24E-06 | 6.21E-06 |
| isot            | 12 Mg 26 | 9.53E-07 | 4.53E-07 | 1.48E-06 | 3.92E-06 | 1.22E-05 |
| elem            | 13 Al    | 3.15E-06 | 1.03E-05 | 1.62E-05 | 1.65E-05 | 1.26E-05 |
| isot            | 13 Al 27 | 3.15E-06 | 1.03E-05 | 1.62E-05 | 1.65E-05 | 1.26E-05 |
| elem            | 14 Si    | 7.33E-02 | 7.51E-02 | 7.66E-02 | 7.61E-02 | 6.83E-02 |
| isot            | 14 Si 28 | 7.33E-02 | 7.51E-02 | 7.65E-02 | 7.60E-02 | 6.80E-02 |
| isot            | 14 Si 29 | 1.84E-05 | 2.15E-05 | 3.22E-05 | 4.49E-05 | 7.83E-05 |
| isot            | 14 Si 30 | 7.91E-06 | 9.19E-06 | 3.48E-05 | 7.61E-05 | 2.26E-04 |
| elem            | 15 P     | 1.14E-05 | 1.25E-05 | 2.36E-05 | 3.85E-05 | 6.86E-05 |
| isot            | 15 P 31  | 1.14E-05 | 1.25E-05 | 2.36E-05 | 3.85E-05 | 6.86E-05 |
| elem            | 16 S     | 5.70E-02 | 5.69E-02 | 5.66E-02 | 5.42E-02 | 4.30E-02 |
| isot            | 16 S 32  | 5.70E-02 | 5.69E-02 | 5.64E-02 | 5.37E-02 | 4.18E-02 |
| isot            | 16 S 33  | 6.45E-06 | 1.46E-05 | 2.71E-05 | 4.05E-05 | 6.05E-05 |
| isot            | 16 S 34  | 3.33E-06 | 3.34E-05 | 1.66E-04 | 4.28E-04 | 1.21E-03 |
| isot            | 16 S 36  | 2.32E-12 | 4.02E-10 | 4.49E-09 | 2.71E-08 | 4.18E-07 |
| elem            | 17 Cl    | 4.63E-06 | 8.00E-06 | 1.89E-05 | 3.46E-05 | 5.50E-05 |
| isot            | 17 Cl 35 | 3.55E-06 | 5.35E-06 | 1.41E-05 | 2.70E-05 | 4.37E-05 |
| isot            | 17 Cl 37 | 1.08E-06 | 2.65E-06 | 4.82E-06 | 7.56E-06 | 1.13E-05 |
| elem            | 18 Ar    | 1.58E-02 | 1.54E-02 | 1.47E-02 | 1.36E-02 | 1.02E-02 |
| isot            | 18 Ar 36 | 1.58E-02 | 1.53E-02 | 1.46E-02 | 1.32E-02 | 9.25E-03 |
| isot            | 18 Ar 38 | 4.85E-07 | 2.01E-05 | 1.15E-04 | 3.30E-04 | 9.16E-04 |
| isot            | 18 Ar 40 | 8.76E-13 | 9.43E-11 | 1.07E-09 | 4.78E-09 | 3.61E-08 |
| elem            | 19 K     | 1.98E-06 | 6.51E-06 | 1.82E-05 | 3.21E-05 | 4.78E-05 |
| isot            | 19 K 39  | 1.57E-06 | 5.80E-06 | 1.68E-05 | 3.00E-05 | 4.50E-05 |
| isot            | 19 K 40  | 9.37E-12 | 4.46E-10 | 2.84E-09 | 1.28E-08 | 3.24E-08 |
| isot            | 19 K 41  | 4.05E-07 | 7.17E-07 | 1.35E-06 | 2.09E-06 | 2.72E-06 |
| elem            | 20 Ca    | 1.93E-02 | 1.82E-02 | 1.66E-02 | 1.45E-02 | 9.60E-03 |
| isot            | 20 Ca 40 | 1.92E-02 | 1.82E-02 | 1.66E-02 | 1.45E-02 | 9.56E-03 |
| isot            | 20 Ca 42 | 4.06E-09 | 5.71E-07 | 3.73E-06 | 1.14E-05 | 3.05E-05 |
| isot            | 20 Ca 43 | 3.87E-08 | 4.92E-08 | 1.80E-07 | 1.25E-07 | 1.00E-07 |
| isot            | 20 Ca 44 | 2.97E-05 | 2.81E-05 | 2.84E-05 | 2.24E-05 | 1.11E-05 |
| isot            | 20 Ca 46 | 1.60E-13 | 4.42E-11 | 5.29E-10 | 2.28E-09 | 1.39E-08 |
| isot            | 20 Ca 48 | 6.17E-13 | 7.55E-12 | 1.19E-10 | 7.13E-10 | 5.03E-09 |
| elem            | 21 Sc    | 9.69E-08 | 8.99E-08 | 1.25E-07 | 1.66E-07 | 2.29E-07 |
| isot            | 21 Sc 45 | 9.69E-08 | 8.99E-08 | 1.25E-07 | 1.66E-07 | 2.29E-07 |

Table 4 *continued.*

| $M_{\text{WD}}$ |          | 1.15     | 1.15     | 1.15     | 1.15     | 1.15     |
|-----------------|----------|----------|----------|----------|----------|----------|
| Z               |          | 2.25E-4  | 2.25E-3  | 9.00E-3  | 2.25E-2  | 6.75E-2  |
| elem            | 22 Ti    | 2.79E-04 | 2.77E-04 | 2.62E-04 | 2.35E-04 | 1.66E-04 |
| isot            | 22 Ti 46 | 2.35E-06 | 6.76E-07 | 3.37E-06 | 8.48E-06 | 1.80E-05 |
| isot            | 22 Ti 47 | 2.08E-06 | 2.06E-07 | 4.41E-07 | 5.64E-07 | 7.35E-07 |
| isot            | 22 Ti 48 | 2.72E-04 | 2.69E-04 | 2.49E-04 | 2.12E-04 | 1.31E-04 |
| isot            | 22 Ti 49 | 2.27E-06 | 6.36E-06 | 9.57E-06 | 1.33E-05 | 1.59E-05 |
| isot            | 22 Ti 50 | 2.17E-12 | 6.18E-11 | 6.95E-10 | 5.29E-09 | 9.34E-08 |
| elem            | 23 V     | 3.51E-06 | 8.19E-06 | 2.32E-05 | 4.05E-05 | 6.56E-05 |
| isot            | 23 V 50  | 1.08E-12 | 2.88E-11 | 4.24E-10 | 2.53E-09 | 1.30E-08 |
| isot            | 23 V 51  | 3.51E-06 | 8.19E-06 | 2.32E-05 | 4.05E-05 | 6.56E-05 |
| elem            | 24 Cr    | 6.67E-03 | 6.63E-03 | 6.31E-03 | 5.80E-03 | 4.83E-03 |
| isot            | 24 Cr 50 | 9.96E-06 | 8.02E-06 | 4.24E-05 | 1.20E-04 | 4.04E-04 |
| isot            | 24 Cr 52 | 6.55E-03 | 6.36E-03 | 5.85E-03 | 5.10E-03 | 3.62E-03 |
| isot            | 24 Cr 53 | 1.16E-04 | 2.67E-04 | 4.11E-04 | 5.78E-04 | 8.04E-04 |
| isot            | 24 Cr 54 | 1.43E-11 | 6.03E-10 | 5.03E-09 | 2.89E-08 | 2.31E-07 |
| elem            | 25 Mn    | 8.71E-05 | 9.46E-04 | 2.40E-03 | 4.00E-03 | 9.67E-03 |
| isot            | 25 Mn 55 | 8.71E-05 | 9.46E-04 | 2.40E-03 | 4.00E-03 | 9.67E-03 |
| elem            | 26 Fe    | 9.38E-01 | 9.36E-01 | 9.25E-01 | 9.05E-01 | 8.46E-01 |
| isot            | 26 Fe 54 | 2.94E-05 | 1.19E-03 | 6.30E-03 | 1.67E-02 | 5.78E-02 |
| isot            | 26 Fe 56 | 9.28E-01 | 9.22E-01 | 9.02E-01 | 8.65E-01 | 7.53E-01 |
| isot            | 26 Fe 57 | 9.69E-03 | 1.32E-02 | 1.69E-02 | 2.29E-02 | 3.45E-02 |
| isot            | 26 Fe 58 | 8.01E-10 | 9.80E-09 | 2.94E-08 | 9.18E-08 | 6.58E-07 |
| elem            | 27 Co    | 1.10E-03 | 2.21E-04 | 5.58E-04 | 8.08E-04 | 8.95E-04 |
| isot            | 27 Co 59 | 1.10E-03 | 2.21E-04 | 5.58E-04 | 8.08E-04 | 8.95E-04 |
| elem            | 28 Ni    | 1.43E-02 | 1.54E-02 | 2.71E-02 | 5.35E-02 | 1.40E-01 |
| isot            | 28 Ni 58 | 2.49E-03 | 2.88E-03 | 1.52E-02 | 4.21E-02 | 1.31E-01 |
| isot            | 28 Ni 60 | 1.16E-02 | 1.19E-02 | 1.03E-02 | 8.15E-03 | 3.87E-03 |
| isot            | 28 Ni 61 | 1.53E-04 | 2.46E-04 | 3.02E-04 | 3.44E-04 | 3.00E-04 |
| isot            | 28 Ni 62 | 1.01E-04 | 4.04E-04 | 1.39E-03 | 2.93E-03 | 5.11E-03 |
| isot            | 28 Ni 64 | 8.64E-12 | 2.06E-09 | 2.97E-08 | 1.79E-07 | 1.02E-06 |
| elem            | 29 Cu    | 9.08E-05 | 1.48E-05 | 2.13E-06 | 3.23E-06 | 5.24E-06 |
| isot            | 29 Cu 63 | 9.04E-05 | 1.40E-05 | 1.06E-06 | 1.83E-06 | 3.43E-06 |
| isot            | 29 Cu 65 | 4.26E-07 | 7.90E-07 | 1.06E-06 | 1.40E-06 | 1.82E-06 |
| elem            | 30 Zn    | 2.49E-04 | 1.41E-04 | 6.00E-05 | 6.88E-05 | 6.48E-05 |
| isot            | 30 Zn 64 | 2.42E-04 | 1.32E-04 | 3.74E-05 | 2.42E-05 | 8.34E-06 |
| isot            | 30 Zn 66 | 2.54E-06 | 8.25E-06 | 2.25E-05 | 4.40E-05 | 5.53E-05 |
| isot            | 30 Zn 67 | 8.94E-07 | 5.24E-08 | 3.87E-08 | 9.93E-08 | 2.11E-07 |
| isot            | 30 Zn 68 | 2.81E-06 | 2.60E-07 | 1.10E-07 | 5.49E-07 | 9.36E-07 |
| isot            | 30 Zn 70 | 2.19E-12 | 5.96E-11 | 9.21E-10 | 6.49E-09 | 1.67E-08 |
| elem            | 31 Ga    | 2.98E-09 | 1.21E-08 | 7.44E-08 | 3.08E-07 | 1.78E-07 |
| isot            | 31 Ga 69 | 1.60E-09 | 1.07E-08 | 5.76E-08 | 2.33E-07 | 1.26E-07 |
| isot            | 31 Ga 71 | 1.37E-09 | 1.45E-09 | 1.67E-08 | 7.46E-08 | 5.20E-08 |
| elem            | 32 Ge    | 1.07E-07 | 3.20E-07 | 1.57E-06 | 3.35E-06 | 8.85E-07 |
| isot            | 32 Ge 70 | 8.22E-08 | 2.83E-07 | 1.11E-06 | 1.88E-06 | 5.94E-07 |
| isot            | 32 Ge 72 | 2.49E-08 | 3.45E-08 | 4.30E-07 | 1.39E-06 | 2.68E-07 |
| isot            | 32 Ge 73 | 6.65E-11 | 1.97E-09 | 1.78E-08 | 2.09E-08 | 4.36E-09 |
| isot            | 32 Ge 74 | 2.60E-12 | 9.91E-11 | 5.44E-09 | 5.21E-08 | 1.78E-08 |
| isot            | 32 Ge 76 | 1.48E-12 | 7.95E-12 | 2.98E-10 | 1.40E-09 | 9.26E-10 |
| elem            | 33 As    | 1.19E-11 | 2.43E-09 | 2.33E-08 | 8.11E-08 | 1.03E-08 |
| isot            | 33 As 75 | 1.19E-11 | 2.43E-09 | 2.33E-08 | 8.11E-08 | 1.03E-08 |
| elem            | 34 Se    | 2.31E-09 | 1.98E-07 | 1.59E-06 | 2.07E-06 | 7.19E-08 |
| isot            | 34 Se 74 | 1.68E-09 | 1.13E-07 | 5.93E-07 | 7.79E-07 | 2.86E-08 |
| isot            | 34 Se 76 | 5.49E-10 | 8.39E-08 | 9.47E-07 | 1.18E-06 | 3.73E-08 |
| isot            | 34 Se 77 | 7.17E-11 | 1.05E-09 | 7.86E-09 | 1.17E-08 | 1.71E-09 |
| isot            | 34 Se 78 | 2.60E-12 | 5.89E-10 | 4.01E-08 | 9.63E-08 | 3.55E-09 |
| isot            | 34 Se 80 | 3.47E-12 | 2.09E-11 | 9.06E-10 | 2.67E-09 | 7.33E-10 |
| elem            | 35 Br    | 1.72E-11 | 2.78E-09 | 2.53E-08 | 2.26E-08 | 4.96E-10 |
| isot            | 35 Br 79 | 1.72E-11 | 2.78E-09 | 2.53E-08 | 2.26E-08 | 4.96E-10 |
| elem            | 36 Kr    | 1.30E-09 | 1.35E-07 | 8.66E-07 | 4.22E-07 | 2.70E-09 |
| isot            | 36 Kr 78 | 9.76E-10 | 4.72E-08 | 1.75E-07 | 8.79E-08 | 5.25E-10 |
| isot            | 36 Kr 80 | 3.19E-10 | 8.75E-08 | 6.91E-07 | 3.34E-07 | 2.18E-09 |

Table 5. Radioactivities with half-life longer than one day in Chandrasekhar-mass DDT models with  $\xi_{\text{CO}} = 0.9$ .

|                     |          |          |          |          |          |          |          |          |          |          |
|---------------------|----------|----------|----------|----------|----------|----------|----------|----------|----------|----------|
| $\rho_{\text{DDT}}$ | 1.2E+07  | 1.2E+07  | 1.2E+07  | 1.2E+07  | 1.2E+07  | 1.6E+07  | 1.6E+07  | 1.6E+07  | 1.6E+07  | 1.6E+07  |
| Z                   | 2.25E-4  | 2.25E-3  | 9.00E-3  | 2.25E-2  | 6.75E-2  | 2.25E-4  | 2.25E-3  | 9.00E-3  | 2.25E-2  | 6.75E-2  |
| Al26                | 1.07E-07 | 2.87E-07 | 3.99E-07 | 6.63E-07 | 1.18E-06 | 8.41E-08 | 1.48E-07 | 2.07E-07 | 3.31E-07 | 5.10E-07 |
| P 32                | 1.97E-10 | 2.48E-08 | 1.36E-07 | 5.23E-07 | 4.89E-06 | 1.28E-10 | 1.66E-08 | 8.86E-08 | 3.28E-07 | 2.71E-06 |
| P 33                | 8.11E-11 | 1.86E-08 | 1.26E-07 | 4.90E-07 | 3.81E-06 | 4.74E-11 | 1.11E-08 | 7.68E-08 | 3.00E-07 | 2.19E-06 |
| S 35                | 2.46E-11 | 6.29E-09 | 7.54E-08 | 7.20E-07 | 1.11E-05 | 1.47E-11 | 4.07E-09 | 4.86E-08 | 4.48E-07 | 6.34E-06 |
| Ar37                | 6.52E-06 | 1.17E-05 | 2.47E-05 | 4.01E-05 | 6.09E-05 | 4.55E-06 | 8.71E-06 | 1.78E-05 | 2.87E-05 | 4.48E-05 |
| Ca41                | 9.76E-07 | 2.19E-06 | 5.51E-06 | 9.45E-06 | 1.31E-05 | 8.78E-07 | 1.77E-06 | 4.18E-06 | 6.92E-06 | 9.82E-06 |
| Ti44                | 4.31E-05 | 3.69E-05 | 3.14E-05 | 2.56E-05 | 1.54E-05 | 4.42E-05 | 3.96E-05 | 3.45E-05 | 2.92E-05 | 1.95E-05 |
| V 48                | 5.32E-04 | 4.97E-04 | 4.43E-04 | 3.51E-04 | 2.01E-04 | 6.81E-04 | 6.53E-04 | 5.89E-04 | 5.02E-04 | 3.36E-04 |
| V 49                | 9.74E-06 | 1.33E-05 | 2.11E-05 | 2.82E-05 | 3.09E-05 | 8.09E-06 | 1.52E-05 | 2.39E-05 | 3.32E-05 | 4.05E-05 |
| Cr51                | 8.37E-06 | 1.83E-05 | 4.76E-05 | 8.39E-05 | 1.34E-04 | 1.04E-05 | 2.21E-05 | 5.84E-05 | 1.01E-04 | 1.66E-04 |
| Mn52                | 9.66E-03 | 9.07E-03 | 8.27E-03 | 6.57E-03 | 4.21E-03 | 1.52E-02 | 1.47E-02 | 1.32E-02 | 1.15E-02 | 8.50E-03 |
| Mn53                | 4.83E-04 | 6.01E-04 | 8.69E-04 | 1.10E-03 | 1.31E-03 | 5.47E-04 | 7.54E-04 | 1.10E-03 | 1.48E-03 | 1.97E-03 |
| Mn54                | 7.56E-06 | 7.60E-06 | 7.80E-06 | 8.27E-06 | 9.75E-06 | 7.47E-06 | 7.51E-06 | 7.71E-06 | 8.16E-06 | 9.59E-06 |
| Fe55                | 3.07E-03 | 4.44E-03 | 6.45E-03 | 8.43E-03 | 1.13E-02 | 3.33E-03 | 5.28E-03 | 8.09E-03 | 1.12E-02 | 1.68E-02 |
| Fe59                | 2.68E-06 | 2.93E-06 | 3.57E-06 | 4.92E-06 | 1.16E-05 | 2.74E-06 | 2.88E-06 | 3.27E-06 | 4.11E-06 | 7.89E-06 |
| Fe60                | 2.08E-05 | 2.19E-05 | 2.70E-05 | 4.08E-05 | 1.43E-04 | 2.09E-05 | 2.17E-05 | 2.53E-05 | 3.48E-05 | 9.62E-05 |
| Co56                | 7.13E-05 | 7.29E-05 | 7.53E-05 | 7.80E-05 | 1.09E-04 | 9.33E-05 | 9.77E-05 | 9.85E-05 | 1.04E-04 | 1.43E-04 |
| Co57                | 6.60E-04 | 6.65E-04 | 6.74E-04 | 6.97E-04 | 7.86E-04 | 6.50E-04 | 6.53E-04 | 6.63E-04 | 6.83E-04 | 7.81E-04 |
| Co58                | 4.00E-06 | 4.03E-06 | 4.11E-06 | 4.23E-06 | 4.70E-06 | 3.99E-06 | 4.01E-06 | 4.07E-06 | 4.25E-06 | 4.76E-06 |
| Co60                | 7.34E-07 | 9.77E-07 | 1.97E-06 | 3.40E-06 | 7.38E-06 | 7.20E-07 | 8.23E-07 | 1.23E-06 | 1.96E-06 | 4.39E-06 |
| Ni56                | 3.16E-01 | 3.03E-01 | 2.93E-01 | 2.50E-01 | 1.88E-01 | 5.17E-01 | 5.10E-01 | 4.76E-01 | 4.34E-01 | 3.66E-01 |
| Ni57                | 3.57E-03 | 3.99E-03 | 4.97E-03 | 5.89E-03 | 7.01E-03 | 4.15E-03 | 4.72E-03 | 6.06E-03 | 7.65E-03 | 1.03E-02 |
| Ni59                | 2.60E-04 | 2.45E-04 | 2.56E-04 | 2.57E-04 | 2.47E-04 | 2.86E-04 | 2.70E-04 | 2.80E-04 | 2.85E-04 | 2.85E-04 |
| Zn65                | 1.94E-08 | 4.56E-07 | 2.64E-06 | 2.59E-06 | 6.74E-07 | 1.89E-08 | 3.10E-07 | 1.57E-06 | 1.56E-06 | 4.15E-07 |

---

Yields are given in solar masses.

Table 5 *continued.*

|                     |          |          |          |          |          |          |          |          |          |          |
|---------------------|----------|----------|----------|----------|----------|----------|----------|----------|----------|----------|
| $\rho_{\text{DDT}}$ | 2.4E+07  | 2.4E+07  | 2.4E+07  | 2.4E+07  | 2.4E+07  | 2.8E+07  | 2.8E+07  | 2.8E+07  | 2.8E+07  | 2.8E+07  |
| Z                   | 2.25E-4  | 2.25E-3  | 9.00E-3  | 2.25E-2  | 6.75E-2  | 2.25E-4  | 2.25E-3  | 9.00E-3  | 2.25E-2  | 6.75E-2  |
| Al26                | 1.30E-07 | 7.80E-08 | 9.12E-08 | 1.31E-07 | 2.05E-07 | 6.24E-07 | 1.58E-07 | 6.94E-08 | 1.00E-07 | 1.54E-07 |
| P 32                | 6.90E-11 | 9.02E-09 | 4.78E-08 | 1.64E-07 | 1.33E-06 | 5.54E-11 | 7.73E-09 | 3.78E-08 | 1.32E-07 | 1.04E-06 |
| P 33                | 2.64E-11 | 5.54E-09 | 3.87E-08 | 1.45E-07 | 1.11E-06 | 2.29E-11 | 4.47E-09 | 2.90E-08 | 1.12E-07 | 8.59E-07 |
| S 35                | 9.20E-12 | 2.45E-09 | 2.76E-08 | 2.24E-07 | 3.10E-06 | 8.23E-12 | 2.09E-09 | 2.24E-08 | 1.81E-07 | 2.42E-06 |
| Ar37                | 3.50E-06 | 6.93E-06 | 1.34E-05 | 2.14E-05 | 3.46E-05 | 3.17E-06 | 6.43E-06 | 1.21E-05 | 1.95E-05 | 3.15E-05 |
| Ca41                | 8.43E-07 | 1.56E-06 | 3.27E-06 | 5.32E-06 | 7.83E-06 | 7.97E-07 | 1.48E-06 | 3.03E-06 | 4.92E-06 | 7.25E-06 |
| Ti44                | 3.87E-05 | 3.41E-05 | 3.00E-05 | 2.53E-05 | 1.67E-05 | 3.73E-05 | 3.46E-05 | 3.55E-05 | 2.81E-05 | 2.00E-05 |
| V 48                | 5.96E-04 | 5.71E-04 | 5.47E-04 | 4.59E-04 | 2.96E-04 | 5.37E-04 | 5.21E-04 | 4.81E-04 | 4.14E-04 | 2.71E-04 |
| V 49                | 5.94E-06 | 1.34E-05 | 2.18E-05 | 2.96E-05 | 3.56E-05 | 5.27E-06 | 1.23E-05 | 1.89E-05 | 2.65E-05 | 3.22E-05 |
| Cr51                | 1.12E-05 | 2.21E-05 | 5.73E-05 | 9.36E-05 | 1.50E-04 | 1.10E-05 | 2.09E-05 | 5.01E-05 | 8.47E-05 | 1.36E-04 |
| Mn52                | 1.54E-02 | 1.48E-02 | 1.50E-02 | 1.22E-02 | 8.44E-03 | 1.37E-02 | 1.33E-02 | 1.21E-02 | 1.07E-02 | 7.45E-03 |
| Mn53                | 5.06E-04 | 7.65E-04 | 1.21E-03 | 1.53E-03 | 1.97E-03 | 4.68E-04 | 7.15E-04 | 1.02E-03 | 1.38E-03 | 1.77E-03 |
| Mn54                | 7.34E-06 | 7.37E-06 | 7.45E-06 | 7.91E-06 | 9.11E-06 | 7.18E-06 | 7.21E-06 | 7.45E-06 | 7.75E-06 | 9.02E-06 |
| Fe55                | 3.30E-03 | 5.32E-03 | 9.36E-03 | 1.25E-02 | 1.91E-02 | 3.28E-03 | 5.08E-03 | 7.93E-03 | 1.14E-02 | 1.69E-02 |
| Fe59                | 2.82E-06 | 2.92E-06 | 3.17E-06 | 3.88E-06 | 6.59E-06 | 2.76E-06 | 2.85E-06 | 3.18E-06 | 3.74E-06 | 6.32E-06 |
| Fe60                | 2.07E-05 | 2.14E-05 | 2.46E-05 | 3.14E-05 | 7.16E-05 | 2.10E-05 | 2.17E-05 | 2.44E-05 | 3.12E-05 | 6.75E-05 |
| Co56                | 1.21E-04 | 1.25E-04 | 1.28E-04 | 1.33E-04 | 1.68E-04 | 1.27E-04 | 1.31E-04 | 1.33E-04 | 1.38E-04 | 1.66E-04 |
| Co57                | 6.46E-04 | 6.49E-04 | 6.56E-04 | 6.77E-04 | 7.60E-04 | 6.42E-04 | 6.48E-04 | 6.57E-04 | 6.74E-04 | 7.56E-04 |
| Co58                | 3.87E-06 | 3.88E-06 | 3.94E-06 | 4.08E-06 | 4.54E-06 | 3.81E-06 | 3.83E-06 | 3.91E-06 | 4.03E-06 | 4.45E-06 |
| Co60                | 7.11E-07 | 7.51E-07 | 8.92E-07 | 1.17E-06 | 2.40E-06 | 7.02E-07 | 7.35E-07 | 8.53E-07 | 1.07E-06 | 2.07E-06 |
| Ni56                | 7.50E-01 | 7.43E-01 | 7.04E-01 | 6.63E-01 | 5.49E-01 | 8.04E-01 | 7.94E-01 | 7.65E-01 | 7.21E-01 | 5.95E-01 |
| Ni57                | 5.52E-03 | 7.11E-03 | 7.95E-03 | 1.21E-02 | 1.76E-02 | 6.47E-03 | 8.75E-03 | 1.15E-02 | 1.50E-02 | 2.16E-02 |
| Ni59                | 5.98E-04 | 2.82E-04 | 2.81E-04 | 3.65E-04 | 3.24E-04 | 9.94E-04 | 2.94E-04 | 4.50E-04 | 5.50E-04 | 7.19E-04 |
| Zn65                | 3.16E-08 | 2.21E-07 | 7.04E-07 | 7.44E-07 | 2.54E-07 | 1.02E-07 | 4.51E-07 | 9.71E-07 | 9.70E-07 | 8.39E-07 |

Table 5 *continued.*

|                     |          |          |          |          |          |
|---------------------|----------|----------|----------|----------|----------|
| $\rho_{\text{DDT}}$ | 4.0E+07  | 4.0E+07  | 4.0E+07  | 4.0E+07  | 4.0E+07  |
| Z                   | 2.25E-4  | 2.25E-3  | 9.00E-3  | 2.25E-2  | 6.75E-2  |
| Al26                | 1.55E-06 | 1.68E-07 | 3.72E-08 | 5.15E-08 | 7.05E-08 |
| P 32                | 3.14E-11 | 4.60E-09 | 2.26E-08 | 7.45E-08 | 5.54E-07 |
| P 33                | 1.84E-11 | 2.38E-09 | 1.56E-08 | 6.02E-08 | 4.66E-07 |
| S 35                | 6.11E-12 | 1.25E-09 | 1.40E-08 | 1.12E-07 | 1.38E-06 |
| Ar37                | 2.24E-06 | 4.79E-06 | 9.06E-06 | 1.46E-05 | 2.34E-05 |
| Ca41                | 6.49E-07 | 1.17E-06 | 2.36E-06 | 3.84E-06 | 5.54E-06 |
| Ti44                | 4.20E-05 | 4.96E-05 | 5.11E-05 | 4.31E-05 | 2.53E-05 |
| V 48                | 4.23E-04 | 4.24E-04 | 3.96E-04 | 3.44E-04 | 2.20E-04 |
| V 49                | 3.99E-06 | 9.82E-06 | 1.50E-05 | 2.10E-05 | 2.55E-05 |
| Cr51                | 1.09E-05 | 1.82E-05 | 4.15E-05 | 6.92E-05 | 1.09E-04 |
| Mn52                | 1.04E-02 | 1.01E-02 | 9.31E-03 | 8.29E-03 | 5.75E-03 |
| Mn53                | 3.82E-04 | 6.05E-04 | 8.39E-04 | 1.13E-03 | 1.43E-03 |
| Mn54                | 7.18E-06 | 7.21E-06 | 7.41E-06 | 7.70E-06 | 8.82E-06 |
| Fe55                | 3.24E-03 | 4.59E-03 | 6.85E-03 | 9.59E-03 | 1.41E-02 |
| Fe59                | 2.81E-06 | 2.88E-06 | 3.16E-06 | 3.64E-06 | 5.80E-06 |
| Fe60                | 2.10E-05 | 2.17E-05 | 2.43E-05 | 3.02E-05 | 5.97E-05 |
| Co56                | 1.40E-04 | 1.43E-04 | 1.45E-04 | 1.48E-04 | 1.68E-04 |
| Co57                | 6.45E-04 | 6.49E-04 | 6.56E-04 | 6.76E-04 | 7.45E-04 |
| Co58                | 3.80E-06 | 3.82E-06 | 3.88E-06 | 4.00E-06 | 4.37E-06 |
| Co60                | 7.01E-07 | 7.20E-07 | 7.81E-07 | 8.92E-07 | 1.47E-06 |
| Ni56                | 9.09E-01 | 9.02E-01 | 8.72E-01 | 8.24E-01 | 6.89E-01 |
| Ni57                | 8.55E-03 | 1.23E-02 | 1.56E-02 | 2.01E-02 | 2.91E-02 |
| Ni59                | 1.61E-03 | 3.29E-04 | 6.65E-04 | 9.20E-04 | 1.27E-03 |
| Zn65                | 3.53E-07 | 1.56E-06 | 1.73E-06 | 2.03E-06 | 1.84E-06 |



Table 6. Radioactivities with half-life longer than one day in sub-Chandrasekhar models with  $\xi_{\text{CO}} = 0.9$ .

| $M_{\text{WD}}$ | 0.88     | 0.88     | 0.88     | 0.88     | 0.88     | 0.97     | 0.97     | 0.97     | 0.97     | 0.97     |
|-----------------|----------|----------|----------|----------|----------|----------|----------|----------|----------|----------|
| Z               | 2.25E-4  | 2.25E-3  | 9.00E-3  | 2.25E-2  | 6.75E-2  | 2.25E-4  | 2.25E-3  | 9.00E-3  | 2.25E-2  | 6.75E-2  |
| Al26            | 7.78E-08 | 2.03E-07 | 2.80E-07 | 4.27E-07 | 6.16E-07 | 4.06E-08 | 7.53E-08 | 1.02E-07 | 1.46E-07 | 1.92E-07 |
| P 32            | 1.47E-10 | 1.96E-08 | 1.06E-07 | 3.82E-07 | 2.98E-06 | 7.04E-11 | 9.88E-09 | 4.99E-08 | 1.68E-07 | 1.18E-06 |
| P 33            | 5.44E-11 | 1.46E-08 | 9.79E-08 | 3.61E-07 | 2.42E-06 | 2.68E-11 | 6.24E-09 | 4.03E-08 | 1.48E-07 | 9.83E-07 |
| S 35            | 1.83E-11 | 4.98E-09 | 5.64E-08 | 4.94E-07 | 6.51E-06 | 8.28E-12 | 2.70E-09 | 2.88E-08 | 2.30E-07 | 2.77E-06 |
| Ar37            | 5.63E-06 | 9.53E-06 | 1.93E-05 | 2.97E-05 | 4.42E-05 | 4.24E-06 | 7.82E-06 | 1.46E-05 | 2.29E-05 | 3.47E-05 |
| Ca41            | 8.23E-07 | 1.88E-06 | 4.49E-06 | 7.07E-06 | 9.58E-06 | 9.39E-07 | 1.79E-06 | 3.61E-06 | 5.71E-06 | 7.96E-06 |
| Ti44            | 2.93E-05 | 2.52E-05 | 2.15E-05 | 1.80E-05 | 1.17E-05 | 3.19E-05 | 2.78E-05 | 2.40E-05 | 2.02E-05 | 1.33E-05 |
| V 48            | 3.74E-04 | 3.49E-04 | 3.08E-04 | 2.59E-04 | 1.76E-04 | 4.72E-04 | 4.52E-04 | 4.09E-04 | 3.50E-04 | 2.22E-04 |
| V 49            | 6.48E-06 | 8.62E-06 | 1.38E-05 | 1.91E-05 | 2.34E-05 | 7.24E-06 | 1.04E-05 | 1.64E-05 | 2.28E-05 | 2.71E-05 |
| Cr51            | 2.62E-06 | 1.14E-05 | 3.24E-05 | 5.79E-05 | 1.01E-04 | 2.30E-06 | 1.47E-05 | 4.00E-05 | 7.01E-05 | 1.14E-04 |
| Mn52            | 7.48E-03 | 7.05E-03 | 6.31E-03 | 5.49E-03 | 4.24E-03 | 1.18E-02 | 1.14E-02 | 1.04E-02 | 9.08E-03 | 6.21E-03 |
| Mn53            | 2.16E-04 | 2.97E-04 | 4.89E-04 | 6.91E-04 | 9.81E-04 | 3.23E-04 | 4.41E-04 | 7.15E-04 | 1.01E-03 | 1.32E-03 |
| Mn54            | 6.69E-11 | 2.99E-09 | 3.24E-08 | 1.93E-07 | 7.53E-07 | 2.71E-11 | 1.89E-09 | 1.78E-08 | 1.03E-07 | 5.50E-07 |
| Fe55            | 1.94E-04 | 1.19E-03 | 2.68E-03 | 4.37E-03 | 7.36E-03 | 1.93E-04 | 1.80E-03 | 4.24E-03 | 7.01E-03 | 1.13E-02 |
| Fe59            | 6.77E-10 | 1.56E-07 | 4.72E-07 | 1.10E-06 | 3.73E-06 | 3.30E-10 | 5.55E-08 | 1.66E-07 | 4.19E-07 | 1.51E-06 |
| Fe60            | 9.17E-11 | 2.79E-07 | 2.27E-06 | 7.85E-06 | 5.30E-05 | 4.96E-11 | 1.13E-07 | 8.52E-07 | 2.93E-06 | 1.89E-05 |
| Co56            | 2.15E-05 | 2.15E-05 | 2.25E-05 | 2.70E-05 | 5.27E-05 | 5.10E-05 | 5.28E-05 | 5.45E-05 | 5.99E-05 | 8.70E-05 |
| Co57            | 3.59E-07 | 8.09E-07 | 2.91E-06 | 9.56E-06 | 5.61E-05 | 8.44E-07 | 1.48E-06 | 3.75E-06 | 1.01E-05 | 5.05E-05 |
| Co58            | 5.72E-09 | 1.23E-08 | 2.69E-08 | 6.30E-08 | 2.51E-07 | 1.86E-09 | 3.99E-09 | 1.22E-08 | 3.55E-08 | 1.71E-07 |
| Co60            | 7.16E-10 | 1.61E-07 | 8.05E-07 | 1.68E-06 | 3.85E-06 | 3.12E-10 | 5.05E-08 | 2.21E-07 | 4.86E-07 | 1.41E-06 |
| Ni56            | 1.91E-01 | 1.82E-01 | 1.69E-01 | 1.55E-01 | 1.39E-01 | 4.57E-01 | 4.49E-01 | 4.33E-01 | 4.12E-01 | 3.63E-01 |
| Ni57            | 5.68E-04 | 7.98E-04 | 1.37E-03 | 2.05E-03 | 3.25E-03 | 1.63E-03 | 2.36E-03 | 3.83E-03 | 5.99E-03 | 1.09E-02 |
| Ni59            | 4.43E-07 | 1.38E-06 | 1.42E-06 | 3.51E-06 | 1.48E-05 | 8.46E-05 | 1.10E-05 | 2.67E-05 | 5.20E-05 | 1.37E-04 |
| Zn65            | 5.27E-09 | 3.33E-07 | 1.78E-06 | 1.65E-06 | 4.03E-07 | 8.55E-09 | 1.73E-07 | 7.35E-07 | 7.01E-07 | 2.60E-07 |

Table 6 continued.

| $M_{\text{WD}}$ | 1.06     | 1.06     | 1.06     | 1.06     | 1.06     | 1.10     | 1.10     | 1.10     | 1.10     | 1.10     |
|-----------------|----------|----------|----------|----------|----------|----------|----------|----------|----------|----------|
| Z               | 2.25E-4  | 2.25E-3  | 9.00E-3  | 2.25E-2  | 6.75E-2  | 2.25E-4  | 2.25E-3  | 9.00E-3  | 2.25E-2  | 6.75E-2  |
| Al26            | 1.46E-06 | 3.49E-08 | 3.75E-08 | 5.07E-08 | 6.05E-08 | 1.35E-06 | 5.37E-08 | 2.32E-08 | 3.08E-08 | 3.57E-08 |
| P 32            | 3.48E-11 | 4.46E-09 | 2.10E-08 | 6.74E-08 | 4.27E-07 | 2.40E-11 | 2.90E-09 | 1.32E-08 | 4.16E-08 | 2.57E-07 |
| P 33            | 1.51E-11 | 2.31E-09 | 1.45E-08 | 5.34E-08 | 3.52E-07 | 1.15E-11 | 1.37E-09 | 8.47E-09 | 3.14E-08 | 2.07E-07 |
| S 35            | 4.11E-12 | 1.26E-09 | 1.36E-08 | 1.03E-07 | 1.09E-06 | 3.11E-12 | 8.58E-10 | 9.42E-09 | 6.95E-08 | 6.94E-07 |
| Ar37            | 2.54E-06 | 5.25E-06 | 9.68E-06 | 1.51E-05 | 2.25E-05 | 1.81E-06 | 4.01E-06 | 7.37E-06 | 1.15E-05 | 1.68E-05 |
| Ca41            | 7.16E-07 | 1.32E-06 | 2.56E-06 | 3.99E-06 | 5.37E-06 | 5.76E-07 | 1.05E-06 | 2.02E-06 | 3.12E-06 | 4.09E-06 |
| Ti44            | 3.39E-05 | 2.99E-05 | 2.92E-05 | 2.37E-05 | 1.28E-05 | 3.27E-05 | 2.97E-05 | 2.95E-05 | 2.35E-05 | 1.21E-05 |
| V 48            | 3.86E-04 | 3.75E-04 | 3.43E-04 | 2.93E-04 | 1.83E-04 | 3.38E-04 | 3.30E-04 | 3.03E-04 | 2.59E-04 | 1.60E-04 |
| V 49            | 4.35E-06 | 8.66E-06 | 1.34E-05 | 1.87E-05 | 2.22E-05 | 3.29E-06 | 7.69E-06 | 1.18E-05 | 1.64E-05 | 1.94E-05 |
| Cr51            | 3.25E-06 | 1.18E-05 | 3.29E-05 | 5.75E-05 | 9.25E-05 | 3.56E-06 | 1.03E-05 | 2.88E-05 | 5.03E-05 | 8.06E-05 |
| Mn52            | 9.52E-03 | 9.21E-03 | 8.46E-03 | 7.37E-03 | 4.96E-03 | 8.23E-03 | 7.97E-03 | 7.33E-03 | 6.38E-03 | 4.30E-03 |
| Mn53            | 2.32E-04 | 3.68E-04 | 5.85E-04 | 8.28E-04 | 1.07E-03 | 1.79E-04 | 3.25E-04 | 5.10E-04 | 7.20E-04 | 9.37E-04 |
| Mn54            | 1.33E-11 | 9.70E-10 | 9.06E-09 | 5.33E-08 | 3.68E-07 | 9.20E-12 | 6.78E-10 | 6.54E-09 | 3.84E-08 | 2.84E-07 |
| Fe55            | 9.15E-05 | 1.42E-03 | 3.46E-03 | 5.75E-03 | 9.20E-03 | 8.50E-05 | 1.21E-03 | 3.00E-03 | 5.00E-03 | 8.80E-03 |
| Fe59            | 1.46E-10 | 2.01E-08 | 6.04E-08 | 1.58E-07 | 6.09E-07 | 9.62E-11 | 1.23E-08 | 3.78E-08 | 1.00E-07 | 3.88E-07 |
| Fe60            | 2.41E-11 | 4.77E-08 | 3.54E-07 | 1.20E-06 | 6.81E-06 | 1.60E-11 | 3.06E-08 | 2.32E-07 | 7.92E-07 | 4.28E-06 |
| Co56            | 7.94E-05 | 8.22E-05 | 8.37E-05 | 8.69E-05 | 1.04E-04 | 9.28E-05 | 9.55E-05 | 9.67E-05 | 9.88E-05 | 1.16E-04 |
| Co57            | 2.52E-06 | 4.09E-06 | 6.51E-06 | 1.25E-05 | 4.34E-05 | 3.55E-06 | 5.34E-06 | 7.81E-06 | 1.35E-05 | 4.02E-05 |
| Co58            | 6.99E-10 | 1.49E-09 | 5.79E-09 | 2.01E-08 | 1.08E-07 | 4.42E-10 | 9.55E-10 | 4.07E-09 | 1.51E-08 | 8.25E-08 |
| Co60            | 1.40E-10 | 1.90E-08 | 6.60E-08 | 1.45E-07 | 4.67E-07 | 9.33E-11 | 1.23E-08 | 4.01E-08 | 8.53E-08 | 2.75E-07 |
| Ni56            | 7.06E-01 | 6.99E-01 | 6.80E-01 | 6.50E-01 | 5.69E-01 | 8.07E-01 | 8.01E-01 | 7.81E-01 | 7.48E-01 | 6.53E-01 |
| Ni57            | 5.02E-03 | 7.71E-03 | 1.02E-02 | 1.43E-02 | 2.33E-02 | 6.99E-03 | 1.02E-02 | 1.32E-02 | 1.81E-02 | 2.86E-02 |
| Ni59            | 7.33E-04 | 8.87E-05 | 2.96E-04 | 4.74E-04 | 6.60E-04 | 9.10E-04 | 1.37E-04 | 4.20E-04 | 6.51E-04 | 8.12E-04 |
| Zn65            | 2.89E-07 | 5.30E-07 | 8.42E-07 | 9.07E-07 | 4.99E-07 | 3.76E-07 | 6.65E-07 | 9.25E-07 | 1.00E-06 | 5.63E-07 |

Table 6 *continued.*

| $M_{\text{WD}}$ | 1.15     | 1.15     | 1.15     | 1.15     | 1.15     |
|-----------------|----------|----------|----------|----------|----------|
| Z               | 2.25E-4  | 2.25E-3  | 9.00E-3  | 2.25E-2  | 6.75E-2  |
| Al26            | 9.18E-07 | 1.33E-07 | 1.22E-08 | 1.60E-08 | 1.79E-08 |
| P 32            | 1.50E-11 | 1.51E-09 | 6.77E-09 | 2.14E-08 | 1.30E-07 |
| P 33            | 8.16E-12 | 6.43E-10 | 4.07E-09 | 1.53E-08 | 1.02E-07 |
| S 35            | 2.19E-12 | 4.93E-10 | 5.61E-09 | 4.08E-08 | 3.81E-07 |
| Ar37            | 1.08E-06 | 2.64E-06 | 4.80E-06 | 7.48E-06 | 1.08E-05 |
| Ca41            | 4.05E-07 | 7.17E-07 | 1.35E-06 | 2.08E-06 | 2.70E-06 |
| Ti44            | 2.97E-05 | 2.81E-05 | 2.84E-05 | 2.24E-05 | 1.10E-05 |
| V 48            | 2.72E-04 | 2.69E-04 | 2.49E-04 | 2.12E-04 | 1.31E-04 |
| V 49            | 2.27E-06 | 6.36E-06 | 9.56E-06 | 1.33E-05 | 1.58E-05 |
| Cr51            | 3.51E-06 | 8.19E-06 | 2.32E-05 | 4.05E-05 | 6.55E-05 |
| Mn52            | 6.55E-03 | 6.36E-03 | 5.85E-03 | 5.10E-03 | 3.57E-03 |
| Mn53            | 1.16E-04 | 2.67E-04 | 4.11E-04 | 5.78E-04 | 8.04E-04 |
| Mn54            | 5.40E-12 | 3.81E-10 | 4.07E-09 | 2.42E-08 | 1.90E-07 |
| Fe55            | 8.71E-05 | 9.46E-04 | 2.40E-03 | 4.00E-03 | 9.67E-03 |
| Fe59            | 5.62E-11 | 6.60E-09 | 2.11E-08 | 5.66E-08 | 2.15E-07 |
| Fe60            | 9.57E-12 | 1.67E-08 | 1.31E-07 | 4.57E-07 | 2.32E-06 |
| Co56            | 1.10E-04 | 1.12E-04 | 1.13E-04 | 1.14E-04 | 1.37E-04 |
| Co57            | 5.00E-06 | 6.94E-06 | 9.51E-06 | 1.47E-05 | 3.68E-05 |
| Co58            | 2.32E-10 | 5.20E-10 | 2.50E-09 | 9.87E-09 | 5.52E-08 |
| Co60            | 5.31E-11 | 6.66E-09 | 2.11E-08 | 4.31E-08 | 1.36E-07 |
| Ni56            | 9.28E-01 | 9.22E-01 | 9.01E-01 | 8.65E-01 | 7.53E-01 |
| Ni57            | 9.69E-03 | 1.32E-02 | 1.69E-02 | 2.28E-02 | 3.45E-02 |
| Ni59            | 1.10E-03 | 2.21E-04 | 5.58E-04 | 8.08E-04 | 8.94E-04 |
| Zn65            | 4.26E-07 | 7.86E-07 | 1.00E-06 | 1.07E-06 | 6.38E-07 |

Table A1. Nucleosynthesis in Chandrasekhar-mass DDT models with the standard  $^{12}\text{C}+^{16}\text{O}$  reaction rate.

| $\rho_{\text{DDT}}$ |          | 1.2E+07  | 1.2E+07  | 1.2E+07  | 1.2E+07  | 1.2E+07  | 1.6E+07  | 1.6E+07  | 1.6E+07  | 1.6E+07  | 1.6E+07  |
|---------------------|----------|----------|----------|----------|----------|----------|----------|----------|----------|----------|----------|
| Z                   |          | 2.25E-4  | 2.25E-3  | 9.00E-3  | 2.25E-2  | 6.75E-2  | 2.25E-4  | 2.25E-3  | 9.00E-3  | 2.25E-2  | 6.75E-2  |
| elem                | 2 He     | 1.31E-04 | 1.22E-04 | 1.00E-04 | 4.64E-05 | 3.05E-08 | 1.32E-04 | 1.23E-04 | 1.01E-04 | 4.63E-05 | 3.18E-08 |
| isot                | 2 He 3   | 1.80E-12 | 1.78E-12 | 1.76E-12 | 1.62E-12 | 1.33E-12 | 1.80E-12 | 1.78E-12 | 1.76E-12 | 1.62E-12 | 1.33E-12 |
| isot                | 2 He 4   | 1.31E-04 | 1.22E-04 | 1.00E-04 | 4.64E-05 | 3.05E-08 | 1.32E-04 | 1.23E-04 | 1.01E-04 | 4.62E-05 | 3.18E-08 |
| elem                | 6 C      | 5.02E-03 | 4.94E-03 | 4.85E-03 | 5.16E-03 | 5.19E-03 | 2.40E-03 | 2.37E-03 | 2.55E-03 | 2.50E-03 | 2.40E-03 |
| isot                | 6 C 12   | 5.02E-03 | 4.94E-03 | 4.85E-03 | 5.16E-03 | 5.19E-03 | 2.40E-03 | 2.37E-03 | 2.55E-03 | 2.50E-03 | 2.40E-03 |
| isot                | 6 C 13   | 2.08E-10 | 3.58E-09 | 1.25E-08 | 3.02E-08 | 7.54E-08 | 1.06E-10 | 1.58E-09 | 6.48E-09 | 1.52E-08 | 3.90E-08 |
| elem                | 7 N      | 1.04E-05 | 8.68E-06 | 6.83E-06 | 5.52E-06 | 5.27E-06 | 9.73E-06 | 7.94E-06 | 6.00E-06 | 3.97E-06 | 2.29E-06 |
| isot                | 7 N 14   | 1.03E-05 | 8.67E-06 | 6.83E-06 | 5.51E-06 | 5.26E-06 | 9.65E-06 | 7.94E-06 | 6.00E-06 | 3.97E-06 | 2.29E-06 |
| isot                | 7 N 15   | 1.44E-07 | 4.58E-09 | 2.50E-09 | 3.92E-09 | 7.25E-09 | 7.38E-08 | 2.23E-09 | 1.24E-09 | 1.62E-09 | 2.61E-09 |
| elem                | 8 O      | 1.69E-01 | 1.69E-01 | 1.69E-01 | 1.79E-01 | 1.81E-01 | 1.07E-01 | 1.08E-01 | 1.16E-01 | 1.17E-01 | 1.14E-01 |
| isot                | 8 O 16   | 1.69E-01 | 1.69E-01 | 1.69E-01 | 1.79E-01 | 1.80E-01 | 1.07E-01 | 1.08E-01 | 1.16E-01 | 1.17E-01 | 1.14E-01 |
| isot                | 8 O 17   | 8.57E-09 | 1.17E-07 | 2.62E-07 | 4.26E-07 | 5.91E-07 | 4.30E-09 | 4.92E-08 | 1.17E-07 | 1.69E-07 | 2.03E-07 |
| isot                | 8 O 18   | 2.46E-09 | 1.90E-09 | 2.14E-09 | 3.06E-09 | 3.98E-09 | 1.05E-09 | 7.81E-10 | 9.56E-10 | 1.14E-09 | 1.25E-09 |
| elem                | 9 F      | 5.65E-11 | 1.43E-11 | 1.46E-11 | 3.85E-11 | 1.42E-10 | 2.21E-11 | 5.18E-12 | 6.32E-12 | 1.63E-11 | 6.10E-11 |
| isot                | 9 F 19   | 5.65E-11 | 1.43E-11 | 1.46E-11 | 3.85E-11 | 1.42E-10 | 2.21E-11 | 5.18E-12 | 6.32E-12 | 1.63E-11 | 6.10E-11 |
| elem                | 10 Ne    | 4.06E-03 | 3.96E-03 | 3.88E-03 | 4.16E-03 | 4.31E-03 | 1.75E-03 | 1.71E-03 | 1.86E-03 | 1.84E-03 | 1.82E-03 |
| isot                | 10 Ne 20 | 4.06E-03 | 3.96E-03 | 3.87E-03 | 4.12E-03 | 4.07E-03 | 1.75E-03 | 1.71E-03 | 1.86E-03 | 1.82E-03 | 1.70E-03 |
| isot                | 10 Ne 21 | 8.60E-09 | 4.89E-08 | 1.46E-07 | 3.88E-07 | 1.66E-06 | 3.72E-09 | 2.05E-08 | 6.97E-08 | 1.74E-07 | 7.19E-07 |
| isot                | 10 Ne 22 | 1.38E-07 | 2.01E-06 | 1.22E-05 | 4.72E-05 | 2.41E-04 | 8.23E-08 | 1.08E-06 | 6.55E-06 | 2.27E-05 | 1.11E-04 |
| elem                | 11 Na    | 2.43E-05 | 2.62E-05 | 3.22E-05 | 5.15E-05 | 1.24E-04 | 1.10E-05 | 1.15E-05 | 1.56E-05 | 2.33E-05 | 5.34E-05 |
| isot                | 11 Na 23 | 2.43E-05 | 2.62E-05 | 3.22E-05 | 5.15E-05 | 1.24E-04 | 1.10E-05 | 1.15E-05 | 1.56E-05 | 2.33E-05 | 5.34E-05 |
| elem                | 12 Mg    | 4.23E-02 | 3.75E-02 | 2.87E-02 | 2.14E-02 | 1.20E-02 | 2.40E-02 | 2.13E-02 | 1.72E-02 | 1.19E-02 | 6.47E-03 |
| isot                | 12 Mg 24 | 4.23E-02 | 3.75E-02 | 2.86E-02 | 2.12E-02 | 1.13E-02 | 2.40E-02 | 2.13E-02 | 1.72E-02 | 1.18E-02 | 6.16E-03 |
| isot                | 12 Mg 25 | 1.17E-06 | 1.21E-05 | 2.99E-05 | 7.96E-05 | 2.64E-04 | 6.02E-07 | 6.06E-06 | 1.55E-05 | 3.69E-05 | 1.12E-04 |
| isot                | 12 Mg 26 | 1.33E-06 | 9.15E-06 | 4.03E-05 | 1.16E-04 | 4.58E-04 | 5.93E-07 | 4.25E-06 | 2.08E-05 | 5.47E-05 | 2.00E-04 |
| elem                | 13 Al    | 1.21E-04 | 3.83E-04 | 7.41E-04 | 9.45E-04 | 9.48E-04 | 6.01E-05 | 2.06E-04 | 4.28E-04 | 5.03E-04 | 4.74E-04 |
| isot                | 13 Al 27 | 1.21E-04 | 3.83E-04 | 7.41E-04 | 9.45E-04 | 9.48E-04 | 6.01E-05 | 2.06E-04 | 4.28E-04 | 5.03E-04 | 4.74E-04 |
| elem                | 14 Si    | 4.35E-01 | 4.45E-01 | 4.52E-01 | 4.60E-01 | 4.37E-01 | 3.34E-01 | 3.41E-01 | 3.59E-01 | 3.55E-01 | 3.37E-01 |
| isot                | 14 Si 28 | 4.35E-01 | 4.44E-01 | 4.50E-01 | 4.56E-01 | 4.24E-01 | 3.34E-01 | 3.41E-01 | 3.58E-01 | 3.52E-01 | 3.30E-01 |
| isot                | 14 Si 29 | 1.66E-04 | 4.63E-04 | 7.07E-04 | 1.21E-03 | 2.99E-03 | 1.04E-04 | 2.99E-04 | 4.74E-04 | 7.39E-04 | 1.69E-03 |
| isot                | 14 Si 30 | 1.97E-05 | 1.86E-04 | 1.10E-03 | 2.92E-03 | 9.45E-03 | 1.13E-05 | 1.14E-04 | 7.00E-04 | 1.73E-03 | 5.56E-03 |
| elem                | 15 P     | 5.09E-05 | 1.24E-04 | 3.57E-04 | 7.17E-04 | 1.68E-03 | 3.81E-05 | 8.02E-05 | 2.36E-04 | 4.43E-04 | 1.01E-03 |
| isot                | 15 P 31  | 5.09E-05 | 1.24E-04 | 3.57E-04 | 7.17E-04 | 1.68E-03 | 3.81E-05 | 8.02E-05 | 2.36E-04 | 4.43E-04 | 1.01E-03 |
| elem                | 16 S     | 2.37E-01 | 2.35E-01 | 2.36E-01 | 2.32E-01 | 1.95E-01 | 1.98E-01 | 1.95E-01 | 1.99E-01 | 1.90E-01 | 1.57E-01 |
| isot                | 16 S 32  | 2.37E-01 | 2.34E-01 | 2.34E-01 | 2.27E-01 | 1.77E-01 | 1.98E-01 | 1.95E-01 | 1.98E-01 | 1.86E-01 | 1.45E-01 |
| isot                | 16 S 33  | 8.03E-05 | 1.47E-04 | 2.93E-04 | 4.60E-04 | 7.57E-04 | 4.76E-05 | 9.38E-05 | 1.99E-04 | 3.06E-04 | 5.19E-04 |
| isot                | 16 S 34  | 1.48E-06 | 3.12E-04 | 1.74E-03 | 5.06E-03 | 1.71E-02 | 1.15E-06 | 2.08E-04 | 1.25E-03 | 3.50E-03 | 1.17E-02 |
| isot                | 16 S 36  | 1.57E-10 | 7.14E-09 | 8.41E-08 | 5.52E-07 | 1.62E-05 | 1.34E-10 | 3.91E-09 | 4.67E-08 | 2.95E-07 | 8.42E-06 |
| elem                | 17 Cl    | 1.29E-05 | 3.64E-05 | 1.11E-04 | 2.53E-04 | 5.13E-04 | 1.07E-05 | 2.52E-05 | 7.87E-05 | 1.70E-04 | 3.45E-04 |
| isot                | 17 Cl 35 | 6.62E-06 | 2.55E-05 | 8.85E-05 | 2.14E-04 | 4.35E-04 | 6.55E-06 | 1.73E-05 | 6.19E-05 | 1.41E-04 | 2.90E-04 |
| isot                | 17 Cl 37 | 6.31E-06 | 1.09E-05 | 2.26E-05 | 3.89E-05 | 7.81E-05 | 4.11E-06 | 7.92E-06 | 1.68E-05 | 2.82E-05 | 5.49E-05 |
| elem                | 18 Ar    | 5.05E-02 | 4.84E-02 | 4.64E-02 | 4.33E-02 | 3.61E-02 | 4.58E-02 | 4.37E-02 | 4.25E-02 | 3.88E-02 | 3.15E-02 |
| isot                | 18 Ar 36 | 5.05E-02 | 4.83E-02 | 4.57E-02 | 4.10E-02 | 2.85E-02 | 4.58E-02 | 4.36E-02 | 4.20E-02 | 3.72E-02 | 2.63E-02 |
| isot                | 18 Ar 38 | 1.21E-06 | 1.20E-04 | 7.18E-04 | 2.25E-03 | 7.64E-03 | 7.33E-07 | 7.56E-05 | 5.00E-04 | 1.55E-03 | 5.17E-03 |
| isot                | 18 Ar 40 | 3.33E-11 | 1.60E-09 | 2.11E-08 | 1.16E-07 | 1.33E-06 | 2.06E-11 | 7.04E-10 | 1.02E-08 | 5.15E-08 | 6.10E-07 |
| elem                | 19 K     | 3.51E-06 | 2.04E-05 | 6.33E-05 | 1.29E-04 | 2.38E-04 | 3.28E-06 | 1.47E-05 | 4.68E-05 | 9.31E-05 | 1.69E-04 |
| isot                | 19 K 39  | 2.84E-06 | 1.86E-05 | 5.92E-05 | 1.22E-04 | 2.26E-04 | 2.72E-06 | 1.33E-05 | 4.35E-05 | 8.76E-05 | 1.60E-04 |
| isot                | 19 K 40  | 8.30E-11 | 3.17E-09 | 2.45E-08 | 1.53E-07 | 5.16E-07 | 5.35E-11 | 1.91E-09 | 1.56E-08 | 9.18E-08 | 2.94E-07 |
| isot                | 19 K 41  | 6.71E-07 | 1.72E-06 | 4.15E-06 | 7.30E-06 | 1.17E-05 | 5.64E-07 | 1.35E-06 | 3.20E-06 | 5.43E-06 | 8.31E-06 |
| elem                | 20 Ca    | 4.90E-02 | 4.58E-02 | 4.18E-02 | 3.57E-02 | 2.49E-02 | 4.88E-02 | 4.58E-02 | 4.26E-02 | 3.71E-02 | 2.66E-02 |
| isot                | 20 Ca 40 | 4.90E-02 | 4.58E-02 | 4.17E-02 | 3.56E-02 | 2.47E-02 | 4.88E-02 | 4.58E-02 | 4.26E-02 | 3.71E-02 | 2.65E-02 |
| isot                | 20 Ca 42 | 1.75E-08 | 2.08E-06 | 1.49E-05 | 5.12E-05 | 1.69E-04 | 1.14E-08 | 1.38E-06 | 1.05E-05 | 3.54E-05 | 1.12E-04 |
| isot                | 20 Ca 43 | 1.06E-09 | 4.73E-09 | 3.87E-08 | 1.92E-07 | 1.02E-06 | 9.39E-10 | 2.70E-09 | 2.32E-08 | 1.09E-07 | 5.49E-07 |
| isot                | 20 Ca 44 | 2.70E-05 | 2.47E-05 | 2.19E-05 | 1.81E-05 | 1.56E-05 | 3.15E-05 | 2.93E-05 | 2.65E-05 | 2.33E-05 | 1.89E-05 |
| isot                | 20 Ca 46 | 3.75E-09 | 4.60E-09 | 1.47E-08 | 6.81E-08 | 8.42E-07 | 3.50E-09 | 3.91E-09 | 9.14E-09 | 3.23E-08 | 3.73E-07 |
| isot                | 20 Ca 48 | 1.57E-08 | 1.65E-08 | 2.18E-08 | 4.21E-08 | 2.65E-07 | 1.55E-08 | 1.62E-08 | 2.10E-08 | 3.41E-08 | 1.59E-07 |
| elem                | 21 Sc    | 9.90E-08 | 1.52E-07 | 2.84E-07 | 5.54E-07 | 1.76E-06 | 8.71E-08 | 1.38E-07 | 2.39E-07 | 4.03E-07 | 1.02E-06 |
| isot                | 21 Sc 45 | 9.90E-08 | 1.52E-07 | 2.84E-07 | 5.54E-07 | 1.76E-06 | 8.71E-08 | 1.38E-07 | 2.39E-07 | 4.03E-07 | 1.02E-06 |

Table A1 *continued*.

| $\rho_{\text{DDT}}$ |          | 1.2E+07  | 1.2E+07  | 1.2E+07  | 1.2E+07  | 1.2E+07  | 1.6E+07  | 1.6E+07  | 1.6E+07  | 1.6E+07  | 1.6E+07  |
|---------------------|----------|----------|----------|----------|----------|----------|----------|----------|----------|----------|----------|
| Z                   |          | 2.25E-4  | 2.25E-3  | 9.00E-3  | 2.25E-2  | 6.75E-2  | 2.25E-4  | 2.25E-3  | 9.00E-3  | 2.25E-2  | 6.75E-2  |
| elem                | 22 Ti    | 7.19E-04 | 7.11E-04 | 6.96E-04 | 6.75E-04 | 7.76E-04 | 8.96E-04 | 8.90E-04 | 8.62E-04 | 8.52E-04 | 8.91E-04 |
| isot                | 22 Ti 46 | 9.24E-08 | 1.85E-06 | 1.13E-05 | 3.21E-05 | 8.62E-05 | 8.85E-08 | 1.38E-06 | 8.23E-06 | 2.32E-05 | 6.07E-05 |
| isot                | 22 Ti 47 | 1.88E-08 | 1.95E-08 | 2.00E-07 | 9.99E-07 | 4.77E-06 | 2.20E-08 | 1.43E-08 | 1.30E-07 | 6.39E-07 | 2.84E-06 |
| isot                | 22 Ti 48 | 4.17E-04 | 4.00E-04 | 3.53E-04 | 2.74E-04 | 1.93E-04 | 5.97E-04 | 5.79E-04 | 5.20E-04 | 4.55E-04 | 3.30E-04 |
| isot                | 22 Ti 49 | 8.63E-06 | 1.19E-05 | 1.88E-05 | 2.42E-05 | 2.88E-05 | 7.62E-06 | 1.42E-05 | 2.22E-05 | 3.05E-05 | 3.85E-05 |
| isot                | 22 Ti 50 | 2.93E-04 | 2.98E-04 | 3.12E-04 | 3.44E-04 | 4.63E-04 | 2.92E-04 | 2.96E-04 | 3.11E-04 | 3.42E-04 | 4.59E-04 |
| elem                | 23 V     | 6.31E-05 | 7.25E-05 | 1.01E-04 | 1.35E-04 | 2.20E-04 | 6.45E-05 | 7.63E-05 | 1.11E-04 | 1.54E-04 | 2.47E-04 |
| isot                | 23 V 50  | 1.79E-08 | 1.85E-08 | 3.11E-08 | 1.50E-07 | 6.12E-07 | 1.71E-08 | 1.75E-08 | 2.46E-08 | 8.25E-08 | 3.39E-07 |
| isot                | 23 V 51  | 6.31E-05 | 7.25E-05 | 1.01E-04 | 1.35E-04 | 2.20E-04 | 6.45E-05 | 7.62E-05 | 1.11E-04 | 1.54E-04 | 2.47E-04 |
| elem                | 24 Cr    | 1.33E-02 | 1.32E-02 | 1.29E-02 | 1.22E-02 | 1.50E-02 | 1.95E-02 | 1.95E-02 | 1.85E-02 | 1.84E-02 | 1.97E-02 |
| isot                | 24 Cr 50 | 4.99E-05 | 8.41E-05 | 2.12E-04 | 5.29E-04 | 1.70E-03 | 5.78E-05 | 8.79E-05 | 2.06E-04 | 4.97E-04 | 1.58E-03 |
| isot                | 24 Cr 52 | 1.07E-02 | 1.04E-02 | 9.68E-03 | 8.37E-03 | 8.82E-03 | 1.68E-02 | 1.66E-02 | 1.51E-02 | 1.41E-02 | 1.30E-02 |
| isot                | 24 Cr 53 | 6.19E-04 | 7.28E-04 | 9.56E-04 | 1.14E-03 | 1.71E-03 | 7.01E-04 | 9.00E-04 | 1.21E-03 | 1.59E-03 | 2.35E-03 |
| isot                | 24 Cr 54 | 1.94E-03 | 1.96E-03 | 2.04E-03 | 2.21E-03 | 2.76E-03 | 1.94E-03 | 1.97E-03 | 2.04E-03 | 2.21E-03 | 2.76E-03 |
| elem                | 25 Mn    | 4.16E-03 | 5.32E-03 | 6.98E-03 | 8.57E-03 | 1.26E-02 | 4.45E-03 | 6.24E-03 | 8.76E-03 | 1.19E-02 | 1.83E-02 |
| isot                | 25 Mn 55 | 4.16E-03 | 5.32E-03 | 6.98E-03 | 8.57E-03 | 1.26E-02 | 4.45E-03 | 6.24E-03 | 8.76E-03 | 1.19E-02 | 1.83E-02 |
| elem                | 26 Fe    | 3.42E-01 | 3.43E-01 | 3.43E-01 | 3.35E-01 | 3.90E-01 | 5.65E-01 | 5.66E-01 | 5.38E-01 | 5.54E-01 | 5.95E-01 |
| isot                | 26 Fe 54 | 3.69E-02 | 4.05E-02 | 5.37E-02 | 8.02E-02 | 1.54E-01 | 3.67E-02 | 4.05E-02 | 5.49E-02 | 8.47E-02 | 1.74E-01 |
| isot                | 26 Fe 56 | 2.97E-01 | 2.94E-01 | 2.80E-01 | 2.44E-01 | 2.22E-01 | 5.19E-01 | 5.16E-01 | 4.72E-01 | 4.56E-01 | 4.04E-01 |
| isot                | 26 Fe 57 | 3.74E-03 | 4.13E-03 | 4.96E-03 | 5.71E-03 | 7.22E-03 | 4.37E-03 | 4.90E-03 | 6.09E-03 | 7.75E-03 | 1.07E-02 |
| isot                | 26 Fe 58 | 4.77E-03 | 4.81E-03 | 4.97E-03 | 5.29E-03 | 6.35E-03 | 4.78E-03 | 4.83E-03 | 4.98E-03 | 5.30E-03 | 6.35E-03 |
| elem                | 27 Co    | 3.41E-04 | 3.31E-04 | 3.38E-04 | 3.43E-04 | 4.18E-04 | 3.57E-04 | 3.45E-04 | 3.54E-04 | 3.66E-04 | 4.27E-04 |
| isot                | 27 Co 59 | 3.41E-04 | 3.31E-04 | 3.38E-04 | 3.43E-04 | 4.18E-04 | 3.57E-04 | 3.45E-04 | 3.54E-04 | 3.66E-04 | 4.27E-04 |
| elem                | 28 Ni    | 2.32E-02 | 2.38E-02 | 2.59E-02 | 2.99E-02 | 4.15E-02 | 2.31E-02 | 2.37E-02 | 2.60E-02 | 3.07E-02 | 4.53E-02 |
| isot                | 28 Ni 58 | 1.82E-02 | 1.86E-02 | 2.06E-02 | 2.43E-02 | 3.42E-02 | 1.81E-02 | 1.86E-02 | 2.08E-02 | 2.53E-02 | 3.86E-02 |
| isot                | 28 Ni 60 | 3.61E-03 | 3.64E-03 | 3.70E-03 | 3.79E-03 | 4.58E-03 | 3.60E-03 | 3.62E-03 | 3.66E-03 | 3.74E-03 | 4.34E-03 |
| isot                | 28 Ni 61 | 2.41E-05 | 2.60E-05 | 3.32E-05 | 4.80E-05 | 1.51E-04 | 2.40E-05 | 2.52E-05 | 2.92E-05 | 3.58E-05 | 8.98E-05 |
| isot                | 28 Ni 62 | 1.38E-03 | 1.40E-03 | 1.49E-03 | 1.72E-03 | 2.45E-03 | 1.37E-03 | 1.39E-03 | 1.47E-03 | 1.63E-03 | 2.15E-03 |
| isot                | 28 Ni 64 | 3.50E-05 | 3.59E-05 | 4.03E-05 | 5.57E-05 | 1.40E-04 | 3.49E-05 | 3.59E-05 | 3.94E-05 | 5.14E-05 | 1.12E-04 |
| elem                | 29 Cu    | 1.05E-06 | 2.04E-06 | 1.18E-05 | 3.53E-05 | 9.72E-05 | 1.12E-06 | 1.42E-06 | 6.87E-06 | 1.86E-05 | 4.92E-05 |
| isot                | 29 Cu 63 | 8.44E-07 | 1.30E-06 | 6.84E-06 | 1.55E-05 | 3.79E-05 | 9.23E-07 | 8.90E-07 | 3.90E-06 | 7.91E-06 | 1.82E-05 |
| isot                | 29 Cu 65 | 2.03E-07 | 7.43E-07 | 4.97E-06 | 1.99E-05 | 5.93E-05 | 1.95E-07 | 5.33E-07 | 2.98E-06 | 1.07E-05 | 3.09E-05 |
| elem                | 30 Zn    | 2.29E-06 | 1.16E-05 | 6.16E-05 | 1.43E-04 | 1.45E-04 | 2.33E-06 | 7.70E-06 | 3.99E-05 | 8.72E-05 | 8.44E-05 |
| isot                | 30 Zn 64 | 2.10E-06 | 8.76E-06 | 2.22E-05 | 1.75E-05 | 7.26E-06 | 2.15E-06 | 5.41E-06 | 1.26E-05 | 9.67E-06 | 4.31E-06 |
| isot                | 30 Zn 66 | 1.47E-07 | 2.16E-06 | 3.70E-05 | 1.07E-04 | 9.85E-05 | 1.44E-07 | 1.81E-06 | 2.55E-05 | 6.64E-05 | 5.92E-05 |
| isot                | 30 Zn 67 | 1.22E-08 | 7.94E-08 | 5.28E-07 | 2.14E-06 | 9.36E-06 | 1.18E-08 | 5.40E-08 | 3.53E-07 | 1.24E-06 | 4.82E-06 |
| isot                | 30 Zn 68 | 3.64E-08 | 5.62E-07 | 1.91E-06 | 1.60E-05 | 2.92E-05 | 3.07E-08 | 4.20E-07 | 1.34E-06 | 9.78E-06 | 1.57E-05 |
| isot                | 30 Zn 70 | 2.93E-10 | 1.46E-09 | 1.89E-08 | 1.64E-07 | 7.38E-07 | 2.71E-10 | 8.44E-10 | 1.12E-08 | 9.88E-08 | 3.89E-07 |
| elem                | 31 Ga    | 1.60E-09 | 8.67E-08 | 1.12E-06 | 6.21E-06 | 4.37E-06 | 1.10E-09 | 6.55E-08 | 8.24E-07 | 3.86E-06 | 2.29E-06 |
| isot                | 31 Ga 69 | 1.40E-09 | 8.06E-08 | 1.01E-06 | 4.99E-06 | 2.83E-06 | 9.59E-10 | 6.11E-08 | 7.32E-07 | 3.06E-06 | 1.50E-06 |
| isot                | 31 Ga 71 | 1.98E-10 | 6.07E-09 | 1.10E-07 | 1.23E-06 | 1.53E-06 | 1.39E-10 | 4.36E-09 | 9.19E-08 | 8.00E-07 | 7.89E-07 |
| elem                | 32 Ge    | 6.88E-09 | 7.44E-07 | 1.38E-05 | 3.50E-05 | 8.41E-06 | 5.22E-09 | 7.41E-07 | 1.12E-05 | 2.42E-05 | 5.04E-06 |
| isot                | 32 Ge 70 | 4.18E-09 | 6.55E-07 | 1.08E-05 | 2.02E-05 | 3.57E-06 | 3.56E-09 | 6.42E-07 | 8.47E-06 | 1.36E-05 | 2.21E-06 |
| isot                | 32 Ge 72 | 2.07E-09 | 7.83E-08 | 2.90E-06 | 1.40E-05 | 4.19E-06 | 1.27E-09 | 9.04E-08 | 2.64E-06 | 1.00E-05 | 2.51E-06 |
| isot                | 32 Ge 73 | 4.99E-10 | 9.64E-09 | 5.49E-08 | 1.15E-07 | 1.55E-07 | 3.14E-10 | 7.63E-09 | 5.00E-08 | 7.92E-08 | 7.78E-08 |
| isot                | 32 Ge 74 | 9.19E-11 | 1.11E-09 | 3.18E-08 | 5.62E-07 | 4.60E-07 | 5.76E-11 | 6.39E-10 | 2.55E-08 | 3.74E-07 | 2.25E-07 |
| isot                | 32 Ge 76 | 3.74E-11 | 2.22E-10 | 1.99E-09 | 1.28E-08 | 4.04E-08 | 2.19E-11 | 1.12E-10 | 1.21E-09 | 7.57E-09 | 2.04E-08 |
| elem                | 33 As    | 1.57E-10 | 4.78E-09 | 9.25E-08 | 6.46E-07 | 1.71E-07 | 9.85E-11 | 4.83E-09 | 8.08E-08 | 4.40E-07 | 9.15E-08 |
| isot                | 33 As 75 | 1.57E-10 | 4.78E-09 | 9.25E-08 | 6.46E-07 | 1.71E-07 | 9.85E-11 | 4.83E-09 | 8.08E-08 | 4.40E-07 | 9.15E-08 |
| elem                | 34 Se    | 4.12E-09 | 2.46E-07 | 4.96E-06 | 8.75E-06 | 6.77E-07 | 3.48E-09 | 3.23E-07 | 5.12E-06 | 7.17E-06 | 4.29E-07 |
| isot                | 34 Se 74 | 3.07E-09 | 1.90E-07 | 2.42E-06 | 3.42E-06 | 2.04E-07 | 2.51E-09 | 2.37E-07 | 2.40E-06 | 2.84E-06 | 1.40E-07 |
| isot                | 34 Se 76 | 5.12E-10 | 5.17E-08 | 2.45E-06 | 4.84E-06 | 3.08E-07 | 6.05E-10 | 8.34E-08 | 2.63E-06 | 3.98E-06 | 2.06E-07 |
| isot                | 34 Se 77 | 3.34E-10 | 2.14E-09 | 1.00E-08 | 5.93E-08 | 4.50E-08 | 2.66E-10 | 1.57E-09 | 9.31E-09 | 3.95E-08 | 2.22E-08 |
| isot                | 34 Se 78 | 6.55E-11 | 1.19E-09 | 8.01E-08 | 4.04E-07 | 7.35E-08 | 3.59E-11 | 8.67E-10 | 8.30E-08 | 2.98E-07 | 4.13E-08 |
| isot                | 34 Se 80 | 1.32E-10 | 6.07E-10 | 4.89E-09 | 2.08E-08 | 4.60E-08 | 6.46E-11 | 2.99E-10 | 2.84E-09 | 1.08E-08 | 2.04E-08 |
| elem                | 35 Br    | 7.37E-11 | 3.09E-09 | 3.31E-08 | 5.18E-08 | 1.56E-08 | 5.03E-11 | 2.88E-09 | 3.03E-08 | 3.72E-08 | 7.58E-09 |
| isot                | 35 Br 79 | 7.37E-11 | 3.09E-09 | 3.31E-08 | 5.18E-08 | 1.56E-08 | 5.03E-11 | 2.88E-09 | 3.03E-08 | 3.72E-08 | 7.58E-09 |
| elem                | 36 Kr    | 1.36E-09 | 5.32E-08 | 8.97E-07 | 7.24E-07 | 3.06E-08 | 1.61E-09 | 7.57E-08 | 1.11E-06 | 6.81E-07 | 1.93E-08 |
| isot                | 36 Kr 78 | 1.18E-09 | 2.95E-08 | 1.89E-07 | 1.24E-07 | 5.42E-09 | 1.44E-09 | 3.77E-08 | 2.24E-07 | 1.16E-07 | 3.40E-09 |
| isot                | 36 Kr 80 | 1.76E-10 | 2.37E-08 | 7.08E-07 | 6.00E-07 | 2.52E-08 | 1.75E-10 | 3.80E-08 | 8.89E-07 | 5.65E-07 | 1.59E-08 |

Table A1 *continued.*

|                     |          |          |          |          |          |          |          |          |          |          |          |
|---------------------|----------|----------|----------|----------|----------|----------|----------|----------|----------|----------|----------|
| $\rho_{\text{DDT}}$ |          | 2.4E+07  | 2.4E+07  | 2.4E+07  | 2.4E+07  | 2.4E+07  | 2.8E+07  | 2.8E+07  | 2.8E+07  | 2.8E+07  | 2.8E+07  |
| Z                   |          | 2.25E-4  | 2.25E-3  | 9.00E-3  | 2.25E-2  | 6.75E-2  | 2.25E-4  | 2.25E-3  | 9.00E-3  | 2.25E-2  | 6.75E-2  |
| elem                | 2 He     | 1.87E-04 | 1.82E-04 | 1.01E-04 | 8.80E-04 | 5.56E-06 | 3.07E-03 | 3.34E-03 | 3.65E-03 | 2.69E-03 | 2.57E-03 |
| isot                | 2 He 3   | 1.80E-12 | 1.78E-12 | 1.76E-12 | 1.62E-12 | 1.33E-12 | 1.80E-12 | 1.78E-12 | 1.76E-12 | 1.62E-12 | 1.33E-12 |
| isot                | 2 He 4   | 1.87E-04 | 1.82E-04 | 1.01E-04 | 8.80E-04 | 5.56E-06 | 3.07E-03 | 3.34E-03 | 3.65E-03 | 2.69E-03 | 2.57E-03 |
| elem                | 6 C      | 1.26E-03 | 1.25E-03 | 1.26E-03 | 1.22E-03 | 1.25E-03 | 1.02E-03 | 1.03E-03 | 9.86E-04 | 1.01E-03 | 9.71E-04 |
| isot                | 6 C 12   | 1.26E-03 | 1.25E-03 | 1.26E-03 | 1.22E-03 | 1.25E-03 | 1.02E-03 | 1.03E-03 | 9.86E-04 | 1.01E-03 | 9.71E-04 |
| isot                | 6 C 13   | 8.07E-11 | 1.16E-09 | 4.40E-09 | 1.04E-08 | 2.77E-08 | 6.21E-11 | 8.31E-10 | 3.23E-09 | 8.00E-09 | 2.00E-08 |
| elem                | 7 N      | 7.52E-06 | 6.17E-06 | 4.37E-06 | 2.72E-06 | 1.27E-06 | 6.37E-06 | 5.34E-06 | 3.64E-06 | 2.32E-06 | 9.69E-07 |
| isot                | 7 N 14   | 7.48E-06 | 6.17E-06 | 4.37E-06 | 2.72E-06 | 1.27E-06 | 6.34E-06 | 5.34E-06 | 3.64E-06 | 2.32E-06 | 9.68E-07 |
| isot                | 7 N 15   | 3.81E-08 | 1.11E-09 | 6.75E-10 | 8.56E-10 | 1.28E-09 | 2.98E-08 | 8.95E-10 | 4.99E-10 | 6.77E-10 | 9.32E-10 |
| elem                | 8 O      | 6.58E-02 | 6.71E-02 | 6.87E-02 | 6.83E-02 | 7.15E-02 | 5.42E-02 | 5.57E-02 | 5.51E-02 | 5.87E-02 | 5.83E-02 |
| isot                | 8 O 16   | 6.58E-02 | 6.71E-02 | 6.87E-02 | 6.83E-02 | 7.15E-02 | 5.42E-02 | 5.57E-02 | 5.51E-02 | 5.87E-02 | 5.83E-02 |
| isot                | 8 O 17   | 2.90E-09 | 3.02E-08 | 6.39E-08 | 8.27E-08 | 8.80E-08 | 2.25E-09 | 2.25E-08 | 4.54E-08 | 6.38E-08 | 6.10E-08 |
| isot                | 8 O 18   | 5.89E-10 | 4.18E-10 | 4.45E-10 | 4.86E-10 | 5.09E-10 | 6.12E-10 | 3.41E-10 | 3.27E-10 | 3.73E-10 | 3.60E-10 |
| elem                | 9 F      | 9.17E-12 | 2.23E-12 | 3.76E-12 | 8.87E-12 | 3.03E-11 | 6.44E-12 | 1.66E-12 | 2.89E-12 | 7.31E-12 | 2.30E-11 |
| isot                | 9 F 19   | 9.17E-12 | 2.23E-12 | 3.76E-12 | 8.87E-12 | 3.03E-11 | 6.44E-12 | 1.66E-12 | 2.89E-12 | 7.31E-12 | 2.30E-11 |
| elem                | 10 Ne    | 7.04E-04 | 7.01E-04 | 7.07E-04 | 6.89E-04 | 7.66E-04 | 5.31E-04 | 5.40E-04 | 5.19E-04 | 5.41E-04 | 5.79E-04 |
| isot                | 10 Ne 20 | 7.04E-04 | 7.00E-04 | 7.03E-04 | 6.76E-04 | 7.03E-04 | 5.31E-04 | 5.39E-04 | 5.16E-04 | 5.31E-04 | 5.35E-04 |
| isot                | 10 Ne 21 | 1.89E-09 | 1.25E-08 | 3.97E-08 | 9.24E-08 | 3.64E-07 | 3.75E-09 | 1.03E-08 | 3.01E-08 | 7.74E-08 | 2.82E-07 |
| isot                | 10 Ne 22 | 4.92E-08 | 6.46E-07 | 3.72E-06 | 1.27E-05 | 6.25E-05 | 1.56E-07 | 4.90E-07 | 2.61E-06 | 9.52E-06 | 4.40E-05 |
| elem                | 11 Na    | 4.70E-06 | 5.06E-06 | 6.73E-06 | 1.04E-05 | 2.63E-05 | 3.57E-06 | 3.92E-06 | 4.99E-06 | 8.29E-06 | 1.98E-05 |
| isot                | 11 Na 23 | 4.70E-06 | 5.06E-06 | 6.73E-06 | 1.04E-05 | 2.63E-05 | 3.57E-06 | 3.92E-06 | 4.99E-06 | 8.29E-06 | 1.98E-05 |
| elem                | 12 Mg    | 1.23E-02 | 1.09E-02 | 8.11E-03 | 5.41E-03 | 3.19E-03 | 9.49E-03 | 8.48E-03 | 5.94E-03 | 4.28E-03 | 2.39E-03 |
| isot                | 12 Mg 24 | 1.23E-02 | 1.09E-02 | 8.09E-03 | 5.37E-03 | 3.05E-03 | 9.49E-03 | 8.48E-03 | 5.93E-03 | 4.25E-03 | 2.28E-03 |
| isot                | 12 Mg 25 | 3.39E-07 | 3.12E-06 | 7.43E-06 | 1.65E-05 | 5.13E-05 | 2.91E-07 | 2.41E-06 | 5.47E-06 | 1.32E-05 | 3.82E-05 |
| isot                | 12 Mg 26 | 2.73E-07 | 2.12E-06 | 9.52E-06 | 2.38E-05 | 9.15E-05 | 9.43E-07 | 1.80E-06 | 7.32E-06 | 1.98E-05 | 7.21E-05 |
| elem                | 13 Al    | 2.69E-05 | 1.01E-04 | 1.92E-04 | 2.18E-04 | 2.22E-04 | 2.04E-05 | 7.82E-05 | 1.39E-04 | 1.70E-04 | 1.65E-04 |
| isot                | 13 Al 27 | 2.69E-05 | 1.01E-04 | 1.92E-04 | 2.18E-04 | 2.22E-04 | 2.04E-05 | 7.82E-05 | 1.39E-04 | 1.70E-04 | 1.65E-04 |
| elem                | 14 Si    | 2.38E-01 | 2.42E-01 | 2.48E-01 | 2.45E-01 | 2.41E-01 | 2.08E-01 | 2.14E-01 | 2.14E-01 | 2.19E-01 | 2.12E-01 |
| isot                | 14 Si 28 | 2.37E-01 | 2.42E-01 | 2.47E-01 | 2.44E-01 | 2.37E-01 | 2.08E-01 | 2.14E-01 | 2.14E-01 | 2.18E-01 | 2.09E-01 |
| isot                | 14 Si 29 | 6.39E-05 | 1.80E-04 | 2.71E-04 | 3.84E-04 | 9.09E-04 | 5.29E-05 | 1.46E-04 | 2.10E-04 | 3.20E-04 | 7.09E-04 |
| isot                | 14 Si 30 | 7.56E-06 | 6.45E-05 | 3.58E-04 | 8.54E-04 | 3.04E-03 | 8.48E-06 | 5.27E-05 | 2.69E-04 | 6.91E-04 | 2.34E-03 |
| elem                | 15 P     | 2.62E-05 | 5.22E-05 | 1.38E-04 | 2.46E-04 | 5.98E-04 | 2.33E-05 | 4.43E-05 | 1.09E-04 | 2.09E-04 | 4.85E-04 |
| isot                | 15 P 31  | 2.62E-05 | 5.22E-05 | 1.38E-04 | 2.46E-04 | 5.98E-04 | 2.33E-05 | 4.43E-05 | 1.09E-04 | 2.09E-04 | 4.85E-04 |
| elem                | 16 S     | 1.45E-01 | 1.43E-01 | 1.42E-01 | 1.35E-01 | 1.15E-01 | 1.28E-01 | 1.28E-01 | 1.24E-01 | 1.21E-01 | 1.01E-01 |
| isot                | 16 S 32  | 1.45E-01 | 1.43E-01 | 1.41E-01 | 1.33E-01 | 1.06E-01 | 1.28E-01 | 1.28E-01 | 1.23E-01 | 1.19E-01 | 9.39E-02 |
| isot                | 16 S 33  | 2.98E-05 | 6.28E-05 | 1.27E-04 | 1.92E-04 | 3.59E-04 | 2.47E-05 | 5.39E-05 | 1.05E-04 | 1.69E-04 | 3.08E-04 |
| isot                | 16 S 34  | 1.37E-06 | 1.51E-04 | 8.48E-04 | 2.28E-03 | 8.04E-03 | 2.87E-06 | 1.32E-04 | 7.04E-04 | 2.02E-03 | 6.78E-03 |
| isot                | 16 S 36  | 1.24E-10 | 2.49E-09 | 2.55E-08 | 1.46E-07 | 4.02E-06 | 1.15E-10 | 2.05E-09 | 2.02E-08 | 1.23E-07 | 3.01E-06 |
| elem                | 17 Cl    | 8.58E-06 | 1.99E-05 | 5.63E-05 | 1.14E-04 | 2.42E-04 | 8.49E-06 | 1.85E-05 | 4.87E-05 | 1.02E-04 | 2.11E-04 |
| isot                | 17 Cl 35 | 5.56E-06 | 1.37E-05 | 4.36E-05 | 9.28E-05 | 2.01E-04 | 5.82E-06 | 1.28E-05 | 3.75E-05 | 8.31E-05 | 1.75E-04 |
| isot                | 17 Cl 37 | 3.01E-06 | 6.20E-06 | 1.27E-05 | 2.09E-05 | 4.07E-05 | 2.67E-06 | 5.70E-06 | 1.12E-05 | 1.92E-05 | 3.62E-05 |
| elem                | 18 Ar    | 3.43E-02 | 3.29E-02 | 3.13E-02 | 2.86E-02 | 2.38E-02 | 3.03E-02 | 2.94E-02 | 2.73E-02 | 2.57E-02 | 2.10E-02 |
| isot                | 18 Ar 36 | 3.43E-02 | 3.28E-02 | 3.09E-02 | 2.75E-02 | 1.99E-02 | 3.03E-02 | 2.94E-02 | 2.70E-02 | 2.46E-02 | 1.76E-02 |
| isot                | 18 Ar 38 | 6.62E-07 | 6.11E-05 | 3.79E-04 | 1.13E-03 | 3.92E-03 | 7.86E-07 | 5.62E-05 | 3.28E-04 | 1.04E-03 | 3.43E-03 |
| isot                | 18 Ar 40 | 1.59E-11 | 4.70E-10 | 5.39E-09 | 2.38E-08 | 2.89E-07 | 1.46E-11 | 3.97E-10 | 4.34E-09 | 2.05E-08 | 2.22E-07 |
| elem                | 19 K     | 2.92E-06 | 1.21E-05 | 3.68E-05 | 7.10E-05 | 1.33E-04 | 2.91E-06 | 1.14E-05 | 3.33E-05 | 6.59E-05 | 1.21E-04 |
| isot                | 19 K 39  | 2.42E-06 | 1.10E-05 | 3.42E-05 | 6.67E-05 | 1.26E-04 | 2.44E-06 | 1.04E-05 | 3.10E-05 | 6.20E-05 | 1.15E-04 |
| isot                | 19 K 40  | 4.14E-11 | 1.36E-09 | 9.47E-09 | 4.99E-08 | 1.66E-07 | 3.68E-11 | 1.16E-09 | 7.77E-09 | 4.21E-08 | 1.33E-07 |
| isot                | 19 K 41  | 4.97E-07 | 1.11E-06 | 2.52E-06 | 4.16E-06 | 6.51E-06 | 4.75E-07 | 1.05E-06 | 2.27E-06 | 3.88E-06 | 5.93E-06 |
| elem                | 20 Ca    | 3.79E-02 | 3.57E-02 | 3.28E-02 | 2.83E-02 | 2.05E-02 | 3.31E-02 | 3.17E-02 | 2.84E-02 | 2.53E-02 | 1.81E-02 |
| isot                | 20 Ca 40 | 3.78E-02 | 3.57E-02 | 3.28E-02 | 2.82E-02 | 2.04E-02 | 3.31E-02 | 3.17E-02 | 2.83E-02 | 2.53E-02 | 1.80E-02 |
| isot                | 20 Ca 42 | 1.08E-08 | 1.16E-06 | 8.36E-06 | 2.69E-05 | 8.77E-05 | 1.17E-08 | 1.10E-06 | 7.38E-06 | 2.50E-05 | 7.82E-05 |
| isot                | 20 Ca 43 | 1.41E-09 | 1.74E-09 | 1.44E-08 | 6.85E-08 | 3.34E-07 | 9.57E-09 | 1.49E-08 | 1.31E-07 | 1.01E-07 | 3.08E-07 |
| isot                | 20 Ca 44 | 3.03E-05 | 2.69E-05 | 2.39E-05 | 2.09E-05 | 1.59E-05 | 2.90E-05 | 2.92E-05 | 3.11E-05 | 2.39E-05 | 1.95E-05 |
| isot                | 20 Ca 46 | 3.48E-09 | 3.76E-09 | 6.23E-09 | 1.60E-08 | 1.56E-07 | 3.46E-09 | 3.70E-09 | 5.72E-09 | 1.42E-08 | 1.18E-07 |
| isot                | 20 Ca 48 | 1.54E-08 | 1.65E-08 | 2.02E-08 | 3.04E-08 | 1.17E-07 | 1.58E-08 | 1.67E-08 | 2.04E-08 | 3.03E-08 | 1.08E-07 |
| elem                | 21 Sc    | 8.01E-08 | 1.15E-07 | 1.89E-07 | 2.88E-07 | 6.28E-07 | 7.73E-08 | 1.08E-07 | 1.70E-07 | 2.64E-07 | 5.35E-07 |
| isot                | 21 Sc 45 | 8.01E-08 | 1.15E-07 | 1.89E-07 | 2.88E-07 | 6.28E-07 | 7.73E-08 | 1.08E-07 | 1.70E-07 | 2.64E-07 | 5.35E-07 |

Table A1 *continued.*

| $\rho_{\text{DDT}}$ |          | 2.4E+07  | 2.4E+07  | 2.4E+07  | 2.4E+07  | 2.4E+07  | 2.8E+07  | 2.8E+07  | 2.8E+07  | 2.8E+07  | 2.8E+07  |
|---------------------|----------|----------|----------|----------|----------|----------|----------|----------|----------|----------|----------|
| Z                   |          | 2.25E-4  | 2.25E-3  | 9.00E-3  | 2.25E-2  | 6.75E-2  | 2.25E-4  | 2.25E-3  | 9.00E-3  | 2.25E-2  | 6.75E-2  |
| elem                | 22 Ti    | 8.55E-04 | 8.47E-04 | 8.40E-04 | 8.03E-04 | 8.28E-04 | 7.81E-04 | 7.85E-04 | 7.69E-04 | 7.66E-04 | 7.93E-04 |
| isot                | 22 Ti 46 | 1.11E-07 | 1.16E-06 | 6.65E-06 | 1.79E-05 | 4.76E-05 | 1.22E-06 | 1.16E-06 | 5.93E-06 | 1.66E-05 | 4.32E-05 |
| isot                | 22 Ti 47 | 4.05E-08 | 1.39E-08 | 1.06E-07 | 4.65E-07 | 1.89E-06 | 1.51E-06 | 1.20E-07 | 3.64E-07 | 5.85E-07 | 1.86E-06 |
| isot                | 22 Ti 48 | 5.57E-04 | 5.37E-04 | 5.02E-04 | 4.16E-04 | 2.89E-04 | 4.82E-04 | 4.77E-04 | 4.35E-04 | 3.83E-04 | 2.63E-04 |
| isot                | 22 Ti 49 | 6.11E-06 | 1.33E-05 | 2.09E-05 | 2.74E-05 | 3.38E-05 | 5.39E-06 | 1.20E-05 | 1.80E-05 | 2.50E-05 | 3.03E-05 |
| isot                | 22 Ti 50 | 2.91E-04 | 2.96E-04 | 3.10E-04 | 3.42E-04 | 4.56E-04 | 2.91E-04 | 2.95E-04 | 3.10E-04 | 3.41E-04 | 4.55E-04 |
| elem                | 23 V     | 6.45E-05 | 7.62E-05 | 1.11E-04 | 1.46E-04 | 2.25E-04 | 6.37E-05 | 7.43E-05 | 1.03E-04 | 1.39E-04 | 2.09E-04 |
| isot                | 23 V 50  | 1.66E-08 | 1.69E-08 | 2.01E-08 | 4.21E-08 | 1.76E-07 | 1.65E-08 | 1.69E-08 | 1.94E-08 | 3.61E-08 | 1.36E-07 |
| isot                | 23 V 51  | 6.45E-05 | 7.62E-05 | 1.11E-04 | 1.46E-04 | 2.25E-04 | 6.37E-05 | 7.43E-05 | 1.03E-04 | 1.39E-04 | 2.09E-04 |
| elem                | 24 Cr    | 2.11E-02 | 2.09E-02 | 2.10E-02 | 1.88E-02 | 1.89E-02 | 1.83E-02 | 1.83E-02 | 1.77E-02 | 1.76E-02 | 1.74E-02 |
| isot                | 24 Cr 50 | 6.25E-05 | 8.55E-05 | 1.83E-04 | 4.06E-04 | 1.26E-03 | 6.87E-05 | 8.28E-05 | 1.66E-04 | 3.74E-04 | 1.13E-03 |
| isot                | 24 Cr 52 | 1.84E-02 | 1.79E-02 | 1.74E-02 | 1.46E-02 | 1.26E-02 | 1.57E-02 | 1.54E-02 | 1.43E-02 | 1.35E-02 | 1.15E-02 |
| isot                | 24 Cr 53 | 7.01E-04 | 9.64E-04 | 1.36E-03 | 1.64E-03 | 2.29E-03 | 6.42E-04 | 8.79E-04 | 1.16E-03 | 1.52E-03 | 2.07E-03 |
| isot                | 24 Cr 54 | 1.94E-03 | 1.97E-03 | 2.04E-03 | 2.20E-03 | 2.76E-03 | 1.94E-03 | 1.96E-03 | 2.04E-03 | 2.21E-03 | 2.76E-03 |
| elem                | 25 Mn    | 4.43E-03 | 6.53E-03 | 1.02E-02 | 1.30E-02 | 2.05E-02 | 4.38E-03 | 6.06E-03 | 8.73E-03 | 1.21E-02 | 1.81E-02 |
| isot                | 25 Mn 55 | 4.43E-03 | 6.53E-03 | 1.02E-02 | 1.30E-02 | 2.05E-02 | 4.38E-03 | 6.06E-03 | 8.73E-03 | 1.21E-02 | 1.81E-02 |
| elem                | 26 Fe    | 7.92E-01 | 7.89E-01 | 7.82E-01 | 7.84E-01 | 7.70E-01 | 8.57E-01 | 8.49E-01 | 8.51E-01 | 8.34E-01 | 8.07E-01 |
| isot                | 26 Fe 54 | 3.67E-02 | 4.03E-02 | 5.51E-02 | 8.07E-02 | 1.65E-01 | 3.67E-02 | 3.97E-02 | 5.13E-02 | 7.61E-02 | 1.49E-01 |
| isot                | 26 Fe 56 | 7.45E-01 | 7.38E-01 | 7.14E-01 | 6.85E-01 | 5.81E-01 | 8.08E-01 | 7.96E-01 | 7.83E-01 | 7.37E-01 | 6.30E-01 |
| isot                | 26 Fe 57 | 5.34E-03 | 6.28E-03 | 8.00E-03 | 1.26E-02 | 1.78E-02 | 6.67E-03 | 8.90E-03 | 1.18E-02 | 1.50E-02 | 2.21E-02 |
| isot                | 26 Fe 58 | 4.78E-03 | 4.83E-03 | 4.99E-03 | 5.31E-03 | 6.36E-03 | 4.79E-03 | 4.84E-03 | 5.00E-03 | 5.32E-03 | 6.36E-03 |
| elem                | 27 Co    | 4.18E-04 | 3.46E-04 | 3.50E-04 | 4.62E-04 | 4.23E-04 | 1.07E-03 | 3.67E-04 | 5.32E-04 | 6.22E-04 | 8.51E-04 |
| isot                | 27 Co 59 | 4.18E-04 | 3.46E-04 | 3.50E-04 | 4.62E-04 | 4.23E-04 | 1.07E-03 | 3.67E-04 | 5.32E-04 | 6.22E-04 | 8.51E-04 |
| elem                | 28 Ni    | 2.32E-02 | 2.39E-02 | 2.67E-02 | 3.95E-02 | 7.01E-02 | 2.78E-02 | 2.85E-02 | 3.53E-02 | 4.74E-02 | 9.62E-02 |
| isot                | 28 Ni 58 | 1.82E-02 | 1.88E-02 | 2.16E-02 | 3.28E-02 | 6.39E-02 | 1.89E-02 | 1.88E-02 | 2.49E-02 | 3.76E-02 | 8.35E-02 |
| isot                | 28 Ni 60 | 3.64E-03 | 3.66E-03 | 3.62E-03 | 4.62E-03 | 4.11E-03 | 7.39E-03 | 8.06E-03 | 8.20E-03 | 6.86E-03 | 6.72E-03 |
| isot                | 28 Ni 61 | 2.40E-05 | 2.53E-05 | 2.65E-05 | 6.46E-05 | 5.47E-05 | 4.83E-05 | 1.06E-04 | 1.56E-04 | 1.57E-04 | 2.45E-04 |
| isot                | 28 Ni 62 | 1.37E-03 | 1.39E-03 | 1.45E-03 | 1.94E-03 | 1.97E-03 | 1.37E-03 | 1.44E-03 | 2.02E-03 | 2.72E-03 | 5.64E-03 |
| isot                | 28 Ni 64 | 3.47E-05 | 3.57E-05 | 3.95E-05 | 4.84E-05 | 9.56E-05 | 3.48E-05 | 3.56E-05 | 3.91E-05 | 4.81E-05 | 9.08E-05 |
| elem                | 29 Cu    | 1.34E-06 | 1.02E-06 | 3.22E-06 | 8.25E-06 | 2.42E-05 | 5.27E-05 | 1.17E-05 | 3.44E-06 | 7.34E-06 | 2.11E-05 |
| isot                | 29 Cu 63 | 1.15E-06 | 6.49E-07 | 1.83E-06 | 3.67E-06 | 8.29E-06 | 5.25E-05 | 1.09E-05 | 1.86E-06 | 3.42E-06 | 8.35E-06 |
| isot                | 29 Cu 65 | 1.90E-07 | 3.75E-07 | 1.39E-06 | 4.59E-06 | 1.59E-05 | 2.73E-07 | 7.34E-07 | 1.57E-06 | 3.92E-06 | 1.27E-05 |
| elem                | 30 Zn    | 2.55E-06 | 4.64E-06 | 2.04E-05 | 5.17E-05 | 4.83E-05 | 7.84E-05 | 1.01E-04 | 4.93E-05 | 6.68E-05 | 1.10E-04 |
| isot                | 30 Zn 64 | 2.38E-06 | 3.03E-06 | 5.53E-06 | 6.74E-06 | 2.56E-06 | 7.64E-05 | 9.67E-05 | 2.62E-05 | 1.45E-05 | 1.12E-05 |
| isot                | 30 Zn 66 | 1.37E-07 | 1.30E-06 | 1.39E-05 | 3.92E-05 | 3.46E-05 | 3.01E-07 | 3.90E-06 | 2.24E-05 | 4.77E-05 | 8.96E-05 |
| isot                | 30 Zn 67 | 1.20E-08 | 3.39E-08 | 1.87E-07 | 5.65E-07 | 2.27E-06 | 4.66E-07 | 9.22E-08 | 1.52E-07 | 4.62E-07 | 1.70E-06 |
| isot                | 30 Zn 68 | 2.65E-08 | 2.83E-07 | 7.30E-07 | 5.05E-06 | 8.62E-06 | 1.25E-06 | 4.84E-07 | 5.69E-07 | 4.06E-06 | 6.88E-06 |
| isot                | 30 Zn 70 | 2.44E-10 | 5.27E-10 | 5.44E-09 | 4.71E-08 | 2.01E-07 | 2.54E-10 | 4.79E-10 | 4.28E-09 | 3.76E-08 | 1.49E-07 |
| elem                | 31 Ga    | 7.21E-10 | 4.51E-08 | 4.73E-07 | 2.17E-06 | 1.33E-06 | 1.43E-09 | 3.92E-08 | 3.64E-07 | 1.77E-06 | 1.08E-06 |
| isot                | 31 Ga 69 | 6.40E-10 | 4.20E-08 | 4.09E-07 | 1.71E-06 | 8.76E-07 | 7.75E-10 | 3.61E-08 | 3.10E-07 | 1.39E-06 | 7.18E-07 |
| isot                | 31 Ga 71 | 8.13E-11 | 3.06E-09 | 6.40E-08 | 4.61E-07 | 4.58E-07 | 6.53E-10 | 3.10E-09 | 5.37E-08 | 3.78E-07 | 3.61E-07 |
| elem                | 32 Ge    | 3.72E-09 | 6.45E-07 | 7.73E-06 | 1.57E-05 | 3.17E-06 | 3.92E-08 | 6.64E-07 | 6.57E-06 | 1.39E-05 | 3.46E-06 |
| isot                | 32 Ge 70 | 2.61E-09 | 5.46E-07 | 5.58E-06 | 8.55E-06 | 1.43E-06 | 2.17E-08 | 5.66E-07 | 4.70E-06 | 7.57E-06 | 1.99E-06 |
| isot                | 32 Ge 72 | 8.56E-10 | 9.23E-08 | 2.09E-06 | 6.80E-06 | 1.56E-06 | 1.72E-08 | 9.14E-08 | 1.80E-06 | 6.00E-06 | 1.33E-06 |
| isot                | 32 Ge 73 | 2.06E-10 | 6.42E-09 | 4.70E-08 | 5.86E-08 | 4.02E-08 | 1.74E-10 | 5.78E-09 | 4.29E-08 | 5.29E-08 | 3.04E-08 |
| isot                | 32 Ge 74 | 3.41E-11 | 3.93E-10 | 1.98E-08 | 2.59E-07 | 1.28E-07 | 3.09E-11 | 3.30E-10 | 1.71E-08 | 2.27E-07 | 1.06E-07 |
| isot                | 32 Ge 76 | 1.31E-11 | 5.71E-11 | 7.26E-10 | 4.65E-09 | 1.02E-08 | 1.07E-11 | 4.58E-11 | 6.21E-10 | 4.05E-09 | 7.48E-09 |
| elem                | 33 As    | 5.43E-11 | 5.19E-09 | 7.41E-08 | 3.30E-07 | 5.59E-08 | 4.27E-11 | 5.06E-09 | 6.73E-08 | 2.99E-07 | 4.80E-08 |
| isot                | 33 As 75 | 5.43E-11 | 5.19E-09 | 7.41E-08 | 3.30E-07 | 5.59E-08 | 4.27E-11 | 5.06E-09 | 6.73E-08 | 2.99E-07 | 4.80E-08 |
| elem                | 34 Se    | 2.83E-09 | 3.83E-07 | 4.86E-06 | 5.85E-06 | 2.88E-07 | 2.57E-09 | 3.92E-07 | 4.62E-06 | 5.56E-06 | 2.54E-07 |
| isot                | 34 Se 74 | 2.07E-09 | 2.63E-07 | 2.14E-06 | 2.30E-06 | 9.91E-08 | 1.87E-09 | 2.61E-07 | 1.98E-06 | 2.18E-06 | 9.05E-08 |
| isot                | 34 Se 76 | 5.33E-10 | 1.18E-07 | 2.62E-06 | 3.26E-06 | 1.45E-07 | 5.00E-10 | 1.28E-07 | 2.54E-06 | 3.11E-06 | 1.28E-07 |
| isot                | 34 Se 77 | 1.81E-10 | 1.51E-09 | 1.04E-08 | 3.18E-08 | 1.27E-08 | 1.55E-10 | 1.51E-09 | 1.05E-08 | 2.93E-08 | 1.03E-08 |
| isot                | 34 Se 78 | 1.88E-11 | 7.96E-10 | 9.19E-08 | 2.46E-07 | 2.26E-08 | 1.51E-11 | 8.01E-10 | 9.10E-08 | 2.35E-07 | 1.83E-08 |
| isot                | 34 Se 80 | 2.92E-11 | 1.44E-10 | 1.68E-09 | 6.79E-09 | 9.07E-09 | 2.26E-11 | 1.13E-10 | 1.51E-09 | 6.21E-09 | 6.83E-09 |
| elem                | 35 Br    | 3.78E-11 | 3.55E-09 | 3.67E-08 | 3.46E-08 | 3.76E-09 | 3.24E-11 | 3.78E-09 | 3.91E-08 | 3.48E-08 | 2.83E-09 |
| isot                | 35 Br 79 | 3.78E-11 | 3.55E-09 | 3.67E-08 | 3.46E-08 | 3.76E-09 | 3.24E-11 | 3.78E-09 | 3.91E-08 | 3.48E-08 | 2.83E-09 |
| elem                | 36 Kr    | 1.47E-09 | 1.16E-07 | 1.35E-06 | 6.57E-07 | 1.31E-08 | 1.36E-09 | 1.34E-07 | 1.44E-06 | 6.52E-07 | 1.11E-08 |
| isot                | 36 Kr 78 | 1.24E-09 | 5.28E-08 | 2.66E-07 | 1.15E-07 | 2.29E-09 | 1.16E-09 | 5.85E-08 | 2.83E-07 | 1.16E-07 | 1.90E-09 |
| isot                | 36 Kr 80 | 2.23E-10 | 6.32E-08 | 1.08E-06 | 5.42E-07 | 1.08E-08 | 2.07E-10 | 7.58E-08 | 1.15E-06 | 5.36E-07 | 9.18E-09 |

Table A1 *continued*.

|                     |          |          |          |          |          |          |
|---------------------|----------|----------|----------|----------|----------|----------|
| $\rho_{\text{DDT}}$ |          | 4.0E+07  | 4.0E+07  | 4.0E+07  | 4.0E+07  | 4.0E+07  |
| Z                   |          | 2.25E-4  | 2.25E-3  | 9.00E-3  | 2.25E-2  | 6.75E-2  |
| elem                | 2 He     | 8.58E-03 | 8.66E-03 | 8.05E-03 | 7.53E-03 | 5.83E-03 |
| isot                | 2 He 3   | 1.86E-12 | 1.84E-12 | 1.70E-12 | 1.67E-12 | 1.28E-12 |
| isot                | 2 He 4   | 8.58E-03 | 8.65E-03 | 8.05E-03 | 7.53E-03 | 5.83E-03 |
| elem                | 6 C      | 5.43E-04 | 5.41E-04 | 5.56E-04 | 5.40E-04 | 5.23E-04 |
| isot                | 6 C 12   | 5.43E-04 | 5.41E-04 | 5.56E-04 | 5.40E-04 | 5.23E-04 |
| isot                | 6 C 13   | 3.38E-11 | 4.65E-10 | 2.20E-09 | 5.26E-09 | 1.21E-08 |
| elem                | 7 N      | 4.55E-06 | 3.71E-06 | 2.64E-06 | 1.58E-06 | 5.81E-07 |
| isot                | 7 N 14   | 4.54E-06 | 3.71E-06 | 2.64E-06 | 1.58E-06 | 5.81E-07 |
| isot                | 7 N 15   | 1.68E-08 | 5.43E-10 | 2.97E-10 | 3.38E-10 | 4.93E-10 |
| elem                | 8 O      | 3.34E-02 | 3.43E-02 | 3.64E-02 | 3.69E-02 | 3.75E-02 |
| isot                | 8 O 16   | 3.33E-02 | 3.43E-02 | 3.64E-02 | 3.69E-02 | 3.75E-02 |
| isot                | 8 O 17   | 1.50E-09 | 1.23E-08 | 2.44E-08 | 3.06E-08 | 2.84E-08 |
| isot                | 8 O 18   | 4.68E-10 | 2.05E-10 | 1.74E-10 | 1.67E-10 | 1.69E-10 |
| elem                | 9 F      | 2.83E-12 | 8.63E-13 | 1.51E-12 | 3.61E-12 | 1.17E-11 |
| isot                | 9 F 19   | 2.83E-12 | 8.63E-13 | 1.51E-12 | 3.61E-12 | 1.17E-11 |
| elem                | 10 Ne    | 2.64E-04 | 2.56E-04 | 2.69E-04 | 2.63E-04 | 2.76E-04 |
| isot                | 10 Ne 20 | 2.64E-04 | 2.56E-04 | 2.67E-04 | 2.58E-04 | 2.51E-04 |
| isot                | 10 Ne 21 | 1.30E-08 | 5.58E-09 | 1.54E-08 | 3.79E-08 | 1.46E-07 |
| isot                | 10 Ne 22 | 1.91E-07 | 2.70E-07 | 1.54E-06 | 5.20E-06 | 2.41E-05 |
| elem                | 11 Na    | 1.81E-06 | 1.90E-06 | 2.63E-06 | 4.14E-06 | 1.01E-05 |
| isot                | 11 Na 23 | 1.81E-06 | 1.90E-06 | 2.63E-06 | 4.14E-06 | 1.01E-05 |
| elem                | 12 Mg    | 5.05E-03 | 4.40E-03 | 3.31E-03 | 2.21E-03 | 1.25E-03 |
| isot                | 12 Mg 24 | 5.05E-03 | 4.40E-03 | 3.31E-03 | 2.19E-03 | 1.20E-03 |
| isot                | 12 Mg 25 | 2.33E-07 | 1.19E-06 | 2.90E-06 | 6.44E-06 | 1.86E-05 |
| isot                | 12 Mg 26 | 1.76E-06 | 9.44E-07 | 3.84E-06 | 9.83E-06 | 3.53E-05 |
| elem                | 13 Al    | 1.09E-05 | 4.04E-05 | 7.65E-05 | 8.63E-05 | 8.34E-05 |
| isot                | 13 Al 27 | 1.09E-05 | 4.04E-05 | 7.65E-05 | 8.63E-05 | 8.34E-05 |
| elem                | 14 Si    | 1.52E-01 | 1.54E-01 | 1.61E-01 | 1.61E-01 | 1.57E-01 |
| isot                | 14 Si 28 | 1.52E-01 | 1.54E-01 | 1.61E-01 | 1.61E-01 | 1.56E-01 |
| isot                | 14 Si 29 | 3.48E-05 | 8.38E-05 | 1.31E-04 | 1.87E-04 | 4.15E-04 |
| isot                | 14 Si 30 | 1.44E-05 | 3.11E-05 | 1.58E-04 | 3.77E-04 | 1.33E-03 |
| elem                | 15 P     | 1.87E-05 | 2.91E-05 | 7.26E-05 | 1.30E-04 | 3.08E-04 |
| isot                | 15 P 31  | 1.87E-05 | 2.91E-05 | 7.26E-05 | 1.30E-04 | 3.08E-04 |
| elem                | 16 S     | 9.59E-02 | 9.42E-02 | 9.51E-02 | 9.10E-02 | 7.59E-02 |
| isot                | 16 S 32  | 9.59E-02 | 9.41E-02 | 9.45E-02 | 8.95E-02 | 7.11E-02 |
| isot                | 16 S 33  | 1.55E-05 | 3.52E-05 | 7.24E-05 | 1.13E-04 | 2.16E-04 |
| isot                | 16 S 34  | 7.80E-06 | 9.03E-05 | 4.91E-04 | 1.33E-03 | 4.61E-03 |
| isot                | 16 S 36  | 1.09E-10 | 1.08E-09 | 1.11E-08 | 6.54E-08 | 1.60E-06 |
| elem                | 17 Cl    | 8.36E-06 | 1.44E-05 | 3.72E-05 | 7.33E-05 | 1.53E-04 |
| isot                | 17 Cl 35 | 6.49E-06 | 1.02E-05 | 2.86E-05 | 5.91E-05 | 1.26E-04 |
| isot                | 17 Cl 37 | 1.87E-06 | 4.23E-06 | 8.61E-06 | 1.42E-05 | 2.69E-05 |
| elem                | 18 Ar    | 2.29E-02 | 2.19E-02 | 2.12E-02 | 1.95E-02 | 1.59E-02 |
| isot                | 18 Ar 36 | 2.29E-02 | 2.19E-02 | 2.09E-02 | 1.88E-02 | 1.35E-02 |
| isot                | 18 Ar 38 | 1.63E-06 | 4.06E-05 | 2.45E-04 | 7.29E-04 | 2.46E-03 |
| isot                | 18 Ar 40 | 1.24E-11 | 1.86E-10 | 2.18E-09 | 9.99E-09 | 1.14E-07 |
| elem                | 19 K     | 3.03E-06 | 9.03E-06 | 2.80E-05 | 5.16E-05 | 9.24E-05 |
| isot                | 19 K 39  | 2.65E-06 | 8.21E-06 | 2.61E-05 | 4.86E-05 | 8.78E-05 |
| isot                | 19 K 40  | 2.27E-11 | 7.90E-10 | 5.48E-09 | 2.78E-08 | 8.55E-08 |
| isot                | 19 K 41  | 3.83E-07 | 8.23E-07 | 1.81E-06 | 2.98E-06 | 4.57E-06 |
| elem                | 20 Ca    | 2.50E-02 | 2.36E-02 | 2.20E-02 | 1.93E-02 | 1.38E-02 |
| isot                | 20 Ca 40 | 2.50E-02 | 2.35E-02 | 2.19E-02 | 1.92E-02 | 1.37E-02 |
| isot                | 20 Ca 42 | 1.32E-08 | 8.25E-07 | 5.69E-06 | 1.81E-05 | 5.72E-05 |
| isot                | 20 Ca 43 | 5.46E-08 | 8.03E-08 | 4.06E-07 | 3.37E-07 | 2.70E-07 |
| isot                | 20 Ca 44 | 3.54E-05 | 4.45E-05 | 4.65E-05 | 4.02E-05 | 2.45E-05 |
| isot                | 20 Ca 46 | 3.45E-09 | 3.60E-09 | 4.66E-09 | 8.88E-09 | 5.75E-08 |
| isot                | 20 Ca 48 | 1.56E-08 | 1.64E-08 | 1.87E-08 | 2.90E-08 | 8.89E-08 |
| elem                | 21 Sc    | 6.69E-08 | 8.74E-08 | 1.34E-07 | 1.99E-07 | 3.65E-07 |
| isot                | 21 Sc 45 | 6.69E-08 | 8.74E-08 | 1.34E-07 | 1.99E-07 | 3.65E-07 |

Table A1 *continued*.

|                     |          |          |          |          |          |          |
|---------------------|----------|----------|----------|----------|----------|----------|
| $\rho_{\text{DDT}}$ |          | 4.0E+07  | 4.0E+07  | 4.0E+07  | 4.0E+07  | 4.0E+07  |
| Z                   |          | 2.25E-4  | 2.25E-3  | 9.00E-3  | 2.25E-2  | 6.75E-2  |
| elem                | 22 Ti    | 6.87E-04 | 6.90E-04 | 6.94E-04 | 6.90E-04 | 7.25E-04 |
| isot                | 22 Ti 46 | 6.42E-06 | 1.06E-06 | 4.65E-06 | 1.24E-05 | 3.24E-05 |
| isot                | 22 Ti 47 | 7.62E-06 | 5.00E-07 | 9.07E-07 | 1.26E-06 | 1.72E-06 |
| isot                | 22 Ti 48 | 3.79E-04 | 3.85E-04 | 3.64E-04 | 3.17E-04 | 2.14E-04 |
| isot                | 22 Ti 49 | 4.34E-06 | 9.72E-06 | 1.47E-05 | 2.00E-05 | 2.42E-05 |
| isot                | 22 Ti 50 | 2.90E-04 | 2.94E-04 | 3.09E-04 | 3.40E-04 | 4.53E-04 |
| elem                | 23 V     | 6.36E-05 | 7.12E-05 | 9.53E-05 | 1.24E-04 | 1.80E-04 |
| isot                | 23 V 50  | 1.65E-08 | 1.67E-08 | 1.83E-08 | 2.70E-08 | 8.28E-08 |
| isot                | 23 V 51  | 6.36E-05 | 7.12E-05 | 9.53E-05 | 1.23E-04 | 1.80E-04 |
| elem                | 24 Cr    | 1.52E-02 | 1.51E-02 | 1.50E-02 | 1.48E-02 | 1.50E-02 |
| isot                | 24 Cr 50 | 8.98E-05 | 7.73E-05 | 1.42E-04 | 3.00E-04 | 8.98E-04 |
| isot                | 24 Cr 52 | 1.26E-02 | 1.23E-02 | 1.18E-02 | 1.10E-02 | 9.63E-03 |
| isot                | 24 Cr 53 | 5.65E-04 | 7.79E-04 | 1.01E-03 | 1.28E-03 | 1.72E-03 |
| isot                | 24 Cr 54 | 1.94E-03 | 1.96E-03 | 2.04E-03 | 2.20E-03 | 2.76E-03 |
| elem                | 25 Mn    | 4.33E-03 | 5.58E-03 | 7.76E-03 | 1.04E-02 | 1.52E-02 |
| isot                | 25 Mn 55 | 4.33E-03 | 5.58E-03 | 7.76E-03 | 1.04E-02 | 1.52E-02 |
| elem                | 26 Fe    | 9.75E-01 | 9.76E-01 | 9.57E-01 | 9.40E-01 | 8.81E-01 |
| isot                | 26 Fe 54 | 3.67E-02 | 3.89E-02 | 4.80E-02 | 6.69E-02 | 1.23E-01 |
| isot                | 26 Fe 56 | 9.24E-01 | 9.19E-01 | 8.88E-01 | 8.47E-01 | 7.22E-01 |
| isot                | 26 Fe 57 | 8.84E-03 | 1.26E-02 | 1.58E-02 | 2.04E-02 | 2.95E-02 |
| isot                | 26 Fe 58 | 4.79E-03 | 4.84E-03 | 5.00E-03 | 5.32E-03 | 6.36E-03 |
| elem                | 27 Co    | 1.70E-03 | 4.04E-04 | 7.38E-04 | 1.01E-03 | 1.39E-03 |
| isot                | 27 Co 59 | 1.70E-03 | 4.04E-04 | 7.38E-04 | 1.01E-03 | 1.39E-03 |
| elem                | 28 Ni    | 3.63E-02 | 3.65E-02 | 4.49E-02 | 6.54E-02 | 1.36E-01 |
| isot                | 28 Ni 58 | 1.99E-02 | 1.90E-02 | 2.77E-02 | 4.71E-02 | 1.15E-01 |
| isot                | 28 Ni 60 | 1.49E-02 | 1.56E-02 | 1.41E-02 | 1.30E-02 | 1.01E-02 |
| isot                | 28 Ni 61 | 1.15E-04 | 2.78E-04 | 3.40E-04 | 4.18E-04 | 5.05E-04 |
| isot                | 28 Ni 62 | 1.38E-03 | 1.54E-03 | 2.75E-03 | 4.81E-03 | 1.02E-02 |
| isot                | 28 Ni 64 | 3.52E-05 | 3.62E-05 | 3.97E-05 | 4.78E-05 | 8.63E-05 |
| elem                | 29 Cu    | 1.57E-04 | 2.73E-05 | 4.14E-06 | 7.20E-06 | 1.66E-05 |
| isot                | 29 Cu 63 | 1.57E-04 | 2.55E-05 | 2.03E-06 | 3.55E-06 | 8.25E-06 |
| isot                | 29 Cu 65 | 5.36E-07 | 1.77E-06 | 2.11E-06 | 3.65E-06 | 8.33E-06 |
| elem                | 30 Zn    | 2.84E-04 | 3.05E-04 | 9.90E-05 | 1.35E-04 | 1.92E-04 |
| isot                | 30 Zn 64 | 2.75E-04 | 2.93E-04 | 6.15E-05 | 4.50E-05 | 2.37E-05 |
| isot                | 30 Zn 66 | 8.69E-07 | 1.09E-05 | 3.70E-05 | 8.73E-05 | 1.63E-04 |
| isot                | 30 Zn 67 | 1.77E-06 | 2.23E-07 | 1.06E-07 | 3.02E-07 | 1.00E-06 |
| isot                | 30 Zn 68 | 5.91E-06 | 1.07E-06 | 3.84E-07 | 2.27E-06 | 4.23E-06 |
| isot                | 30 Zn 70 | 2.56E-10 | 3.84E-10 | 2.73E-09 | 2.24E-08 | 8.33E-08 |
| elem                | 31 Ga    | 4.98E-09 | 2.98E-08 | 2.37E-07 | 1.06E-06 | 6.72E-07 |
| isot                | 31 Ga 69 | 2.58E-09 | 2.68E-08 | 1.96E-07 | 8.25E-07 | 4.54E-07 |
| isot                | 31 Ga 71 | 2.40E-09 | 3.06E-09 | 4.03E-08 | 2.39E-07 | 2.18E-07 |
| elem                | 32 Ge    | 2.29E-07 | 7.38E-07 | 4.81E-06 | 1.02E-05 | 3.65E-06 |
| isot                | 32 Ge 70 | 1.25E-07 | 6.56E-07 | 3.49E-06 | 5.90E-06 | 2.64E-06 |
| isot                | 32 Ge 72 | 1.04E-07 | 7.75E-08 | 1.26E-06 | 4.07E-06 | 9.25E-07 |
| isot                | 32 Ge 73 | 1.89E-10 | 4.46E-09 | 3.60E-08 | 4.09E-08 | 1.79E-08 |
| isot                | 32 Ge 74 | 2.37E-11 | 2.33E-10 | 1.30E-08 | 1.56E-07 | 6.89E-08 |
| isot                | 32 Ge 76 | 6.94E-12 | 2.62E-11 | 5.45E-10 | 3.02E-09 | 4.19E-09 |
| elem                | 33 As    | 6.06E-11 | 4.48E-09 | 5.35E-08 | 2.18E-07 | 3.42E-08 |
| isot                | 33 As 75 | 6.06E-11 | 4.48E-09 | 5.35E-08 | 2.18E-07 | 3.42E-08 |
| elem                | 34 Se    | 2.28E-09 | 3.56E-07 | 3.75E-06 | 4.58E-06 | 2.01E-07 |
| isot                | 34 Se 74 | 1.68E-09 | 2.23E-07 | 1.53E-06 | 1.78E-06 | 7.72E-08 |
| isot                | 34 Se 76 | 4.74E-10 | 1.31E-07 | 2.12E-06 | 2.58E-06 | 1.02E-07 |
| isot                | 34 Se 77 | 1.08E-10 | 1.47E-09 | 1.03E-08 | 2.30E-08 | 6.34E-09 |
| isot                | 34 Se 78 | 9.17E-12 | 8.37E-10 | 8.25E-08 | 2.02E-07 | 1.17E-08 |
| isot                | 34 Se 80 | 1.28E-11 | 6.21E-11 | 1.28E-09 | 4.80E-09 | 3.37E-09 |
| elem                | 35 Br    | 2.72E-11 | 4.07E-09 | 3.96E-08 | 3.46E-08 | 1.75E-09 |
| isot                | 35 Br 79 | 2.72E-11 | 4.07E-09 | 3.96E-08 | 3.46E-08 | 1.75E-09 |
| elem                | 36 Kr    | 1.20E-09 | 1.61E-07 | 1.44E-06 | 6.64E-07 | 7.94E-09 |
| isot                | 36 Kr 78 | 9.85E-10 | 6.46E-08 | 2.87E-07 | 1.25E-07 | 1.42E-09 |
| isot                | 36 Kr 80 | 2.19E-10 | 9.63E-08 | 1.15E-06 | 5.39E-07 | 6.51E-09 |



Table A2. Nucleosynthesis in sub-Chandrasekhar models with the standard  $^{12}\text{C}+^{16}\text{O}$  reaction rate.

| $M_{\text{WD}}$ |          | 0.88     | 0.88     | 0.88     | 0.88     | 0.88     | 0.97     | 0.97     | 0.97     | 0.97     | 0.97     |
|-----------------|----------|----------|----------|----------|----------|----------|----------|----------|----------|----------|----------|
| Z               |          | 2.25E-4  | 2.25E-3  | 9.00E-3  | 2.25E-2  | 6.75E-2  | 2.25E-4  | 2.25E-3  | 9.00E-3  | 2.25E-2  | 6.75E-2  |
| elem            | 2 He     | 9.87E-08 | 9.71E-08 | 7.65E-08 | 3.33E-08 | 2.92E-10 | 2.25E-04 | 2.39E-04 | 2.72E-04 | 3.35E-04 | 4.93E-04 |
| isot            | 2 He 3   | 1.97E-16 | 1.97E-16 | 1.99E-16 | 2.04E-16 | 2.39E-16 | 7.16E-16 | 7.09E-16 | 6.89E-16 | 6.52E-16 | 5.39E-16 |
| isot            | 2 He 4   | 9.87E-08 | 9.71E-08 | 7.65E-08 | 3.33E-08 | 2.92E-10 | 2.25E-04 | 2.39E-04 | 2.72E-04 | 3.35E-04 | 4.93E-04 |
| elem            | 6 C      | 4.10E-03 | 4.08E-03 | 3.99E-03 | 3.83E-03 | 3.33E-03 | 1.67E-03 | 1.66E-03 | 1.63E-03 | 1.56E-03 | 1.36E-03 |
| isot            | 6 C 12   | 4.10E-03 | 4.08E-03 | 3.99E-03 | 3.83E-03 | 3.33E-03 | 1.67E-03 | 1.66E-03 | 1.62E-03 | 1.55E-03 | 1.36E-03 |
| isot            | 6 C 13   | 2.25E-10 | 3.71E-09 | 1.23E-08 | 2.61E-08 | 5.62E-08 | 9.58E-11 | 1.53E-09 | 5.68E-09 | 1.28E-08 | 2.83E-08 |
| elem            | 7 N      | 8.41E-06 | 6.92E-06 | 5.30E-06 | 4.02E-06 | 2.72E-06 | 7.19E-06 | 5.84E-06 | 4.11E-06 | 2.60E-06 | 1.15E-06 |
| isot            | 7 N 14   | 8.31E-06 | 6.92E-06 | 5.30E-06 | 4.02E-06 | 2.71E-06 | 7.15E-06 | 5.84E-06 | 4.11E-06 | 2.60E-06 | 1.15E-06 |
| isot            | 7 N 15   | 9.83E-08 | 2.92E-09 | 1.93E-09 | 2.77E-09 | 3.50E-09 | 3.79E-08 | 1.13E-09 | 7.20E-10 | 9.81E-10 | 1.23E-09 |
| elem            | 8 O      | 1.35E-01 | 1.36E-01 | 1.37E-01 | 1.38E-01 | 1.29E-01 | 7.22E-02 | 7.35E-02 | 7.39E-02 | 7.40E-02 | 6.83E-02 |
| isot            | 8 O 16   | 1.35E-01 | 1.36E-01 | 1.37E-01 | 1.38E-01 | 1.29E-01 | 7.22E-02 | 7.35E-02 | 7.38E-02 | 7.40E-02 | 6.83E-02 |
| isot            | 8 O 17   | 7.23E-09 | 1.04E-07 | 2.24E-07 | 2.99E-07 | 2.87E-07 | 3.54E-09 | 3.79E-08 | 7.69E-08 | 9.93E-08 | 8.42E-08 |
| isot            | 8 O 18   | 1.92E-09 | 1.54E-09 | 1.69E-09 | 2.01E-09 | 1.81E-09 | 6.49E-10 | 5.15E-10 | 5.43E-10 | 6.06E-10 | 5.14E-10 |
| elem            | 9 F      | 3.65E-11 | 9.22E-12 | 1.03E-11 | 2.43E-11 | 7.62E-11 | 1.06E-11 | 2.52E-12 | 3.97E-12 | 1.02E-11 | 3.06E-11 |
| isot            | 9 F 19   | 3.65E-11 | 9.22E-12 | 1.03E-11 | 2.43E-11 | 7.62E-11 | 1.06E-11 | 2.52E-12 | 3.97E-12 | 1.02E-11 | 3.06E-11 |
| elem            | 10 Ne    | 2.69E-03 | 2.65E-03 | 2.59E-03 | 2.51E-03 | 2.27E-03 | 8.65E-04 | 8.53E-04 | 8.32E-04 | 8.01E-04 | 7.32E-04 |
| isot            | 10 Ne 20 | 2.69E-03 | 2.65E-03 | 2.57E-03 | 2.46E-03 | 2.07E-03 | 8.65E-04 | 8.52E-04 | 8.25E-04 | 7.81E-04 | 6.53E-04 |
| isot            | 10 Ne 21 | 6.26E-09 | 4.21E-08 | 1.23E-07 | 2.75E-07 | 9.24E-07 | 2.37E-09 | 1.56E-08 | 4.92E-08 | 1.16E-07 | 3.78E-07 |
| isot            | 10 Ne 22 | 2.29E-07 | 2.96E-06 | 1.56E-05 | 4.94E-05 | 1.92E-04 | 9.67E-08 | 1.19E-06 | 6.14E-06 | 1.95E-05 | 7.81E-05 |
| elem            | 11 Na    | 1.69E-05 | 1.86E-05 | 2.34E-05 | 3.42E-05 | 6.99E-05 | 5.79E-06 | 6.32E-06 | 8.18E-06 | 1.25E-05 | 2.64E-05 |
| isot            | 11 Na 23 | 1.69E-05 | 1.86E-05 | 2.34E-05 | 3.42E-05 | 6.99E-05 | 5.79E-06 | 6.32E-06 | 8.18E-06 | 1.25E-05 | 2.64E-05 |
| elem            | 12 Mg    | 3.24E-02 | 2.90E-02 | 2.19E-02 | 1.52E-02 | 7.64E-03 | 1.35E-02 | 1.20E-02 | 8.74E-03 | 5.85E-03 | 2.87E-03 |
| isot            | 12 Mg 24 | 3.24E-02 | 2.90E-02 | 2.18E-02 | 1.51E-02 | 7.25E-03 | 1.35E-02 | 1.20E-02 | 8.72E-03 | 5.81E-03 | 2.73E-03 |
| isot            | 12 Mg 25 | 8.70E-07 | 9.33E-06 | 2.29E-05 | 5.33E-05 | 1.44E-04 | 3.94E-07 | 3.55E-06 | 8.60E-06 | 1.95E-05 | 5.06E-05 |
| isot            | 12 Mg 26 | 9.34E-07 | 6.88E-06 | 2.99E-05 | 7.61E-05 | 2.50E-04 | 3.42E-07 | 2.62E-06 | 1.15E-05 | 2.88E-05 | 9.00E-05 |
| elem            | 13 Al    | 8.49E-05 | 2.84E-04 | 5.50E-04 | 6.49E-04 | 5.69E-04 | 3.08E-05 | 1.12E-04 | 2.08E-04 | 2.37E-04 | 2.01E-04 |
| isot            | 13 Al 27 | 8.49E-05 | 2.84E-04 | 5.50E-04 | 6.49E-04 | 5.69E-04 | 3.08E-05 | 1.12E-04 | 2.08E-04 | 2.37E-04 | 2.01E-04 |
| elem            | 14 Si    | 3.14E-01 | 3.24E-01 | 3.29E-01 | 3.28E-01 | 3.10E-01 | 2.38E-01 | 2.44E-01 | 2.47E-01 | 2.45E-01 | 2.29E-01 |
| isot            | 14 Si 28 | 3.14E-01 | 3.23E-01 | 3.28E-01 | 3.25E-01 | 3.02E-01 | 2.38E-01 | 2.43E-01 | 2.47E-01 | 2.44E-01 | 2.25E-01 |
| isot            | 14 Si 29 | 1.32E-04 | 3.76E-04 | 5.57E-04 | 8.77E-04 | 1.90E-03 | 6.87E-05 | 1.95E-04 | 2.81E-04 | 4.07E-04 | 8.20E-04 |
| isot            | 14 Si 30 | 1.41E-05 | 1.46E-04 | 8.66E-04 | 2.15E-03 | 6.42E-03 | 5.72E-06 | 7.02E-05 | 3.85E-04 | 9.20E-04 | 2.77E-03 |
| elem            | 15 P     | 3.15E-05 | 9.66E-05 | 2.76E-04 | 5.21E-04 | 1.11E-03 | 2.23E-05 | 5.53E-05 | 1.46E-04 | 2.63E-04 | 5.54E-04 |
| isot            | 15 P 31  | 3.15E-05 | 9.56E-05 | 2.76E-04 | 5.21E-04 | 1.11E-03 | 2.23E-05 | 5.53E-05 | 1.46E-04 | 2.63E-04 | 5.54E-04 |
| elem            | 16 S     | 1.66E-01 | 1.64E-01 | 1.65E-01 | 1.60E-01 | 1.35E-01 | 1.39E-01 | 1.37E-01 | 1.36E-01 | 1.30E-01 | 1.05E-01 |
| isot            | 16 S 32  | 1.66E-01 | 1.64E-01 | 1.63E-01 | 1.56E-01 | 1.22E-01 | 1.39E-01 | 1.37E-01 | 1.35E-01 | 1.27E-01 | 9.71E-02 |
| isot            | 16 S 33  | 6.12E-05 | 1.13E-04 | 2.25E-04 | 3.38E-04 | 5.28E-04 | 3.30E-05 | 6.80E-05 | 1.32E-04 | 2.03E-04 | 3.38E-04 |
| isot            | 16 S 34  | 1.10E-06 | 2.53E-04 | 1.43E-03 | 3.99E-03 | 1.27E-02 | 8.89E-07 | 1.73E-04 | 9.32E-04 | 2.52E-03 | 7.92E-03 |
| isot            | 16 S 36  | 2.51E-11 | 6.18E-09 | 6.70E-08 | 3.89E-07 | 9.69E-06 | 1.17E-11 | 2.82E-09 | 2.98E-08 | 1.68E-07 | 3.66E-06 |
| elem            | 17 Cl    | 8.76E-06 | 2.77E-05 | 8.44E-05 | 1.81E-04 | 3.44E-04 | 7.67E-06 | 2.19E-05 | 6.03E-05 | 1.22E-04 | 2.33E-04 |
| isot            | 17 Cl 35 | 3.94E-06 | 1.95E-05 | 6.71E-05 | 1.52E-04 | 2.90E-04 | 4.30E-06 | 1.53E-05 | 4.69E-05 | 9.99E-05 | 1.94E-04 |
| isot            | 17 Cl 37 | 4.82E-06 | 8.22E-06 | 1.73E-05 | 2.87E-05 | 5.38E-05 | 3.37E-06 | 6.66E-06 | 1.34E-05 | 2.22E-05 | 3.94E-05 |
| elem            | 18 Ar    | 3.47E-02 | 3.30E-02 | 3.15E-02 | 2.93E-02 | 2.49E-02 | 3.13E-02 | 2.99E-02 | 2.83E-02 | 2.61E-02 | 2.12E-02 |
| isot            | 18 Ar 36 | 3.47E-02 | 3.30E-02 | 3.09E-02 | 2.76E-02 | 1.93E-02 | 3.12E-02 | 2.98E-02 | 2.79E-02 | 2.49E-02 | 1.71E-02 |
| isot            | 18 Ar 38 | 9.58E-07 | 9.37E-05 | 5.75E-04 | 1.75E-03 | 5.61E-03 | 9.15E-07 | 7.48E-05 | 4.31E-04 | 1.29E-03 | 4.07E-03 |
| isot            | 18 Ar 40 | 1.51E-11 | 1.37E-09 | 1.71E-08 | 7.78E-08 | 7.55E-07 | 5.79E-12 | 6.08E-10 | 7.21E-09 | 3.06E-08 | 2.77E-07 |
| elem            | 19 K     | 2.46E-06 | 1.53E-05 | 4.89E-05 | 9.64E-05 | 1.68E-04 | 2.74E-06 | 1.39E-05 | 4.01E-05 | 7.77E-05 | 1.34E-04 |
| isot            | 19 K 39  | 1.97E-06 | 1.40E-05 | 4.57E-05 | 9.10E-05 | 1.59E-04 | 2.23E-06 | 1.27E-05 | 3.75E-05 | 7.33E-05 | 1.28E-04 |
| isot            | 19 K 40  | 6.51E-11 | 2.38E-09 | 1.72E-08 | 1.01E-07 | 3.05E-07 | 4.75E-11 | 1.46E-09 | 9.60E-09 | 5.09E-08 | 1.48E-07 |
| isot            | 19 K 41  | 4.95E-07 | 1.31E-06 | 3.17E-06 | 5.37E-06 | 7.98E-06 | 5.09E-07 | 1.19E-06 | 2.63E-06 | 4.37E-06 | 6.36E-06 |
| elem            | 20 Ca    | 3.38E-02 | 3.11E-02 | 2.80E-02 | 2.43E-02 | 1.73E-02 | 3.29E-02 | 3.08E-02 | 2.79E-02 | 2.43E-02 | 1.68E-02 |
| isot            | 20 Ca 40 | 3.38E-02 | 3.11E-02 | 2.80E-02 | 2.42E-02 | 1.72E-02 | 3.29E-02 | 3.08E-02 | 2.79E-02 | 2.43E-02 | 1.67E-02 |
| isot            | 20 Ca 42 | 1.53E-08 | 1.65E-06 | 1.19E-05 | 3.91E-05 | 1.21E-04 | 1.40E-08 | 1.43E-06 | 9.45E-06 | 3.06E-05 | 9.22E-05 |
| isot            | 20 Ca 43 | 4.41E-10 | 3.31E-09 | 2.83E-08 | 1.29E-07 | 6.14E-07 | 6.34E-10 | 1.98E-09 | 1.56E-08 | 6.89E-08 | 3.14E-07 |
| isot            | 20 Ca 44 | 1.85E-05 | 1.66E-05 | 1.47E-05 | 1.29E-05 | 1.17E-05 | 2.27E-05 | 2.05E-05 | 1.82E-05 | 1.59E-05 | 1.24E-05 |
| isot            | 20 Ca 46 | 2.32E-12 | 6.34E-10 | 8.00E-09 | 4.09E-08 | 4.60E-07 | 8.57E-13 | 2.77E-10 | 3.24E-09 | 1.51E-08 | 1.44E-07 |
| isot            | 20 Ca 48 | 1.26E-11 | 1.23E-10 | 1.43E-09 | 9.38E-09 | 1.03E-07 | 4.75E-12 | 4.93E-11 | 6.30E-10 | 3.79E-09 | 3.66E-08 |
| elem            | 21 Sc    | 6.17E-08 | 9.79E-08 | 1.88E-07 | 3.60E-07 | 1.04E-06 | 6.44E-08 | 9.61E-08 | 1.62E-07 | 2.59E-07 | 5.46E-07 |
| isot            | 21 Sc 45 | 6.17E-08 | 9.79E-08 | 1.88E-07 | 3.60E-07 | 1.04E-06 | 6.44E-08 | 9.61E-08 | 1.62E-07 | 2.59E-07 | 5.46E-07 |

Table A2 continued.

| $M_{\text{WD}}$ |          | 0.88     | 0.88     | 0.88     | 0.88     | 0.88     | 0.97     | 0.97     | 0.97     | 0.97     | 0.97     |
|-----------------|----------|----------|----------|----------|----------|----------|----------|----------|----------|----------|----------|
| Z               |          | 2.25E-4  | 2.25E-3  | 9.00E-3  | 2.25E-2  | 6.75E-2  | 2.25E-4  | 2.25E-3  | 9.00E-3  | 2.25E-2  | 6.75E-2  |
| elem            | 22 Ti    | 2.93E-04 | 2.80E-04 | 2.64E-04 | 2.51E-04 | 2.56E-04 | 4.14E-04 | 4.03E-04 | 3.81E-04 | 3.51E-04 | 2.88E-04 |
| isot            | 22 Ti 46 | 4.64E-08 | 1.45E-06 | 8.90E-06 | 2.44E-05 | 6.11E-05 | 4.91E-08 | 1.34E-06 | 7.31E-06 | 1.98E-05 | 4.87E-05 |
| isot            | 22 Ti 47 | 4.34E-09 | 1.09E-08 | 1.48E-07 | 7.19E-07 | 3.09E-06 | 2.28E-08 | 8.14E-09 | 1.02E-07 | 4.61E-07 | 1.86E-06 |
| isot            | 22 Ti 48 | 2.88E-04 | 2.72E-04 | 2.43E-04 | 2.10E-04 | 1.67E-04 | 4.08E-04 | 3.93E-04 | 3.59E-04 | 3.11E-04 | 2.12E-04 |
| isot            | 22 Ti 49 | 5.01E-06 | 7.08E-06 | 1.16E-05 | 1.59E-05 | 2.09E-05 | 6.17E-06 | 9.12E-06 | 1.47E-05 | 2.03E-05 | 2.43E-05 |
| isot            | 22 Ti 50 | 3.51E-11 | 1.12E-09 | 8.86E-09 | 1.12E-07 | 3.85E-06 | 1.37E-11 | 4.14E-10 | 3.70E-09 | 4.19E-08 | 1.36E-06 |
| elem            | 23 V     | 2.21E-06 | 1.06E-05 | 2.92E-05 | 5.15E-05 | 1.11E-04 | 2.13E-06 | 1.40E-05 | 3.76E-05 | 6.49E-05 | 1.19E-04 |
| isot            | 23 V 50  | 2.15E-11 | 3.27E-10 | 8.81E-09 | 8.48E-08 | 3.61E-07 | 7.16E-12 | 1.38E-10 | 3.22E-09 | 2.73E-08 | 1.37E-07 |
| isot            | 23 V 51  | 2.21E-06 | 1.06E-05 | 2.92E-05 | 5.14E-05 | 1.11E-04 | 2.13E-06 | 1.40E-05 | 3.76E-05 | 6.49E-05 | 1.18E-04 |
| elem            | 24 Cr    | 6.01E-03 | 5.84E-03 | 5.62E-03 | 5.53E-03 | 7.26E-03 | 1.09E-02 | 1.07E-02 | 1.03E-02 | 9.63E-03 | 9.17E-03 |
| isot            | 24 Cr 50 | 1.54E-06 | 2.29E-05 | 1.12E-04 | 3.34E-04 | 1.18E-03 | 1.34E-06 | 2.11E-05 | 1.06E-04 | 3.08E-04 | 1.04E-03 |
| isot            | 24 Cr 52 | 5.84E-03 | 5.58E-03 | 5.10E-03 | 4.62E-03 | 5.00E-03 | 1.06E-02 | 1.03E-02 | 9.50E-03 | 8.39E-03 | 6.73E-03 |
| isot            | 24 Cr 53 | 1.69E-04 | 2.41E-04 | 4.04E-04 | 5.78E-04 | 1.08E-03 | 2.87E-04 | 3.97E-04 | 6.50E-04 | 9.25E-04 | 1.39E-03 |
| isot            | 24 Cr 54 | 2.38E-10 | 8.80E-09 | 5.87E-08 | 3.29E-07 | 3.00E-06 | 9.83E-11 | 4.45E-09 | 3.11E-08 | 1.76E-07 | 1.94E-06 |
| elem            | 25 Mn    | 1.79E-04 | 1.00E-03 | 2.23E-03 | 3.65E-03 | 7.16E-03 | 1.93E-04 | 1.66E-03 | 3.89E-03 | 6.44E-03 | 1.11E-02 |
| isot            | 25 Mn 55 | 1.79E-04 | 1.00E-03 | 2.23E-03 | 3.65E-03 | 7.16E-03 | 1.93E-04 | 1.66E-03 | 3.89E-03 | 6.44E-03 | 1.11E-02 |
| elem            | 26 Fe    | 1.50E-01 | 1.48E-01 | 1.51E-01 | 1.65E-01 | 2.25E-01 | 4.28E-01 | 4.26E-01 | 4.27E-01 | 4.36E-01 | 4.68E-01 |
| isot            | 26 Fe 54 | 1.21E-04 | 2.59E-03 | 1.17E-02 | 3.03E-02 | 8.51E-02 | 9.31E-05 | 2.90E-03 | 1.35E-02 | 3.50E-02 | 9.64E-02 |
| isot            | 26 Fe 56 | 1.50E-01 | 1.45E-01 | 1.39E-01 | 1.33E-01 | 1.37E-01 | 4.27E-01 | 4.21E-01 | 4.10E-01 | 3.95E-01 | 3.61E-01 |
| isot            | 26 Fe 57 | 4.36E-04 | 6.35E-04 | 1.11E-03 | 1.70E-03 | 3.04E-03 | 1.53E-03 | 2.23E-03 | 3.64E-03 | 5.73E-03 | 1.07E-02 |
| isot            | 26 Fe 58 | 1.47E-08 | 2.68E-07 | 6.76E-07 | 1.93E-06 | 1.77E-05 | 5.52E-09 | 8.59E-08 | 2.35E-07 | 7.35E-07 | 7.05E-06 |
| elem            | 27 Co    | 4.36E-07 | 1.84E-06 | 2.37E-06 | 6.46E-06 | 5.26E-05 | 8.55E-05 | 1.11E-05 | 2.72E-05 | 5.36E-05 | 1.53E-04 |
| isot            | 27 Co 59 | 4.36E-07 | 1.84E-06 | 2.37E-06 | 6.46E-06 | 5.26E-05 | 8.55E-05 | 1.11E-05 | 2.72E-05 | 5.36E-05 | 1.53E-04 |
| elem            | 28 Ni    | 6.74E-05 | 2.80E-04 | 1.08E-03 | 2.79E-03 | 8.35E-03 | 5.28E-04 | 8.59E-04 | 3.11E-03 | 8.59E-03 | 3.41E-02 |
| isot            | 28 Ni 58 | 6.63E-05 | 2.44E-04 | 9.45E-04 | 2.44E-03 | 7.08E-03 | 2.33E-04 | 4.85E-04 | 2.66E-03 | 7.88E-03 | 3.22E-02 |
| isot            | 28 Ni 60 | 1.05E-06 | 2.99E-05 | 9.19E-05 | 1.95E-04 | 6.61E-04 | 2.92E-04 | 3.59E-04 | 3.83E-04 | 4.95E-04 | 8.56E-04 |
| isot            | 28 Ni 61 | 1.96E-08 | 8.78E-07 | 5.16E-06 | 1.39E-05 | 7.21E-05 | 2.43E-06 | 4.54E-06 | 8.43E-06 | 1.73E-05 | 5.97E-05 |
| isot            | 28 Ni 62 | 3.61E-08 | 4.51E-06 | 3.77E-05 | 1.44E-04 | 4.94E-04 | 3.44E-07 | 1.10E-05 | 5.77E-05 | 2.00E-04 | 8.95E-04 |
| isot            | 28 Ni 64 | 1.48E-10 | 3.10E-08 | 6.36E-07 | 5.89E-06 | 3.85E-05 | 5.38E-11 | 1.21E-08 | 2.33E-07 | 2.03E-06 | 1.39E-05 |
| elem            | 29 Cu    | 2.73E-08 | 1.01E-06 | 7.67E-06 | 2.24E-05 | 5.60E-05 | 2.36E-06 | 4.52E-07 | 2.89E-06 | 8.14E-06 | 2.08E-05 |
| isot            | 29 Cu 63 | 2.18E-08 | 6.00E-07 | 4.33E-06 | 9.25E-06 | 2.01E-05 | 2.35E-06 | 2.47E-07 | 1.57E-06 | 3.38E-06 | 7.15E-06 |
| isot            | 29 Cu 65 | 5.55E-09 | 4.12E-07 | 3.34E-06 | 1.32E-05 | 3.58E-05 | 8.83E-09 | 2.05E-07 | 1.31E-06 | 4.76E-06 | 1.36E-05 |
| elem            | 30 Zn    | 2.45E-07 | 8.91E-06 | 4.81E-05 | 1.06E-04 | 9.44E-05 | 4.12E-06 | 5.25E-06 | 2.18E-05 | 4.82E-05 | 4.69E-05 |
| isot            | 30 Zn 64 | 2.22E-07 | 6.53E-06 | 1.58E-05 | 1.18E-05 | 4.56E-06 | 4.06E-06 | 3.68E-06 | 6.19E-06 | 5.13E-06 | 2.90E-06 |
| isot            | 30 Zn 66 | 6.61E-09 | 1.87E-06 | 3.04E-05 | 8.11E-05 | 6.63E-05 | 1.52E-08 | 1.28E-06 | 1.47E-05 | 3.72E-05 | 3.47E-05 |
| isot            | 30 Zn 67 | 1.55E-09 | 5.19E-08 | 3.59E-07 | 1.36E-06 | 5.23E-06 | 1.71E-08 | 2.74E-08 | 1.78E-07 | 5.67E-07 | 1.88E-06 |
| isot            | 30 Zn 68 | 1.48E-08 | 4.55E-07 | 1.55E-06 | 1.21E-05 | 1.79E-05 | 2.58E-08 | 2.65E-07 | 7.41E-07 | 5.24E-06 | 7.22E-06 |
| isot            | 30 Zn 70 | 3.53E-11 | 8.54E-10 | 1.28E-08 | 1.09E-07 | 4.23E-07 | 1.33E-11 | 3.21E-10 | 5.23E-09 | 4.61E-08 | 1.62E-07 |
| elem            | 31 Ga    | 1.24E-09 | 6.86E-08 | 8.73E-07 | 4.34E-06 | 2.46E-06 | 6.33E-10 | 4.33E-08 | 4.63E-07 | 2.07E-06 | 1.07E-06 |
| isot            | 31 Ga 69 | 1.07E-09 | 6.41E-08 | 7.89E-07 | 3.46E-06 | 1.60E-06 | 5.49E-10 | 4.04E-08 | 4.06E-07 | 1.63E-06 | 7.05E-07 |
| isot            | 31 Ga 71 | 1.70E-10 | 4.52E-09 | 8.44E-08 | 8.82E-07 | 8.62E-07 | 8.42E-11 | 2.88E-09 | 5.74E-08 | 4.38E-07 | 3.63E-07 |
| elem            | 32 Ge    | 6.15E-09 | 7.34E-07 | 1.22E-05 | 2.72E-05 | 5.38E-06 | 3.95E-09 | 6.47E-07 | 7.67E-06 | 1.51E-05 | 2.65E-06 |
| isot            | 32 Ge 70 | 3.97E-09 | 6.49E-07 | 9.42E-06 | 1.55E-05 | 2.30E-06 | 2.86E-09 | 5.49E-07 | 5.54E-06 | 8.27E-06 | 1.21E-06 |
| isot            | 32 Ge 72 | 1.67E-09 | 7.74E-08 | 2.71E-06 | 1.12E-05 | 2.71E-06 | 8.46E-10 | 9.16E-08 | 2.08E-06 | 6.56E-06 | 1.30E-06 |
| isot            | 32 Ge 73 | 4.25E-10 | 7.49E-09 | 4.17E-08 | 7.52E-08 | 8.39E-08 | 2.02E-10 | 5.44E-09 | 3.71E-08 | 4.78E-08 | 3.20E-08 |
| isot            | 32 Ge 74 | 6.12E-11 | 7.32E-10 | 2.74E-08 | 4.35E-07 | 2.53E-07 | 2.18E-11 | 3.36E-10 | 1.85E-08 | 2.39E-07 | 1.03E-07 |
| isot            | 32 Ge 76 | 2.36E-11 | 1.60E-10 | 1.35E-09 | 8.73E-09 | 2.38E-08 | 1.13E-11 | 5.40E-11 | 6.48E-10 | 4.02E-09 | 8.52E-09 |
| elem            | 33 As    | 1.32E-10 | 4.21E-09 | 8.00E-08 | 4.80E-07 | 9.67E-08 | 5.29E-11 | 4.55E-09 | 6.46E-08 | 2.90E-07 | 4.41E-08 |
| isot            | 33 As 75 | 1.32E-10 | 4.21E-09 | 8.00E-08 | 4.80E-07 | 9.67E-08 | 5.29E-11 | 4.55E-09 | 6.46E-08 | 2.90E-07 | 4.41E-08 |
| elem            | 34 Se    | 3.76E-09 | 2.56E-07 | 4.57E-06 | 6.83E-06 | 4.28E-07 | 2.93E-09 | 3.70E-07 | 4.68E-06 | 5.45E-06 | 2.42E-07 |
| isot            | 34 Se 74 | 2.74E-09 | 1.97E-07 | 2.18E-06 | 2.67E-06 | 1.31E-07 | 2.16E-09 | 2.55E-07 | 2.07E-06 | 2.17E-06 | 8.28E-08 |
| isot            | 34 Se 76 | 5.83E-10 | 5.61E-08 | 2.29E-06 | 3.79E-06 | 1.98E-07 | 5.36E-10 | 1.13E-07 | 2.51E-06 | 3.04E-06 | 1.20E-07 |
| isot            | 34 Se 77 | 3.10E-10 | 1.58E-09 | 8.03E-09 | 4.37E-08 | 2.61E-08 | 1.89E-10 | 1.17E-09 | 7.94E-09 | 2.71E-08 | 1.05E-08 |
| isot            | 34 Se 78 | 4.22E-11 | 9.48E-10 | 8.11E-08 | 3.14E-07 | 4.70E-08 | 1.95E-11 | 8.01E-10 | 8.58E-08 | 2.15E-07 | 1.98E-08 |
| isot            | 34 Se 80 | 8.39E-11 | 4.16E-10 | 3.66E-09 | 1.37E-08 | 2.55E-08 | 3.06E-11 | 1.50E-10 | 1.57E-09 | 6.13E-09 | 8.24E-09 |
| elem            | 35 Br    | 6.93E-11 | 2.69E-09 | 2.67E-08 | 3.43E-08 | 8.63E-09 | 4.20E-11 | 2.97E-09 | 2.91E-08 | 2.63E-08 | 3.16E-09 |
| isot            | 35 Br 79 | 6.93E-11 | 2.69E-09 | 2.67E-08 | 3.43E-08 | 8.63E-09 | 4.20E-11 | 2.97E-09 | 2.91E-08 | 2.63E-08 | 3.16E-09 |
| elem            | 36 Kr    | 1.66E-09 | 5.35E-08 | 8.08E-07 | 5.35E-07 | 1.99E-08 | 1.55E-09 | 1.05E-07 | 1.23E-06 | 5.68E-07 | 1.20E-08 |
| isot            | 36 Kr 78 | 1.51E-09 | 2.87E-08 | 1.58E-07 | 8.53E-08 | 3.47E-09 | 1.31E-09 | 4.68E-08 | 2.32E-07 | 9.45E-08 | 2.00E-09 |
| isot            | 36 Kr 80 | 1.60E-10 | 2.48E-08 | 6.50E-07 | 4.50E-07 | 1.64E-08 | 2.38E-10 | 5.85E-08 | 9.99E-07 | 4.73E-07 | 9.97E-09 |

Table A2 continued.

| $M_{\text{WD}}$ |          | 1.06     | 1.06     | 1.06     | 1.06     | 1.06     | 1.10     | 1.10     | 1.10     | 1.10     | 1.10     |
|-----------------|----------|----------|----------|----------|----------|----------|----------|----------|----------|----------|----------|
| Z               |          | 2.25E-4  | 2.25E-3  | 9.00E-3  | 2.25E-2  | 6.75E-2  | 2.25E-4  | 2.25E-3  | 9.00E-3  | 2.25E-2  | 6.75E-2  |
| elem            | 2 He     | 5.13E-03 | 5.13E-03 | 4.90E-03 | 4.43E-03 | 2.84E-03 | 6.91E-03 | 6.87E-03 | 6.48E-03 | 5.70E-03 | 3.52E-03 |
| isot            | 2 He 3   | 2.13E-15 | 2.11E-15 | 3.26E-15 | 3.06E-15 | 4.47E-15 | 7.08E-13 | 7.45E-13 | 8.09E-13 | 9.20E-13 | 1.21E-12 |
| isot            | 2 He 4   | 5.13E-03 | 5.13E-03 | 4.90E-03 | 4.43E-03 | 2.84E-03 | 6.91E-03 | 6.87E-03 | 6.48E-03 | 5.70E-03 | 3.52E-03 |
| elem            | 6 C      | 7.21E-04 | 7.20E-04 | 6.99E-04 | 6.66E-04 | 5.76E-04 | 4.92E-04 | 4.91E-04 | 4.75E-04 | 4.51E-04 | 3.87E-04 |
| isot            | 6 C 12   | 7.21E-04 | 7.19E-04 | 6.99E-04 | 6.66E-04 | 5.76E-04 | 4.92E-04 | 4.91E-04 | 4.75E-04 | 4.51E-04 | 3.87E-04 |
| isot            | 6 C 13   | 4.56E-11 | 6.68E-10 | 2.74E-09 | 6.33E-09 | 1.38E-08 | 3.81E-11 | 4.95E-10 | 1.97E-09 | 4.57E-09 | 9.65E-09 |
| elem            | 7 N      | 5.05E-06 | 4.11E-06 | 2.82E-06 | 1.64E-06 | 5.54E-07 | 4.09E-06 | 3.35E-06 | 2.29E-06 | 1.30E-06 | 4.01E-07 |
| isot            | 7 N 14   | 5.04E-06 | 4.11E-06 | 2.82E-06 | 1.64E-06 | 5.53E-07 | 4.08E-06 | 3.35E-06 | 2.29E-06 | 1.30E-06 | 4.01E-07 |
| isot            | 7 N 15   | 1.54E-08 | 5.12E-10 | 3.01E-10 | 3.52E-10 | 5.11E-10 | 9.90E-09 | 3.74E-10 | 2.10E-10 | 2.22E-10 | 3.40E-10 |
| elem            | 8 O      | 3.42E-02 | 3.53E-02 | 3.56E-02 | 3.54E-02 | 3.19E-02 | 2.31E-02 | 2.40E-02 | 2.42E-02 | 2.39E-02 | 2.11E-02 |
| isot            | 8 O 16   | 3.42E-02 | 3.53E-02 | 3.56E-02 | 3.54E-02 | 3.19E-02 | 2.31E-02 | 2.40E-02 | 2.42E-02 | 2.39E-02 | 2.11E-02 |
| isot            | 8 O 17   | 1.81E-09 | 1.51E-08 | 2.74E-08 | 3.30E-08 | 2.68E-08 | 1.33E-09 | 1.00E-08 | 1.74E-08 | 1.98E-08 | 1.57E-08 |
| isot            | 8 O 18   | 2.76E-10 | 1.95E-10 | 1.87E-10 | 1.87E-10 | 1.79E-10 | 1.95E-10 | 1.27E-10 | 1.17E-10 | 1.10E-10 | 1.11E-10 |
| elem            | 9 F      | 3.21E-12 | 8.09E-13 | 1.61E-12 | 4.23E-12 | 1.30E-11 | 1.95E-12 | 5.40E-13 | 1.09E-12 | 2.67E-12 | 8.14E-12 |
| isot            | 9 F 19   | 3.21E-12 | 8.09E-13 | 1.61E-12 | 4.23E-12 | 1.30E-11 | 1.95E-12 | 5.40E-13 | 1.09E-12 | 2.67E-12 | 8.14E-12 |
| elem            | 10 Ne    | 2.94E-04 | 2.89E-04 | 2.81E-04 | 2.69E-04 | 2.47E-04 | 1.80E-04 | 1.77E-04 | 1.72E-04 | 1.64E-04 | 1.50E-04 |
| isot            | 10 Ne 20 | 2.93E-04 | 2.89E-04 | 2.78E-04 | 2.61E-04 | 2.14E-04 | 1.79E-04 | 1.76E-04 | 1.70E-04 | 1.58E-04 | 1.28E-04 |
| isot            | 10 Ne 21 | 5.66E-09 | 6.01E-09 | 1.90E-08 | 4.75E-08 | 1.70E-07 | 7.28E-09 | 3.94E-09 | 1.23E-08 | 3.06E-08 | 1.12E-07 |
| isot            | 10 Ne 22 | 2.11E-07 | 5.27E-07 | 2.67E-06 | 8.27E-06 | 3.29E-05 | 2.28E-07 | 3.75E-07 | 1.87E-06 | 5.69E-06 | 2.21E-05 |
| elem            | 11 Na    | 2.02E-06 | 2.21E-06 | 2.95E-06 | 4.64E-06 | 1.03E-05 | 1.24E-06 | 1.36E-06 | 1.84E-06 | 2.91E-06 | 6.59E-06 |
| isot            | 11 Na 23 | 2.02E-06 | 2.21E-06 | 2.95E-06 | 4.64E-06 | 1.03E-05 | 1.24E-06 | 1.36E-06 | 1.84E-06 | 2.91E-06 | 6.59E-06 |
| elem            | 12 Mg    | 4.92E-03 | 4.31E-03 | 3.02E-03 | 1.93E-03 | 9.31E-04 | 2.90E-03 | 2.51E-03 | 1.71E-03 | 1.07E-03 | 5.17E-04 |
| isot            | 12 Mg 24 | 4.92E-03 | 4.31E-03 | 3.01E-03 | 1.92E-03 | 8.78E-04 | 2.90E-03 | 2.51E-03 | 1.71E-03 | 1.06E-03 | 4.83E-04 |
| isot            | 12 Mg 25 | 2.12E-07 | 1.26E-06 | 3.13E-06 | 7.05E-06 | 1.86E-05 | 1.81E-07 | 7.55E-07 | 1.92E-06 | 4.33E-06 | 1.16E-05 |
| isot            | 12 Mg 26 | 1.54E-06 | 1.00E-06 | 4.40E-06 | 1.13E-05 | 3.41E-05 | 1.57E-06 | 6.56E-07 | 2.76E-06 | 7.16E-06 | 2.18E-05 |
| elem            | 13 Al    | 1.09E-05 | 4.00E-05 | 7.04E-05 | 7.67E-05 | 6.28E-05 | 6.66E-06 | 2.37E-05 | 4.02E-05 | 4.28E-05 | 3.48E-05 |
| isot            | 13 Al 27 | 1.09E-05 | 4.00E-05 | 7.04E-05 | 7.67E-05 | 6.28E-05 | 6.66E-06 | 2.37E-05 | 4.02E-05 | 4.28E-05 | 3.48E-05 |
| elem            | 14 Si    | 1.59E-01 | 1.62E-01 | 1.65E-01 | 1.63E-01 | 1.50E-01 | 1.26E-01 | 1.29E-01 | 1.31E-01 | 1.30E-01 | 1.18E-01 |
| isot            | 14 Si 28 | 1.59E-01 | 1.62E-01 | 1.64E-01 | 1.63E-01 | 1.49E-01 | 1.26E-01 | 1.29E-01 | 1.31E-01 | 1.29E-01 | 1.17E-01 |
| isot            | 14 Si 29 | 3.26E-05 | 8.45E-05 | 1.23E-04 | 1.71E-04 | 3.32E-04 | 2.36E-05 | 5.42E-05 | 7.93E-05 | 1.10E-04 | 2.12E-04 |
| isot            | 14 Si 30 | 4.93E-06 | 2.97E-05 | 1.48E-04 | 3.39E-04 | 1.03E-03 | 5.46E-06 | 1.92E-05 | 8.97E-05 | 2.00E-04 | 6.05E-04 |
| elem            | 15 P     | 1.59E-05 | 2.92E-05 | 7.02E-05 | 1.22E-04 | 2.59E-04 | 1.36E-05 | 2.10E-05 | 4.79E-05 | 8.22E-05 | 1.75E-04 |
| isot            | 15 P 31  | 1.59E-05 | 2.92E-05 | 7.02E-05 | 1.22E-04 | 2.59E-04 | 1.36E-05 | 2.10E-05 | 4.79E-05 | 8.22E-05 | 1.75E-04 |
| elem            | 16 S     | 9.95E-02 | 9.81E-02 | 9.64E-02 | 9.15E-02 | 7.21E-02 | 8.17E-02 | 8.06E-02 | 7.89E-02 | 7.45E-02 | 5.79E-02 |
| isot            | 16 S 32  | 9.95E-02 | 9.80E-02 | 9.58E-02 | 9.00E-02 | 6.78E-02 | 8.17E-02 | 8.05E-02 | 7.85E-02 | 7.35E-02 | 5.49E-02 |
| isot            | 16 S 33  | 1.64E-05 | 3.70E-05 | 7.15E-05 | 1.10E-04 | 1.92E-04 | 1.12E-05 | 2.63E-05 | 5.09E-05 | 7.88E-05 | 1.40E-04 |
| isot            | 16 S 34  | 1.32E-06 | 9.48E-05 | 4.98E-04 | 1.32E-03 | 4.11E-03 | 1.87E-06 | 6.60E-05 | 3.44E-04 | 9.06E-04 | 2.80E-03 |
| isot            | 16 S 36  | 5.47E-12 | 1.18E-09 | 1.28E-08 | 7.19E-08 | 1.28E-06 | 3.80E-12 | 7.64E-10 | 8.33E-09 | 4.75E-08 | 7.74E-07 |
| elem            | 17 Cl    | 5.97E-06 | 1.49E-05 | 3.84E-05 | 7.39E-05 | 1.40E-04 | 5.17E-06 | 1.15E-05 | 2.91E-05 | 5.51E-05 | 1.04E-04 |
| isot            | 17 Cl 35 | 3.90E-06 | 1.03E-05 | 2.94E-05 | 5.92E-05 | 1.15E-04 | 3.64E-06 | 7.90E-06 | 2.21E-05 | 4.39E-05 | 8.46E-05 |
| isot            | 17 Cl 37 | 2.07E-06 | 4.60E-06 | 9.03E-06 | 1.46E-05 | 2.52E-05 | 1.53E-06 | 3.59E-06 | 6.99E-06 | 1.13E-05 | 1.90E-05 |
| elem            | 18 Ar    | 2.32E-02 | 2.22E-02 | 2.10E-02 | 1.93E-02 | 1.50E-02 | 1.94E-02 | 1.87E-02 | 1.76E-02 | 1.60E-02 | 1.22E-02 |
| isot            | 18 Ar 36 | 2.32E-02 | 2.22E-02 | 2.07E-02 | 1.85E-02 | 1.27E-02 | 1.94E-02 | 1.86E-02 | 1.74E-02 | 1.55E-02 | 1.06E-02 |
| isot            | 18 Ar 38 | 7.13E-07 | 4.75E-05 | 2.65E-04 | 7.71E-04 | 2.34E-03 | 6.31E-07 | 3.46E-05 | 1.92E-04 | 5.55E-04 | 1.66E-03 |
| isot            | 18 Ar 40 | 2.25E-12 | 2.50E-10 | 3.02E-09 | 1.29E-08 | 1.02E-07 | 1.49E-12 | 1.63E-10 | 1.94E-09 | 8.45E-09 | 6.44E-08 |
| elem            | 19 K     | 2.34E-06 | 1.03E-05 | 2.84E-05 | 5.26E-05 | 8.78E-05 | 2.04E-06 | 8.14E-06 | 2.23E-05 | 4.05E-05 | 6.62E-05 |
| isot            | 19 K 39  | 1.94E-06 | 9.42E-06 | 2.65E-05 | 4.95E-05 | 8.34E-05 | 1.70E-06 | 7.41E-06 | 2.08E-05 | 3.81E-05 | 6.28E-05 |
| isot            | 19 K 40  | 2.57E-11 | 8.42E-10 | 5.32E-09 | 2.57E-08 | 7.07E-08 | 1.87E-11 | 6.32E-10 | 3.96E-09 | 1.86E-08 | 4.97E-08 |
| isot            | 19 K 41  | 4.04E-07 | 9.02E-07 | 1.90E-06 | 3.06E-06 | 4.30E-06 | 3.37E-07 | 7.34E-07 | 1.52E-06 | 2.42E-06 | 3.33E-06 |
| elem            | 20 Ca    | 2.49E-02 | 2.34E-02 | 2.13E-02 | 1.86E-02 | 1.28E-02 | 2.10E-02 | 1.98E-02 | 1.81E-02 | 1.58E-02 | 1.08E-02 |
| isot            | 20 Ca 40 | 2.49E-02 | 2.34E-02 | 2.13E-02 | 1.85E-02 | 1.27E-02 | 2.10E-02 | 1.98E-02 | 1.81E-02 | 1.57E-02 | 1.07E-02 |
| isot            | 20 Ca 42 | 8.92E-09 | 9.83E-07 | 6.25E-06 | 1.94E-05 | 5.53E-05 | 6.85E-09 | 7.42E-07 | 4.68E-06 | 1.44E-05 | 3.97E-05 |
| isot            | 20 Ca 43 | 2.16E-08 | 2.46E-08 | 1.11E-07 | 9.76E-08 | 1.70E-07 | 2.99E-08 | 3.54E-08 | 1.42E-07 | 1.07E-07 | 1.27E-07 |
| isot            | 20 Ca 44 | 2.68E-05 | 2.44E-05 | 2.49E-05 | 2.04E-05 | 1.19E-05 | 2.68E-05 | 2.49E-05 | 2.58E-05 | 2.08E-05 | 1.12E-05 |
| isot            | 20 Ca 46 | 3.89E-13 | 1.20E-10 | 1.40E-09 | 6.06E-09 | 4.54E-08 | 2.41E-13 | 7.85E-11 | 9.27E-10 | 3.97E-09 | 2.69E-08 |
| isot            | 20 Ca 48 | 1.88E-12 | 2.03E-11 | 2.96E-10 | 1.72E-09 | 1.36E-08 | 1.19E-12 | 1.30E-11 | 2.01E-10 | 1.19E-09 | 8.81E-09 |
| elem            | 21 Sc    | 6.27E-08 | 7.92E-08 | 1.25E-07 | 1.84E-07 | 3.17E-07 | 6.12E-08 | 6.85E-08 | 1.06E-07 | 1.54E-07 | 2.51E-07 |
| isot            | 21 Sc 45 | 6.27E-08 | 7.92E-08 | 1.25E-07 | 1.84E-07 | 3.17E-07 | 6.12E-08 | 6.85E-08 | 1.06E-07 | 1.54E-07 | 2.51E-07 |

Table A2 continued.

| $M_{\text{WD}}$ |          | 1.06     | 1.06     | 1.06     | 1.06     | 1.06     | 1.10     | 1.10     | 1.10     | 1.10     | 1.10     |
|-----------------|----------|----------|----------|----------|----------|----------|----------|----------|----------|----------|----------|
| Z               |          | 2.25E-4  | 2.25E-3  | 9.00E-3  | 2.25E-2  | 6.75E-2  | 2.25E-4  | 2.25E-3  | 9.00E-3  | 2.25E-2  | 6.75E-2  |
| elem            | 22 Ti    | 3.48E-04 | 3.42E-04 | 3.25E-04 | 2.95E-04 | 2.27E-04 | 3.07E-04 | 3.04E-04 | 2.89E-04 | 2.60E-04 | 1.95E-04 |
| isot            | 22 Ti 46 | 1.47E-06 | 9.74E-07 | 5.09E-06 | 1.33E-05 | 3.15E-05 | 1.89E-06 | 7.65E-07 | 3.92E-06 | 1.01E-05 | 2.35E-05 |
| isot            | 22 Ti 47 | 1.74E-06 | 1.10E-07 | 3.12E-07 | 5.35E-07 | 1.13E-06 | 1.97E-06 | 1.53E-07 | 3.77E-07 | 5.43E-07 | 8.77E-07 |
| isot            | 22 Ti 48 | 3.41E-04 | 3.33E-04 | 3.07E-04 | 2.65E-04 | 1.74E-04 | 3.01E-04 | 2.96E-04 | 2.74E-04 | 2.35E-04 | 1.53E-04 |
| isot            | 22 Ti 49 | 3.71E-06 | 7.73E-06 | 1.22E-05 | 1.68E-05 | 1.99E-05 | 2.81E-06 | 6.91E-06 | 1.08E-05 | 1.49E-05 | 1.76E-05 |
| isot            | 22 Ti 50 | 6.13E-12 | 1.62E-10 | 1.61E-09 | 1.52E-08 | 3.91E-07 | 3.93E-12 | 1.06E-10 | 1.11E-09 | 9.54E-09 | 2.07E-07 |
| elem            | 23 V     | 3.14E-06 | 1.14E-05 | 3.12E-05 | 5.37E-05 | 9.36E-05 | 3.43E-06 | 9.95E-06 | 2.74E-05 | 4.72E-05 | 8.16E-05 |
| isot            | 23 V 50  | 2.96E-12 | 6.69E-11 | 1.23E-09 | 8.70E-09 | 4.73E-08 | 2.00E-12 | 4.85E-11 | 7.93E-10 | 5.17E-09 | 2.90E-08 |
| isot            | 23 V 51  | 3.14E-06 | 1.14E-05 | 3.12E-05 | 5.37E-05 | 9.35E-05 | 3.43E-06 | 9.95E-06 | 2.74E-05 | 4.72E-05 | 8.15E-05 |
| elem            | 24 Cr    | 8.89E-03 | 8.78E-03 | 8.41E-03 | 7.86E-03 | 7.14E-03 | 7.71E-03 | 7.64E-03 | 7.32E-03 | 6.85E-03 | 6.28E-03 |
| isot            | 24 Cr 50 | 7.85E-06 | 1.53E-05 | 7.85E-05 | 2.29E-04 | 7.70E-04 | 8.99E-06 | 1.25E-05 | 6.55E-05 | 1.91E-04 | 6.41E-04 |
| isot            | 24 Cr 52 | 8.67E-03 | 8.43E-03 | 7.80E-03 | 6.87E-03 | 5.26E-03 | 7.54E-03 | 7.33E-03 | 6.78E-03 | 5.99E-03 | 4.63E-03 |
| isot            | 24 Cr 53 | 2.07E-04 | 3.36E-04 | 5.38E-04 | 7.64E-04 | 1.11E-03 | 1.60E-04 | 2.98E-04 | 4.72E-04 | 6.72E-04 | 1.00E-03 |
| isot            | 24 Cr 54 | 4.26E-11 | 2.14E-09 | 1.62E-08 | 9.25E-08 | 1.19E-06 | 2.74E-11 | 1.47E-09 | 1.18E-08 | 6.77E-08 | 9.04E-07 |
| elem            | 25 Mn    | 1.01E-04 | 1.32E-03 | 3.21E-03 | 5.34E-03 | 9.00E-03 | 9.49E-05 | 1.14E-03 | 2.80E-03 | 4.86E-03 | 9.20E-03 |
| isot            | 25 Mn 55 | 1.01E-04 | 1.32E-03 | 3.21E-03 | 5.34E-03 | 9.00E-03 | 9.49E-05 | 1.14E-03 | 2.80E-03 | 4.86E-03 | 9.20E-03 |
| elem            | 26 Fe    | 6.90E-01 | 6.89E-01 | 6.84E-01 | 6.79E-01 | 6.62E-01 | 7.98E-01 | 7.97E-01 | 7.90E-01 | 7.79E-01 | 7.46E-01 |
| isot            | 26 Fe 54 | 5.84E-05 | 2.09E-03 | 1.01E-02 | 2.65E-02 | 7.26E-02 | 4.84E-05 | 1.71E-03 | 8.47E-03 | 2.25E-02 | 6.69E-02 |
| isot            | 26 Fe 56 | 6.85E-01 | 6.79E-01 | 6.64E-01 | 6.38E-01 | 5.67E-01 | 7.91E-01 | 7.85E-01 | 7.69E-01 | 7.39E-01 | 6.51E-01 |
| isot            | 26 Fe 57 | 4.94E-03 | 7.62E-03 | 1.01E-02 | 1.41E-02 | 2.32E-02 | 6.86E-03 | 1.00E-02 | 1.30E-02 | 1.78E-02 | 2.79E-02 |
| isot            | 26 Fe 58 | 2.25E-09 | 3.01E-08 | 8.69E-08 | 2.78E-07 | 2.42E-06 | 1.45E-09 | 1.86E-08 | 5.49E-08 | 1.75E-07 | 1.42E-06 |
| elem            | 27 Co    | 7.34E-04 | 8.85E-05 | 2.96E-04 | 4.74E-04 | 6.66E-04 | 9.07E-04 | 1.30E-04 | 4.03E-04 | 6.14E-04 | 8.14E-04 |
| isot            | 27 Co 59 | 7.34E-04 | 8.85E-05 | 2.96E-04 | 4.74E-04 | 6.66E-04 | 9.07E-04 | 1.30E-04 | 4.03E-04 | 6.14E-04 | 8.14E-04 |
| elem            | 28 Ni    | 8.12E-03 | 8.24E-03 | 1.53E-02 | 3.14E-02 | 9.36E-02 | 1.09E-02 | 1.13E-02 | 2.04E-02 | 4.08E-02 | 1.13E-01 |
| isot            | 28 Ni 58 | 1.27E-03 | 7.42E-04 | 8.01E-03 | 2.39E-02 | 8.65E-02 | 1.63E-03 | 1.34E-03 | 1.09E-02 | 3.13E-02 | 1.04E-01 |
| isot            | 28 Ni 60 | 6.75E-03 | 7.14E-03 | 6.28E-03 | 5.37E-03 | 3.00E-03 | 9.14E-03 | 9.49E-03 | 8.21E-03 | 6.81E-03 | 3.55E-03 |
| isot            | 28 Ni 61 | 7.85E-05 | 1.45E-04 | 1.82E-04 | 2.20E-04 | 2.22E-04 | 1.13E-04 | 1.96E-04 | 2.42E-04 | 2.82E-04 | 2.69E-04 |
| isot            | 28 Ni 62 | 1.13E-05 | 2.08E-04 | 8.25E-04 | 1.93E-03 | 3.94E-03 | 3.09E-05 | 2.88E-04 | 1.09E-03 | 2.44E-03 | 4.69E-03 |
| isot            | 28 Ni 64 | 2.28E-11 | 5.00E-09 | 8.43E-08 | 6.25E-07 | 4.27E-06 | 1.54E-11 | 3.39E-09 | 5.33E-08 | 3.60E-07 | 2.28E-06 |
| elem            | 29 Cu    | 6.51E-05 | 5.22E-06 | 2.09E-06 | 4.23E-06 | 9.19E-06 | 7.97E-05 | 9.45E-06 | 2.06E-06 | 3.59E-06 | 6.84E-06 |
| isot            | 29 Cu 63 | 6.48E-05 | 4.68E-06 | 1.05E-06 | 2.09E-06 | 4.24E-06 | 7.93E-05 | 8.78E-06 | 1.02E-06 | 1.90E-06 | 3.77E-06 |
| isot            | 29 Cu 65 | 2.89E-07 | 5.44E-07 | 1.04E-06 | 2.15E-06 | 4.95E-06 | 3.71E-07 | 6.67E-07 | 1.04E-06 | 1.69E-06 | 3.07E-06 |
| elem            | 30 Zn    | 1.65E-04 | 7.88E-05 | 4.49E-05 | 6.13E-05 | 5.87E-05 | 2.15E-04 | 1.07E-04 | 5.30E-05 | 6.59E-05 | 6.12E-05 |
| isot            | 30 Zn 64 | 1.61E-04 | 7.32E-05 | 2.55E-05 | 1.75E-05 | 6.40E-06 | 2.10E-04 | 1.00E-04 | 3.19E-05 | 2.13E-05 | 7.31E-06 |
| isot            | 30 Zn 66 | 1.05E-06 | 5.29E-06 | 1.90E-05 | 4.16E-05 | 4.86E-05 | 1.70E-06 | 6.77E-06 | 2.08E-05 | 4.33E-05 | 5.17E-05 |
| isot            | 30 Zn 67 | 7.25E-07 | 2.01E-08 | 8.46E-08 | 2.37E-07 | 6.40E-07 | 8.37E-07 | 2.78E-08 | 5.98E-08 | 1.60E-07 | 3.85E-07 |
| isot            | 30 Zn 68 | 2.02E-06 | 2.12E-07 | 3.01E-07 | 1.96E-06 | 2.97E-06 | 2.46E-06 | 2.17E-07 | 1.92E-07 | 1.12E-06 | 1.80E-06 |
| isot            | 30 Zn 70 | 5.24E-12 | 1.37E-10 | 2.22E-09 | 1.80E-08 | 5.64E-08 | 3.59E-12 | 9.68E-11 | 1.51E-09 | 1.14E-08 | 3.34E-08 |
| elem            | 31 Ga    | 1.96E-09 | 2.43E-08 | 2.03E-07 | 8.85E-07 | 4.74E-07 | 2.45E-09 | 1.80E-08 | 1.32E-07 | 5.65E-07 | 3.15E-07 |
| isot            | 31 Ga 69 | 1.09E-09 | 2.23E-08 | 1.69E-07 | 6.90E-07 | 3.24E-07 | 1.33E-09 | 1.62E-08 | 1.06E-07 | 4.37E-07 | 2.18E-07 |
| isot            | 31 Ga 71 | 8.67E-10 | 2.02E-09 | 3.37E-08 | 1.95E-07 | 1.50E-07 | 1.12E-09 | 1.74E-09 | 2.52E-08 | 1.29E-07 | 9.62E-08 |
| elem            | 32 Ge    | 6.74E-08 | 5.02E-07 | 4.03E-06 | 8.15E-06 | 1.62E-06 | 8.89E-08 | 4.14E-07 | 2.71E-06 | 5.65E-06 | 1.25E-06 |
| isot            | 32 Ge 70 | 4.93E-08 | 4.29E-07 | 2.81E-06 | 4.40E-06 | 8.76E-07 | 6.72E-08 | 3.57E-07 | 1.88E-06 | 3.07E-06 | 7.32E-07 |
| isot            | 32 Ge 72 | 1.80E-08 | 6.97E-08 | 1.18E-06 | 3.59E-06 | 6.85E-07 | 2.17E-08 | 5.42E-08 | 7.91E-07 | 2.46E-06 | 4.75E-07 |
| isot            | 32 Ge 73 | 9.90E-11 | 3.64E-09 | 2.91E-08 | 3.29E-08 | 1.23E-08 | 8.66E-11 | 2.86E-09 | 2.41E-08 | 2.72E-08 | 7.83E-09 |
| isot            | 32 Ge 74 | 8.08E-12 | 1.87E-10 | 1.10E-08 | 1.33E-07 | 4.86E-08 | 4.93E-12 | 1.42E-10 | 8.04E-09 | 8.86E-08 | 3.16E-08 |
| isot            | 32 Ge 76 | 4.66E-12 | 2.26E-11 | 4.17E-10 | 2.34E-09 | 2.95E-09 | 2.79E-12 | 1.40E-11 | 3.57E-10 | 1.86E-09 | 1.77E-09 |
| elem            | 33 As    | 2.39E-11 | 3.96E-09 | 4.54E-08 | 1.83E-07 | 2.47E-08 | 1.77E-11 | 3.37E-09 | 3.51E-08 | 1.30E-07 | 1.72E-08 |
| isot            | 33 As 75 | 2.39E-11 | 3.96E-09 | 4.54E-08 | 1.83E-07 | 2.47E-08 | 1.77E-11 | 3.37E-09 | 3.51E-08 | 1.30E-07 | 1.72E-08 |
| elem            | 34 Se    | 2.19E-09 | 3.47E-07 | 3.43E-06 | 3.90E-06 | 1.46E-07 | 2.16E-09 | 2.88E-07 | 2.61E-06 | 3.14E-06 | 1.14E-07 |
| isot            | 34 Se 74 | 1.63E-09 | 2.16E-07 | 1.39E-06 | 1.51E-06 | 5.48E-08 | 1.62E-09 | 1.72E-07 | 1.02E-06 | 1.20E-06 | 4.41E-08 |
| isot            | 34 Se 76 | 4.47E-10 | 1.28E-07 | 1.95E-06 | 2.19E-06 | 7.52E-08 | 4.56E-10 | 1.14E-07 | 1.51E-06 | 1.78E-06 | 5.91E-08 |
| isot            | 34 Se 77 | 9.65E-11 | 1.17E-09 | 8.45E-09 | 1.86E-08 | 4.50E-09 | 7.79E-11 | 1.15E-09 | 8.22E-09 | 1.50E-08 | 2.95E-09 |
| isot            | 34 Se 78 | 7.61E-12 | 8.46E-10 | 7.97E-08 | 1.77E-07 | 9.25E-09 | 4.81E-12 | 7.90E-10 | 6.18E-08 | 1.42E-07 | 6.17E-09 |
| isot            | 34 Se 80 | 1.11E-11 | 5.68E-11 | 1.08E-09 | 3.96E-09 | 2.55E-09 | 6.75E-12 | 3.59E-11 | 9.82E-10 | 3.27E-09 | 1.49E-09 |
| elem            | 35 Br    | 2.19E-11 | 3.60E-09 | 3.38E-08 | 2.80E-08 | 1.28E-09 | 2.03E-11 | 3.50E-09 | 3.11E-08 | 2.62E-08 | 8.39E-10 |
| isot            | 35 Br 79 | 2.19E-11 | 3.60E-09 | 3.38E-08 | 2.80E-08 | 1.28E-09 | 2.03E-11 | 3.50E-09 | 3.11E-08 | 2.62E-08 | 8.39E-10 |
| elem            | 36 Kr    | 1.19E-09 | 1.56E-07 | 1.30E-06 | 5.53E-07 | 5.98E-09 | 1.19E-09 | 1.58E-07 | 1.17E-06 | 5.26E-07 | 4.42E-09 |
| isot            | 36 Kr 78 | 9.49E-10 | 6.07E-08 | 2.53E-07 | 1.02E-07 | 1.04E-09 | 9.43E-10 | 5.82E-08 | 2.30E-07 | 1.02E-07 | 8.11E-10 |
| isot            | 36 Kr 80 | 2.41E-10 | 9.54E-08 | 1.04E-06 | 4.50E-07 | 4.94E-09 | 2.46E-10 | 9.95E-08 | 9.39E-07 | 4.24E-07 | 3.61E-09 |

Table A2 *continued*.

| $M_{\text{WD}}$ |          | 1.15     | 1.15     | 1.15     | 1.15     | 1.15     |
|-----------------|----------|----------|----------|----------|----------|----------|
| Z               |          | 2.25E-4  | 2.25E-3  | 9.00E-3  | 2.25E-2  | 6.75E-2  |
| elem            | 2 He     | 7.90E-03 | 7.81E-03 | 7.27E-03 | 6.34E-03 | 4.06E-03 |
| isot            | 2 He 3   | 4.26E-12 | 4.26E-12 | 4.22E-12 | 4.20E-12 | 4.03E-12 |
| isot            | 2 He 4   | 7.90E-03 | 7.81E-03 | 7.27E-03 | 6.34E-03 | 4.06E-03 |
| elem            | 6 C      | 3.00E-04 | 2.99E-04 | 2.88E-04 | 2.72E-04 | 2.30E-04 |
| isot            | 6 C 12   | 3.00E-04 | 2.99E-04 | 2.88E-04 | 2.72E-04 | 2.30E-04 |
| isot            | 6 C 13   | 2.85E-11 | 3.07E-10 | 1.39E-09 | 3.25E-09 | 6.27E-09 |
| elem            | 7 N      | 2.90E-06 | 2.41E-06 | 1.66E-06 | 9.51E-07 | 2.66E-07 |
| isot            | 7 N 14   | 2.90E-06 | 2.41E-06 | 1.66E-06 | 9.51E-07 | 2.65E-07 |
| isot            | 7 N 15   | 5.50E-09 | 2.57E-10 | 1.35E-10 | 1.38E-10 | 1.95E-10 |
| elem            | 8 O      | 1.32E-02 | 1.38E-02 | 1.39E-02 | 1.37E-02 | 1.18E-02 |
| isot            | 8 O 16   | 1.32E-02 | 1.38E-02 | 1.39E-02 | 1.37E-02 | 1.18E-02 |
| isot            | 8 O 17   | 9.44E-10 | 6.21E-09 | 9.63E-09 | 1.07E-08 | 7.71E-09 |
| isot            | 8 O 18   | 1.34E-10 | 8.11E-11 | 6.54E-11 | 5.73E-11 | 5.76E-11 |
| elem            | 9 F      | 9.73E-13 | 3.24E-13 | 6.30E-13 | 1.54E-12 | 4.36E-12 |
| isot            | 9 F 19   | 9.73E-13 | 3.24E-13 | 6.30E-13 | 1.54E-12 | 4.36E-12 |
| elem            | 10 Ne    | 9.42E-05 | 9.28E-05 | 8.99E-05 | 8.54E-05 | 7.84E-05 |
| isot            | 10 Ne 20 | 9.40E-05 | 9.25E-05 | 8.86E-05 | 8.18E-05 | 6.50E-05 |
| isot            | 10 Ne 21 | 5.17E-09 | 2.54E-09 | 6.73E-09 | 1.77E-08 | 6.31E-08 |
| isot            | 10 Ne 22 | 1.83E-07 | 2.51E-07 | 1.19E-06 | 3.58E-06 | 1.34E-05 |
| elem            | 11 Na    | 6.46E-07 | 7.17E-07 | 9.87E-07 | 1.59E-06 | 3.60E-06 |
| isot            | 11 Na 23 | 6.46E-07 | 7.17E-07 | 9.87E-07 | 1.59E-06 | 3.60E-06 |
| elem            | 12 Mg    | 1.34E-03 | 1.15E-03 | 7.62E-04 | 4.70E-04 | 2.30E-04 |
| isot            | 12 Mg 24 | 1.34E-03 | 1.14E-03 | 7.60E-04 | 4.63E-04 | 2.12E-04 |
| isot            | 12 Mg 25 | 1.31E-07 | 3.85E-07 | 1.02E-06 | 2.29E-06 | 6.25E-06 |
| isot            | 12 Mg 26 | 1.23E-06 | 4.64E-07 | 1.49E-06 | 3.89E-06 | 1.21E-05 |
| elem            | 13 Al    | 3.47E-06 | 1.15E-05 | 1.86E-05 | 1.93E-05 | 1.57E-05 |
| isot            | 13 Al 27 | 3.47E-06 | 1.15E-05 | 1.86E-05 | 1.93E-05 | 1.57E-05 |
| elem            | 14 Si    | 8.82E-02 | 8.98E-02 | 9.09E-02 | 8.94E-02 | 7.82E-02 |
| isot            | 14 Si 28 | 8.82E-02 | 8.97E-02 | 9.08E-02 | 8.93E-02 | 7.78E-02 |
| isot            | 14 Si 29 | 1.69E-05 | 2.85E-05 | 4.22E-05 | 5.81E-05 | 1.12E-04 |
| isot            | 14 Si 30 | 6.29E-06 | 1.09E-05 | 4.36E-05 | 9.50E-05 | 2.88E-04 |
| elem            | 15 P     | 1.07E-05 | 1.33E-05 | 2.76E-05 | 4.64E-05 | 9.79E-05 |
| isot            | 15 P 31  | 1.07E-05 | 1.33E-05 | 2.76E-05 | 4.64E-05 | 9.79E-05 |
| elem            | 16 S     | 5.95E-02 | 5.88E-02 | 5.74E-02 | 5.38E-02 | 4.08E-02 |
| isot            | 16 S 32  | 5.95E-02 | 5.87E-02 | 5.71E-02 | 5.32E-02 | 3.92E-02 |
| isot            | 16 S 33  | 6.57E-06 | 1.60E-05 | 3.09E-05 | 4.79E-05 | 8.47E-05 |
| isot            | 16 S 34  | 2.80E-06 | 3.86E-05 | 1.97E-04 | 5.15E-04 | 1.57E-03 |
| isot            | 16 S 36  | 2.31E-12 | 4.31E-10 | 4.71E-09 | 2.73E-08 | 4.02E-07 |
| elem            | 17 Cl    | 4.17E-06 | 7.68E-06 | 1.89E-05 | 3.53E-05 | 6.50E-05 |
| isot            | 17 Cl 35 | 3.21E-06 | 5.27E-06 | 1.42E-05 | 2.79E-05 | 5.27E-05 |
| isot            | 17 Cl 37 | 9.58E-07 | 2.41E-06 | 4.62E-06 | 7.41E-06 | 1.22E-05 |
| elem            | 18 Ar    | 1.46E-02 | 1.41E-02 | 1.33E-02 | 1.20E-02 | 9.01E-03 |
| isot            | 18 Ar 36 | 1.46E-02 | 1.41E-02 | 1.31E-02 | 1.17E-02 | 8.02E-03 |
| isot            | 18 Ar 38 | 5.53E-07 | 2.10E-05 | 1.17E-04 | 3.37E-04 | 9.83E-04 |
| isot            | 18 Ar 40 | 8.80E-13 | 9.47E-11 | 1.08E-09 | 4.77E-09 | 3.51E-08 |
| elem            | 19 K     | 1.66E-06 | 5.40E-06 | 1.50E-05 | 2.68E-05 | 4.25E-05 |
| isot            | 19 K 39  | 1.41E-06 | 4.88E-06 | 1.40E-05 | 2.52E-05 | 4.02E-05 |
| isot            | 19 K 40  | 1.11E-11 | 4.13E-10 | 2.64E-09 | 1.21E-08 | 3.11E-08 |
| isot            | 19 K 41  | 2.51E-07 | 5.14E-07 | 1.05E-06 | 1.66E-06 | 2.23E-06 |
| elem            | 20 Ca    | 1.61E-02 | 1.53E-02 | 1.40E-02 | 1.22E-02 | 8.39E-03 |
| isot            | 20 Ca 40 | 1.61E-02 | 1.53E-02 | 1.40E-02 | 1.22E-02 | 8.35E-03 |
| isot            | 20 Ca 42 | 5.03E-09 | 4.66E-07 | 2.97E-06 | 9.08E-06 | 2.45E-05 |
| isot            | 20 Ca 43 | 3.73E-08 | 4.80E-08 | 1.79E-07 | 1.22E-07 | 8.76E-08 |
| isot            | 20 Ca 44 | 2.51E-05 | 2.42E-05 | 2.55E-05 | 2.03E-05 | 1.04E-05 |
| isot            | 20 Ca 46 | 1.58E-13 | 4.42E-11 | 5.30E-10 | 2.27E-09 | 1.37E-08 |
| isot            | 20 Ca 48 | 6.20E-13 | 7.58E-12 | 1.19E-10 | 7.11E-10 | 4.97E-09 |
| elem            | 21 Sc    | 6.22E-08 | 5.51E-08 | 8.28E-08 | 1.18E-07 | 1.82E-07 |
| isot            | 21 Sc 45 | 6.22E-08 | 5.51E-08 | 8.28E-08 | 1.18E-07 | 1.82E-07 |

Table A2 *continued*.

| $M_{\text{WD}}$ |          | 1.15     | 1.15     | 1.15     | 1.15     | 1.15     |
|-----------------|----------|----------|----------|----------|----------|----------|
| Z               |          | 2.25E-4  | 2.25E-3  | 9.00E-3  | 2.25E-2  | 6.75E-2  |
| elem            | 22 Ti    | 2.53E-04 | 2.52E-04 | 2.39E-04 | 2.14E-04 | 1.58E-04 |
| isot            | 22 Ti 46 | 2.36E-06 | 5.23E-07 | 2.53E-06 | 6.48E-06 | 1.49E-05 |
| isot            | 22 Ti 47 | 2.08E-06 | 2.01E-07 | 4.36E-07 | 5.49E-07 | 6.42E-07 |
| isot            | 22 Ti 48 | 2.46E-04 | 2.45E-04 | 2.27E-04 | 1.95E-04 | 1.28E-04 |
| isot            | 22 Ti 49 | 2.06E-06 | 5.79E-06 | 8.85E-06 | 1.22E-05 | 1.49E-05 |
| isot            | 22 Ti 50 | 2.17E-12 | 6.20E-11 | 6.94E-10 | 5.24E-09 | 9.06E-08 |
| elem            | 23 V     | 3.30E-06 | 8.00E-06 | 2.24E-05 | 3.90E-05 | 6.91E-05 |
| isot            | 23 V 50  | 1.10E-12 | 3.08E-11 | 4.45E-10 | 2.65E-09 | 1.55E-08 |
| isot            | 23 V 51  | 3.30E-06 | 8.00E-06 | 2.24E-05 | 3.90E-05 | 6.91E-05 |
| elem            | 24 Cr    | 6.18E-03 | 6.16E-03 | 5.94E-03 | 5.75E-03 | 5.64E-03 |
| isot            | 24 Cr 50 | 9.90E-06 | 9.05E-06 | 4.82E-05 | 1.41E-04 | 4.70E-04 |
| isot            | 24 Cr 52 | 6.07E-03 | 5.90E-03 | 5.50E-03 | 5.02E-03 | 4.20E-03 |
| isot            | 24 Cr 53 | 1.05E-04 | 2.48E-04 | 3.90E-04 | 5.88E-04 | 9.69E-04 |
| isot            | 24 Cr 54 | 1.53E-11 | 8.43E-10 | 7.37E-09 | 4.28E-08 | 5.64E-07 |
| elem            | 25 Mn    | 9.45E-05 | 8.96E-04 | 2.43E-03 | 5.37E-03 | 1.15E-02 |
| isot            | 25 Mn 55 | 9.45E-05 | 8.96E-04 | 2.43E-03 | 5.37E-03 | 1.15E-02 |
| elem            | 26 Fe    | 9.28E-01 | 9.27E-01 | 9.17E-01 | 9.01E-01 | 8.54E-01 |
| isot            | 26 Fe 54 | 3.28E-05 | 1.23E-03 | 6.54E-03 | 1.99E-02 | 6.94E-02 |
| isot            | 26 Fe 56 | 9.19E-01 | 9.13E-01 | 8.94E-01 | 8.59E-01 | 7.52E-01 |
| isot            | 26 Fe 57 | 9.20E-03 | 1.27E-02 | 1.64E-02 | 2.17E-02 | 3.24E-02 |
| isot            | 26 Fe 58 | 8.02E-10 | 1.00E-08 | 3.06E-08 | 9.66E-08 | 7.08E-07 |
| elem            | 27 Co    | 1.06E-03 | 1.66E-04 | 4.49E-04 | 6.51E-04 | 8.87E-04 |
| isot            | 27 Co 59 | 1.06E-03 | 1.66E-04 | 4.49E-04 | 6.51E-04 | 8.87E-04 |
| elem            | 28 Ni    | 1.30E-02 | 1.40E-02 | 2.56E-02 | 4.87E-02 | 1.25E-01 |
| isot            | 28 Ni 58 | 2.75E-03 | 3.17E-03 | 1.53E-02 | 3.85E-02 | 1.16E-01 |
| isot            | 28 Ni 60 | 1.00E-02 | 1.03E-02 | 8.83E-03 | 7.24E-03 | 3.88E-03 |
| isot            | 28 Ni 61 | 1.25E-04 | 2.19E-04 | 2.70E-04 | 3.11E-04 | 3.00E-04 |
| isot            | 28 Ni 62 | 4.03E-05 | 3.06E-04 | 1.17E-03 | 2.57E-03 | 5.11E-03 |
| isot            | 28 Ni 64 | 8.58E-12 | 2.05E-09 | 2.96E-08 | 1.77E-07 | 1.00E-06 |
| elem            | 29 Cu    | 9.08E-05 | 1.47E-05 | 1.98E-06 | 3.07E-06 | 5.23E-06 |
| isot            | 29 Cu 63 | 9.04E-05 | 1.39E-05 | 9.65E-07 | 1.70E-06 | 3.42E-06 |
| isot            | 29 Cu 65 | 3.77E-07 | 7.49E-07 | 1.02E-06 | 1.37E-06 | 1.81E-06 |
| elem            | 30 Zn    | 2.42E-04 | 1.36E-04 | 5.65E-05 | 6.68E-05 | 6.49E-05 |
| isot            | 30 Zn 64 | 2.37E-04 | 1.29E-04 | 3.54E-05 | 2.35E-05 | 8.36E-06 |
| isot            | 30 Zn 66 | 1.90E-06 | 7.36E-06 | 2.09E-05 | 4.27E-05 | 5.54E-05 |
| isot            | 30 Zn 67 | 8.96E-07 | 5.24E-08 | 3.83E-08 | 9.79E-08 | 2.08E-07 |
| isot            | 30 Zn 68 | 2.81E-06 | 2.60E-07 | 1.10E-07 | 5.40E-07 | 9.31E-07 |
| isot            | 30 Zn 70 | 2.18E-12 | 5.94E-11 | 9.09E-10 | 6.34E-09 | 1.64E-08 |
| elem            | 31 Ga    | 2.89E-09 | 1.20E-08 | 7.32E-08 | 3.02E-07 | 1.79E-07 |
| isot            | 31 Ga 69 | 1.53E-09 | 1.06E-08 | 5.68E-08 | 2.30E-07 | 1.28E-07 |
| isot            | 31 Ga 71 | 1.36E-09 | 1.43E-09 | 1.64E-08 | 7.26E-08 | 5.16E-08 |
| elem            | 32 Ge    | 1.02E-07 | 3.11E-07 | 1.55E-06 | 3.33E-06 | 9.00E-07 |
| isot            | 32 Ge 70 | 7.71E-08 | 2.75E-07 | 1.11E-06 | 1.89E-06 | 6.05E-07 |
| isot            | 32 Ge 72 | 2.49E-08 | 3.39E-08 | 4.21E-07 | 1.37E-06 | 2.72E-07 |
| isot            | 32 Ge 73 | 6.53E-11 | 1.93E-09 | 1.74E-08 | 2.03E-08 | 4.30E-09 |
| isot            | 32 Ge 74 | 2.62E-12 | 9.81E-11 | 5.22E-09 | 5.01E-08 | 1.77E-08 |
| isot            | 32 Ge 76 | 1.47E-12 | 7.89E-12 | 2.86E-10 | 1.35E-09 | 9.14E-10 |
| elem            | 33 As    | 1.18E-11 | 2.50E-09 | 2.32E-08 | 7.92E-08 | 1.05E-08 |
| isot            | 33 As 75 | 1.18E-11 | 2.50E-09 | 2.32E-08 | 7.92E-08 | 1.05E-08 |
| elem            | 34 Se    | 2.17E-09 | 1.93E-07 | 1.57E-06 | 2.05E-06 | 7.49E-08 |
| isot            | 34 Se 74 | 1.61E-09 | 1.10E-07 | 5.89E-07 | 7.71E-07 | 2.99E-08 |
| isot            | 34 Se 76 | 4.92E-10 | 8.10E-08 | 9.31E-07 | 1.17E-06 | 3.90E-08 |
| isot            | 34 Se 77 | 6.96E-11 | 9.95E-10 | 7.49E-09 | 1.11E-08 | 1.70E-09 |
| isot            | 34 Se 78 | 2.60E-12 | 6.00E-10 | 3.85E-08 | 9.41E-08 | 3.60E-09 |
| isot            | 34 Se 80 | 3.52E-12 | 2.08E-11 | 8.61E-10 | 2.55E-09 | 7.31E-10 |
| elem            | 35 Br    | 1.72E-11 | 2.95E-09 | 2.47E-08 | 2.21E-08 | 5.05E-10 |
| isot            | 35 Br 79 | 1.72E-11 | 2.95E-09 | 2.47E-08 | 2.21E-08 | 5.05E-10 |
| elem            | 36 Kr    | 1.28E-09 | 1.30E-07 | 8.51E-07 | 4.23E-07 | 2.84E-09 |
| isot            | 36 Kr 78 | 9.78E-10 | 4.51E-08 | 1.70E-07 | 8.64E-08 | 5.48E-10 |
| isot            | 36 Kr 80 | 3.00E-10 | 8.45E-08 | 6.81E-07 | 3.37E-07 | 2.29E-09 |

Table A3. Radioactivities with half-life longer than one day in Chandrasekhar-mass DDT models with the standard  $^{12}\text{C}+^{16}\text{O}$  reaction rate.

|                     |          |          |          |          |          |          |          |          |          |          |
|---------------------|----------|----------|----------|----------|----------|----------|----------|----------|----------|----------|
| $\rho_{\text{DDT}}$ | 1.2E+07  | 1.2E+07  | 1.2E+07  | 1.2E+07  | 1.2E+07  | 1.6E+07  | 1.6E+07  | 1.6E+07  | 1.6E+07  | 1.6E+07  |
| Z                   | 2.25E-4  | 2.25E-3  | 9.00E-3  | 2.25E-2  | 6.75E-2  | 2.25E-4  | 2.25E-3  | 9.00E-3  | 2.25E-2  | 6.75E-2  |
| Al26                | 1.29E-07 | 3.89E-07 | 5.25E-07 | 8.19E-07 | 1.32E-06 | 8.06E-08 | 2.01E-07 | 2.86E-07 | 3.97E-07 | 5.71E-07 |
| P 32                | 2.25E-10 | 2.97E-08 | 1.57E-07 | 5.68E-07 | 4.76E-06 | 1.40E-10 | 2.00E-08 | 1.05E-07 | 3.41E-07 | 2.57E-06 |
| P 33                | 8.13E-11 | 2.34E-08 | 1.49E-07 | 5.37E-07 | 3.73E-06 | 5.02E-11 | 1.38E-08 | 9.17E-08 | 3.13E-07 | 2.10E-06 |
| S 35                | 2.74E-11 | 6.40E-09 | 7.57E-08 | 7.14E-07 | 1.08E-05 | 1.58E-11 | 4.10E-09 | 4.96E-08 | 4.22E-07 | 5.93E-06 |
| Ar37                | 6.31E-06 | 1.08E-05 | 2.22E-05 | 3.74E-05 | 6.53E-05 | 4.11E-06 | 7.87E-06 | 1.65E-05 | 2.73E-05 | 4.77E-05 |
| Ca41                | 6.71E-07 | 1.72E-06 | 4.13E-06 | 7.20E-06 | 1.08E-05 | 5.64E-07 | 1.35E-06 | 3.19E-06 | 5.38E-06 | 7.94E-06 |
| Ti44                | 2.70E-05 | 2.47E-05 | 2.18E-05 | 1.78E-05 | 1.26E-05 | 3.15E-05 | 2.93E-05 | 2.64E-05 | 2.31E-05 | 1.72E-05 |
| V 48                | 4.16E-04 | 3.99E-04 | 3.52E-04 | 2.72E-04 | 1.83E-04 | 5.96E-04 | 5.78E-04 | 5.19E-04 | 4.54E-04 | 3.23E-04 |
| V 49                | 8.20E-06 | 1.15E-05 | 1.83E-05 | 2.35E-05 | 2.60E-05 | 7.21E-06 | 1.38E-05 | 2.18E-05 | 2.99E-05 | 3.68E-05 |
| Cr51                | 1.15E-05 | 2.04E-05 | 4.73E-05 | 7.76E-05 | 1.46E-04 | 1.40E-05 | 2.52E-05 | 5.85E-05 | 9.73E-05 | 1.77E-04 |
| Mn52                | 7.82E-03 | 7.58E-03 | 6.75E-03 | 5.30E-03 | 4.09E-03 | 1.40E-02 | 1.37E-02 | 1.21E-02 | 1.10E-02 | 8.52E-03 |
| Mn53                | 4.85E-04 | 5.93E-04 | 8.16E-04 | 9.91E-04 | 1.54E-03 | 5.68E-04 | 7.67E-04 | 1.07E-03 | 1.45E-03 | 2.18E-03 |
| Mn54                | 7.64E-06 | 7.70E-06 | 7.93E-06 | 8.38E-06 | 1.19E-05 | 7.43E-06 | 7.48E-06 | 7.78E-06 | 8.16E-06 | 1.12E-05 |
| Fe55                | 3.58E-03 | 4.73E-03 | 6.38E-03 | 7.94E-03 | 1.19E-02 | 3.88E-03 | 5.66E-03 | 8.17E-03 | 1.13E-02 | 1.76E-02 |
| Fe59                | 8.17E-07 | 1.04E-06 | 1.51E-06 | 2.59E-06 | 8.25E-06 | 8.29E-07 | 9.24E-07 | 1.19E-06 | 1.72E-06 | 4.40E-06 |
| Fe60                | 2.05E-06 | 2.50E-06 | 5.52E-06 | 1.52E-05 | 9.79E-05 | 2.08E-06 | 2.32E-06 | 3.89E-06 | 8.67E-06 | 4.99E-05 |
| Co56                | 6.80E-05 | 7.00E-05 | 7.21E-05 | 7.63E-05 | 9.65E-05 | 9.22E-05 | 9.67E-05 | 9.61E-05 | 1.06E-04 | 1.34E-04 |
| Co57                | 6.42E-04 | 6.45E-04 | 6.55E-04 | 6.85E-04 | 8.39E-04 | 6.34E-04 | 6.37E-04 | 6.46E-04 | 6.69E-04 | 8.09E-04 |
| Co58                | 3.71E-06 | 3.74E-06 | 3.81E-06 | 3.94E-06 | 4.62E-06 | 3.67E-06 | 3.70E-06 | 3.77E-06 | 3.91E-06 | 4.57E-06 |
| Co60                | 5.24E-07 | 7.63E-07 | 1.76E-06 | 3.27E-06 | 7.18E-06 | 5.10E-07 | 6.07E-07 | 1.04E-06 | 1.69E-06 | 4.05E-06 |
| Ni56                | 2.69E-01 | 2.66E-01 | 2.51E-01 | 2.14E-01 | 1.85E-01 | 4.91E-01 | 4.87E-01 | 4.43E-01 | 4.26E-01 | 3.68E-01 |
| Ni57                | 2.89E-03 | 3.28E-03 | 4.09E-03 | 4.80E-03 | 6.12E-03 | 3.53E-03 | 4.06E-03 | 5.23E-03 | 6.86E-03 | 9.60E-03 |
| Ni59                | 2.30E-04 | 2.20E-04 | 2.23E-04 | 2.20E-04 | 2.34E-04 | 2.49E-04 | 2.37E-04 | 2.42E-04 | 2.48E-04 | 2.67E-04 |
| Zn65                | 1.12E-08 | 4.61E-07 | 2.67E-06 | 2.71E-06 | 7.00E-07 | 9.15E-09 | 3.01E-07 | 1.61E-06 | 1.54E-06 | 4.19E-07 |

Table A3 continued.

|                     |          |          |          |          |          |          |          |          |          |          |
|---------------------|----------|----------|----------|----------|----------|----------|----------|----------|----------|----------|
| $\rho_{\text{DDT}}$ | 2.4E+07  | 2.4E+07  | 2.4E+07  | 2.4E+07  | 2.4E+07  | 2.8E+07  | 2.8E+07  | 2.8E+07  | 2.8E+07  | 2.8E+07  |
| Z                   | 2.25E-4  | 2.25E-3  | 9.00E-3  | 2.25E-2  | 6.75E-2  | 2.25E-4  | 2.25E-3  | 9.00E-3  | 2.25E-2  | 6.75E-2  |
| Al26                | 4.95E-08 | 1.00E-07 | 1.30E-07 | 1.69E-07 | 2.50E-07 | 7.68E-07 | 1.75E-07 | 9.68E-08 | 1.34E-07 | 1.86E-07 |
| P 32                | 8.30E-11 | 1.19E-08 | 5.71E-08 | 1.75E-07 | 1.31E-06 | 6.60E-11 | 9.78E-09 | 4.48E-08 | 1.46E-07 | 1.02E-06 |
| P 33                | 3.00E-11 | 7.50E-09 | 4.59E-08 | 1.53E-07 | 1.10E-06 | 2.55E-11 | 5.85E-09 | 3.38E-08 | 1.23E-07 | 8.41E-07 |
| S 35                | 1.07E-11 | 2.66E-09 | 2.82E-08 | 2.15E-07 | 3.01E-06 | 9.72E-12 | 2.21E-09 | 2.25E-08 | 1.78E-07 | 2.31E-06 |
| Ar37                | 3.01E-06 | 6.17E-06 | 1.26E-05 | 2.04E-05 | 3.68E-05 | 2.67E-06 | 5.67E-06 | 1.11E-05 | 1.88E-05 | 3.32E-05 |
| Ca41                | 4.97E-07 | 1.11E-06 | 2.52E-06 | 4.14E-06 | 6.33E-06 | 4.75E-07 | 1.05E-06 | 2.26E-06 | 3.86E-06 | 5.80E-06 |
| Ti44                | 3.03E-05 | 2.69E-05 | 2.39E-05 | 2.08E-05 | 1.49E-05 | 2.90E-05 | 2.92E-05 | 3.11E-05 | 2.38E-05 | 1.87E-05 |
| V 48                | 5.57E-04 | 5.36E-04 | 5.01E-04 | 4.14E-04 | 2.84E-04 | 4.81E-04 | 4.76E-04 | 4.34E-04 | 3.81E-04 | 2.59E-04 |
| V 49                | 5.70E-06 | 1.29E-05 | 2.05E-05 | 2.69E-05 | 3.27E-05 | 4.98E-06 | 1.16E-05 | 1.76E-05 | 2.45E-05 | 2.93E-05 |
| Cr51                | 1.46E-05 | 2.58E-05 | 5.88E-05 | 9.08E-05 | 1.57E-04 | 1.43E-05 | 2.40E-05 | 5.12E-05 | 8.36E-05 | 1.42E-04 |
| Mn52                | 1.56E-02 | 1.51E-02 | 1.45E-02 | 1.15E-02 | 8.40E-03 | 1.29E-02 | 1.26E-02 | 1.14E-02 | 1.04E-02 | 7.39E-03 |
| Mn53                | 5.69E-04 | 8.31E-04 | 1.22E-03 | 1.49E-03 | 2.12E-03 | 5.09E-04 | 7.45E-04 | 1.02E-03 | 1.38E-03 | 1.90E-03 |
| Mn54                | 7.25E-06 | 7.30E-06 | 7.49E-06 | 7.95E-06 | 1.03E-05 | 7.18E-06 | 7.33E-06 | 7.51E-06 | 7.74E-06 | 1.02E-05 |
| Fe55                | 3.86E-03 | 5.96E-03 | 9.65E-03 | 1.24E-02 | 1.98E-02 | 3.82E-03 | 5.49E-03 | 8.14E-03 | 1.15E-02 | 1.74E-02 |
| Fe59                | 8.29E-07 | 8.89E-07 | 1.08E-06 | 1.44E-06 | 3.22E-06 | 8.41E-07 | 8.97E-07 | 1.03E-06 | 1.36E-06 | 2.83E-06 |
| Fe60                | 2.03E-06 | 2.22E-06 | 3.16E-06 | 5.60E-06 | 2.70E-05 | 2.11E-06 | 2.22E-06 | 3.03E-06 | 5.43E-06 | 2.29E-05 |
| Co56                | 1.18E-04 | 1.24E-04 | 1.27E-04 | 1.33E-04 | 1.62E-04 | 1.25E-04 | 1.28E-04 | 1.32E-04 | 1.38E-04 | 1.59E-04 |
| Co57                | 6.29E-04 | 6.31E-04 | 6.41E-04 | 6.63E-04 | 7.79E-04 | 6.29E-04 | 6.32E-04 | 6.41E-04 | 6.61E-04 | 7.72E-04 |
| Co58                | 3.56E-06 | 3.58E-06 | 3.63E-06 | 3.77E-06 | 4.31E-06 | 3.52E-06 | 3.57E-06 | 3.63E-06 | 3.70E-06 | 4.25E-06 |
| Co60                | 5.02E-07 | 5.42E-07 | 6.86E-07 | 9.42E-07 | 2.18E-06 | 4.99E-07 | 5.36E-07 | 6.41E-07 | 8.46E-07 | 1.80E-06 |
| Ni56                | 7.16E-01 | 7.10E-01 | 6.85E-01 | 6.55E-01 | 5.46E-01 | 7.80E-01 | 7.67E-01 | 7.54E-01 | 7.07E-01 | 5.96E-01 |
| Ni57                | 4.51E-03 | 5.44E-03 | 7.15E-03 | 1.17E-02 | 1.68E-02 | 5.83E-03 | 8.06E-03 | 1.10E-02 | 1.42E-02 | 2.11E-02 |
| Ni59                | 3.12E-04 | 2.39E-04 | 2.40E-04 | 3.47E-04 | 2.80E-04 | 9.60E-04 | 2.60E-04 | 4.23E-04 | 5.08E-04 | 7.12E-04 |
| Zn65                | 7.46E-09 | 1.68E-07 | 7.07E-07 | 7.72E-07 | 2.61E-07 | 9.24E-08 | 5.34E-07 | 1.02E-06 | 9.71E-07 | 8.83E-07 |

Table A3 *continued*.

|                     |          |          |          |          |          |
|---------------------|----------|----------|----------|----------|----------|
| $\rho_{\text{DDT}}$ | 4.0E+07  | 4.0E+07  | 4.0E+07  | 4.0E+07  | 4.0E+07  |
| Z                   | 2.25E-4  | 2.25E-3  | 9.00E-3  | 2.25E-2  | 6.75E-2  |
| Al26                | 1.67E-06 | 1.61E-07 | 5.49E-08 | 6.99E-08 | 9.22E-08 |
| P 32                | 3.71E-11 | 5.87E-09 | 2.78E-08 | 8.26E-08 | 5.57E-07 |
| P 33                | 1.98E-11 | 3.07E-09 | 1.89E-08 | 6.56E-08 | 4.67E-07 |
| S 35                | 7.17E-12 | 1.32E-09 | 1.45E-08 | 1.09E-07 | 1.34E-06 |
| Ar37                | 1.87E-06 | 4.22E-06 | 8.53E-06 | 1.39E-05 | 2.50E-05 |
| Ca41                | 3.83E-07 | 8.23E-07 | 1.81E-06 | 2.97E-06 | 4.50E-06 |
| Ti44                | 3.54E-05 | 4.45E-05 | 4.65E-05 | 4.01E-05 | 2.40E-05 |
| V 48                | 3.78E-04 | 3.84E-04 | 3.63E-04 | 3.16E-04 | 2.11E-04 |
| V 49                | 3.93E-06 | 9.30E-06 | 1.42E-05 | 1.95E-05 | 2.34E-05 |
| Cr51                | 1.42E-05 | 2.13E-05 | 4.36E-05 | 6.87E-05 | 1.14E-04 |
| Mn52                | 9.80E-03 | 9.49E-03 | 8.94E-03 | 7.97E-03 | 5.76E-03 |
| Mn53                | 4.32E-04 | 6.45E-04 | 8.69E-04 | 1.13E-03 | 1.55E-03 |
| Mn54                | 7.17E-06 | 7.22E-06 | 7.47E-06 | 7.72E-06 | 9.75E-06 |
| Fe55                | 3.77E-03 | 5.01E-03 | 7.18E-03 | 9.77E-03 | 1.45E-02 |
| Fe59                | 8.56E-07 | 8.88E-07 | 9.91E-07 | 1.23E-06 | 2.32E-06 |
| Fe60                | 2.12E-06 | 2.25E-06 | 2.76E-06 | 4.38E-06 | 1.54E-05 |
| Co56                | 1.39E-04 | 1.43E-04 | 1.45E-04 | 1.49E-04 | 1.63E-04 |
| Co57                | 6.29E-04 | 6.33E-04 | 6.40E-04 | 6.62E-04 | 7.56E-04 |
| Co58                | 3.51E-06 | 3.52E-06 | 3.61E-06 | 3.68E-06 | 4.16E-06 |
| Co60                | 5.01E-07 | 5.18E-07 | 5.74E-07 | 6.77E-07 | 1.23E-06 |
| Ni56                | 8.96E-01 | 8.91E-01 | 8.59E-01 | 8.17E-01 | 6.88E-01 |
| Ni57                | 8.01E-03 | 1.18E-02 | 1.49E-02 | 1.95E-02 | 2.85E-02 |
| Ni59                | 1.59E-03 | 2.98E-04 | 6.30E-04 | 8.92E-04 | 1.25E-03 |
| Zn65                | 3.54E-07 | 1.58E-06 | 1.72E-06 | 2.05E-06 | 1.84E-06 |



Table A4. Radioactivities with half-life longer than one day in sub-Chandrasekhar models with the standard  $^{12}\text{C}+^{16}\text{O}$  reaction rate.

| $M_{\text{WD}}$ | 0.88     | 0.88     | 0.88     | 0.88     | 0.88     | 0.97     | 0.97     | 0.97     | 0.97     | 0.97     |
|-----------------|----------|----------|----------|----------|----------|----------|----------|----------|----------|----------|
| Z               | 2.25E-4  | 2.25E-3  | 9.00E-3  | 2.25E-2  | 6.75E-2  | 2.25E-4  | 2.25E-3  | 9.00E-3  | 2.25E-2  | 6.75E-2  |
| Z               | 2.25e-4  | 2.25e-3  | 9.00e-3  | 2.25e-2  | 6.75e-2  | 2.25e-4  | 2.25e-3  | 9.00e-3  | 2.25e-2  | 6.75e-2  |
| Al26            | 9.89E-08 | 2.81E-07 | 3.74E-07 | 5.25E-07 | 7.03E-07 | 5.46E-08 | 1.07E-07 | 1.40E-07 | 1.87E-07 | 2.30E-07 |
| P 32            | 1.68E-10 | 2.37E-08 | 1.23E-07 | 4.09E-07 | 2.91E-06 | 8.68E-11 | 1.24E-08 | 5.96E-08 | 1.84E-07 | 1.17E-06 |
| P 33            | 5.59E-11 | 1.87E-08 | 1.16E-07 | 3.90E-07 | 2.38E-06 | 2.93E-11 | 8.08E-09 | 4.81E-08 | 1.62E-07 | 9.77E-07 |
| S 35            | 1.93E-11 | 5.13E-09 | 5.74E-08 | 4.85E-07 | 6.31E-06 | 8.90E-12 | 2.83E-09 | 2.96E-08 | 2.27E-07 | 2.68E-06 |
| Ar37            | 4.82E-06 | 8.15E-06 | 1.69E-05 | 2.76E-05 | 4.56E-05 | 3.37E-06 | 6.63E-06 | 1.32E-05 | 2.16E-05 | 3.59E-05 |
| Ca41            | 4.95E-07 | 1.31E-06 | 3.16E-06 | 5.30E-06 | 7.52E-06 | 5.09E-07 | 1.19E-06 | 2.62E-06 | 4.35E-06 | 6.19E-06 |
| Ti44            | 1.85E-05 | 1.66E-05 | 1.47E-05 | 1.27E-05 | 9.67E-06 | 2.27E-05 | 2.05E-05 | 1.82E-05 | 1.58E-05 | 1.15E-05 |
| V 48            | 2.88E-04 | 2.72E-04 | 2.43E-04 | 2.09E-04 | 1.60E-04 | 4.08E-04 | 3.93E-04 | 3.59E-04 | 3.10E-04 | 2.08E-04 |
| V 49            | 5.01E-06 | 7.08E-06 | 1.16E-05 | 1.58E-05 | 1.97E-05 | 6.17E-06 | 9.12E-06 | 1.47E-05 | 2.02E-05 | 2.39E-05 |
| Cr51            | 2.21E-06 | 1.06E-05 | 2.92E-05 | 5.12E-05 | 1.07E-04 | 2.13E-06 | 1.40E-05 | 3.76E-05 | 6.48E-05 | 1.17E-04 |
| Mn52            | 5.84E-03 | 5.58E-03 | 5.10E-03 | 4.58E-03 | 3.96E-03 | 1.06E-02 | 1.03E-02 | 9.49E-03 | 8.36E-03 | 5.97E-03 |
| Mn53            | 1.69E-04 | 2.41E-04 | 4.04E-04 | 5.77E-04 | 1.08E-03 | 2.87E-04 | 3.97E-04 | 6.50E-04 | 9.25E-04 | 1.39E-03 |
| Mn54            | 7.29E-11 | 4.04E-09 | 4.03E-08 | 2.33E-07 | 2.02E-06 | 3.01E-11 | 2.77E-09 | 2.45E-08 | 1.39E-07 | 1.55E-06 |
| Fe55            | 1.79E-04 | 1.00E-03 | 2.23E-03 | 3.65E-03 | 7.16E-03 | 1.93E-04 | 1.66E-03 | 3.89E-03 | 6.44E-03 | 1.11E-02 |
| Fe59            | 6.78E-10 | 1.59E-07 | 4.80E-07 | 1.11E-06 | 3.75E-06 | 3.29E-10 | 5.63E-08 | 1.68E-07 | 4.22E-07 | 1.51E-06 |
| Fe60            | 9.16E-11 | 2.83E-07 | 2.30E-06 | 7.95E-06 | 5.29E-05 | 4.94E-11 | 1.14E-07 | 8.59E-07 | 2.95E-06 | 1.88E-05 |
| Co56            | 1.73E-05 | 1.76E-05 | 1.93E-05 | 2.49E-05 | 4.22E-05 | 4.79E-05 | 4.98E-05 | 5.20E-05 | 5.82E-05 | 7.86E-05 |
| Co57            | 2.99E-07 | 7.07E-07 | 2.89E-06 | 1.13E-05 | 9.39E-05 | 7.96E-07 | 1.40E-06 | 3.78E-06 | 1.16E-05 | 8.19E-05 |
| Co58            | 5.92E-09 | 1.28E-08 | 2.72E-08 | 6.68E-08 | 3.56E-07 | 1.90E-09 | 4.08E-09 | 1.24E-08 | 3.85E-08 | 2.59E-07 |
| Co60            | 7.22E-10 | 1.65E-07 | 8.26E-07 | 1.72E-06 | 3.89E-06 | 3.12E-10 | 5.11E-08 | 2.25E-07 | 4.92E-07 | 1.42E-06 |
| Ni56            | 1.50E-01 | 1.45E-01 | 1.38E-01 | 1.33E-01 | 1.33E-01 | 4.27E-01 | 4.21E-01 | 4.10E-01 | 3.95E-01 | 3.58E-01 |
| Ni57            | 4.36E-04 | 6.34E-04 | 1.11E-03 | 1.69E-03 | 2.94E-03 | 1.53E-03 | 2.23E-03 | 3.64E-03 | 5.72E-03 | 1.06E-02 |
| Ni59            | 4.25E-07 | 1.40E-06 | 1.37E-06 | 3.57E-06 | 1.81E-05 | 8.55E-05 | 1.10E-05 | 2.68E-05 | 5.25E-05 | 1.40E-04 |
| Zn65            | 5.39E-09 | 3.47E-07 | 1.83E-06 | 1.72E-06 | 4.18E-07 | 8.77E-09 | 1.79E-07 | 7.55E-07 | 7.25E-07 | 2.67E-07 |

Table A4 *continued.*

| $M_{\text{WD}}$ | 1.06     | 1.06     | 1.06     | 1.06     | 1.06     | 1.10     | 1.10     | 1.10     | 1.10     | 1.10     |
|-----------------|----------|----------|----------|----------|----------|----------|----------|----------|----------|----------|
| Z               | 2.25E-4  | 2.25E-3  | 9.00E-3  | 2.25E-2  | 6.75E-2  | 2.25E-4  | 2.25E-3  | 9.00E-3  | 2.25E-2  | 6.75E-2  |
| Al26            | 1.43E-06 | 4.78E-08 | 5.27E-08 | 6.70E-08 | 7.59E-08 | 1.51E-06 | 5.62E-08 | 3.27E-08 | 4.10E-08 | 4.55E-08 |
| P 32            | 4.20E-11 | 5.77E-09 | 2.58E-08 | 7.57E-08 | 4.34E-07 | 2.85E-11 | 3.80E-09 | 1.65E-08 | 4.75E-08 | 2.64E-07 |
| P 33            | 1.60E-11 | 3.05E-09 | 1.75E-08 | 5.91E-08 | 3.56E-07 | 1.19E-11 | 1.82E-09 | 1.03E-08 | 3.50E-08 | 2.12E-07 |
| S 35            | 4.30E-12 | 1.35E-09 | 1.41E-08 | 1.02E-07 | 1.06E-06 | 3.19E-12 | 9.21E-10 | 9.79E-09 | 6.89E-08 | 6.77E-07 |
| Ar37            | 2.07E-06 | 4.59E-06 | 8.96E-06 | 1.44E-05 | 2.37E-05 | 1.53E-06 | 3.58E-06 | 6.94E-06 | 1.11E-05 | 1.81E-05 |
| Ca41            | 4.04E-07 | 9.02E-07 | 1.89E-06 | 3.05E-06 | 4.24E-06 | 3.37E-07 | 7.34E-07 | 1.52E-06 | 2.42E-06 | 3.29E-06 |
| Ti44            | 2.68E-05 | 2.44E-05 | 2.49E-05 | 2.04E-05 | 1.15E-05 | 2.68E-05 | 2.49E-05 | 2.58E-05 | 2.08E-05 | 1.10E-05 |
| V 48            | 3.41E-04 | 3.33E-04 | 3.07E-04 | 2.64E-04 | 1.72E-04 | 3.01E-04 | 2.96E-04 | 2.73E-04 | 2.35E-04 | 1.51E-04 |
| V 49            | 3.71E-06 | 7.73E-06 | 1.22E-05 | 1.68E-05 | 1.98E-05 | 2.81E-06 | 6.91E-06 | 1.08E-05 | 1.48E-05 | 1.75E-05 |
| Cr51            | 3.14E-06 | 1.14E-05 | 3.12E-05 | 5.37E-05 | 9.31E-05 | 3.43E-06 | 9.95E-06 | 2.74E-05 | 4.72E-05 | 8.13E-05 |
| Mn52            | 8.67E-03 | 8.43E-03 | 7.79E-03 | 6.85E-03 | 4.78E-03 | 7.54E-03 | 7.33E-03 | 6.78E-03 | 5.97E-03 | 4.28E-03 |
| Mn53            | 2.07E-04 | 3.36E-04 | 5.38E-04 | 7.64E-04 | 1.11E-03 | 1.60E-04 | 2.98E-04 | 4.72E-04 | 6.72E-04 | 1.00E-03 |
| Mn54            | 1.53E-11 | 1.50E-09 | 1.36E-08 | 7.88E-08 | 1.05E-06 | 1.07E-11 | 1.07E-09 | 1.01E-08 | 5.91E-08 | 8.24E-07 |
| Fe55            | 1.01E-04 | 1.32E-03 | 3.21E-03 | 5.34E-03 | 9.00E-03 | 9.49E-05 | 1.14E-03 | 2.80E-03 | 4.86E-03 | 9.20E-03 |
| Fe59            | 1.45E-10 | 2.04E-08 | 6.09E-08 | 1.59E-07 | 6.09E-07 | 9.56E-11 | 1.24E-08 | 3.81E-08 | 1.01E-07 | 3.89E-07 |
| Fe60            | 2.38E-11 | 4.79E-08 | 3.55E-07 | 1.20E-06 | 6.79E-06 | 1.57E-11 | 3.07E-08 | 2.33E-07 | 7.93E-07 | 4.27E-06 |
| Co56            | 7.72E-05 | 8.01E-05 | 8.19E-05 | 8.58E-05 | 9.84E-05 | 9.10E-05 | 9.38E-05 | 9.54E-05 | 9.90E-05 | 1.13E-04 |
| Co57            | 2.48E-06 | 4.04E-06 | 6.53E-06 | 1.34E-05 | 6.65E-05 | 3.48E-06 | 5.26E-06 | 7.80E-06 | 1.42E-05 | 5.94E-05 |
| Co58            | 7.07E-10 | 1.53E-09 | 5.99E-09 | 2.21E-08 | 1.70E-07 | 4.48E-10 | 9.81E-10 | 4.22E-09 | 1.68E-08 | 1.34E-07 |
| Co60            | 1.40E-10 | 1.91E-08 | 6.66E-08 | 1.46E-07 | 4.68E-07 | 9.28E-11 | 1.24E-08 | 4.04E-08 | 8.59E-08 | 2.75E-07 |
| Ni56            | 6.85E-01 | 6.79E-01 | 6.64E-01 | 6.38E-01 | 5.65E-01 | 7.91E-01 | 7.85E-01 | 7.69E-01 | 7.39E-01 | 6.50E-01 |
| Ni57            | 4.94E-03 | 7.62E-03 | 1.01E-02 | 1.41E-02 | 2.31E-02 | 6.86E-03 | 1.00E-02 | 1.30E-02 | 1.78E-02 | 2.79E-02 |
| Ni59            | 7.34E-04 | 8.84E-05 | 2.96E-04 | 4.74E-04 | 6.62E-04 | 9.07E-04 | 1.30E-04 | 4.03E-04 | 6.14E-04 | 8.12E-04 |
| Zn65            | 2.89E-07 | 5.34E-07 | 8.48E-07 | 9.15E-07 | 5.03E-07 | 3.71E-07 | 6.61E-07 | 9.20E-07 | 9.97E-07 | 5.66E-07 |

Table A4 *continued.*

| $M_{\text{WD}}$ | 1.15     | 1.15     | 1.15     | 1.15     | 1.15     |
|-----------------|----------|----------|----------|----------|----------|
| Z               | 2.25E-4  | 2.25E-3  | 9.00E-3  | 2.25E-2  | 6.75E-2  |
| Al26            | 1.19E-06 | 1.40E-07 | 1.74E-08 | 2.16E-08 | 2.32E-08 |
| P 32            | 1.62E-11 | 2.03E-09 | 8.59E-09 | 2.46E-08 | 1.36E-07 |
| P 33            | 8.00E-12 | 8.59E-10 | 4.94E-09 | 1.71E-08 | 1.05E-07 |
| S 35            | 2.17E-12 | 5.35E-10 | 5.87E-09 | 4.06E-08 | 3.73E-07 |
| Ar37            | 9.58E-07 | 2.41E-06 | 4.59E-06 | 7.32E-06 | 1.17E-05 |
| Ca41            | 2.51E-07 | 5.14E-07 | 1.04E-06 | 1.65E-06 | 2.21E-06 |
| Ti44            | 2.51E-05 | 2.42E-05 | 2.55E-05 | 2.03E-05 | 1.03E-05 |
| V 48            | 2.46E-04 | 2.45E-04 | 2.27E-04 | 1.95E-04 | 1.27E-04 |
| V 49            | 2.06E-06 | 5.79E-06 | 8.85E-06 | 1.22E-05 | 1.49E-05 |
| Cr51            | 3.30E-06 | 8.00E-06 | 2.24E-05 | 3.90E-05 | 6.90E-05 |
| Mn52            | 6.07E-03 | 5.90E-03 | 5.50E-03 | 5.01E-03 | 3.99E-03 |
| Mn53            | 1.05E-04 | 2.48E-04 | 3.90E-04 | 5.88E-04 | 9.69E-04 |
| Mn54            | 6.33E-12 | 6.18E-10 | 6.39E-09 | 3.81E-08 | 5.23E-07 |
| Fe55            | 9.45E-05 | 8.96E-04 | 2.43E-03 | 5.37E-03 | 1.15E-02 |
| Fe59            | 5.56E-11 | 6.64E-09 | 2.12E-08 | 5.67E-08 | 2.15E-07 |
| Fe60            | 9.39E-12 | 1.67E-08 | 1.31E-07 | 4.57E-07 | 2.31E-06 |
| Co56            | 1.09E-04 | 1.12E-04 | 1.14E-04 | 1.20E-04 | 1.40E-04 |
| Co57            | 4.75E-06 | 6.69E-06 | 9.31E-06 | 1.50E-05 | 4.81E-05 |
| Co58            | 2.35E-10 | 5.34E-10 | 2.62E-09 | 1.10E-08 | 8.78E-08 |
| Co60            | 5.27E-11 | 6.68E-09 | 2.12E-08 | 4.33E-08 | 1.36E-07 |
| Ni56            | 9.18E-01 | 9.13E-01 | 8.94E-01 | 8.59E-01 | 7.51E-01 |
| Ni57            | 9.19E-03 | 1.27E-02 | 1.64E-02 | 2.17E-02 | 3.23E-02 |
| Ni59            | 1.06E-03 | 1.66E-04 | 4.49E-04 | 6.51E-04 | 8.86E-04 |
| Zn65            | 3.77E-07 | 7.45E-07 | 9.58E-07 | 1.04E-06 | 6.41E-07 |
